# Supplementary material for: Minimal Session Types for the $\pi$-calculus (Extended Version)
Source: arXiv:2107.10936 source file (2024-01-22)
Supplement: Supplementary file 1 [file appendix-mst-pi-examples.tex]

\providecommand{\thesisalt}[2]{\ifx\thesis\undefined#1\else#2\fi}

 \newpage
\section{Additional Examples}

\subsection{First Decomposition: Core Fragment}
\label{pi:app:ss:amcore}

\begin{example}[Core Fragment]
  \label{pi:ex:ex1-decomp}
  % Let $P$ be a \sessp process which incorporates name-passing and $w$ be a
  % channel through which first an integer value, then a boolean value is sent. 
  Let $P$ be a \sessp process which incorporates name-passing 
  and implements channels $u$ and $\dual w$ with types 
    $S = \btout{\dual T}\tinact$ 
  and $T = \btinp{\mathsf{Int}}\btout{\mathsf{Bool}}\tinact$, respectively:
  % The degree of $P$ is $\lenHO{P} = 25$.
  \begin{align*}
    P &= \news{u:S}(\bout{u}{w} \binp{\dual w}{t} \bout{\dual w}{\unaryint{t}} \inact \Par
      \binp{\dual u}{x} \bout{x}{\textsf{5}}\binp{x}{b} \inact) = \news{u}(A \Par B)	
  \end{align*}
  
  \noindent 
  The degree of $P$ is $\lenHO{P} = 25$.
  Then, the decomposition of $P$ into a collection of first-order processes
  typed with minimal session types is:
  \begin{align*}
    \F{P} &= \news{ \prop_1, \dots, c_{25}}\big(\propout{1}{} \inact \Par 
              \AmeliaMod{1}{\epsilon}{P\sigma}_\empg \big)\\
          &= \news{ \prop_1, \dots, c_{25}}\big(\propout{1}{} \inact \Par 
          \AmeliaMod{1}{\epsilon}{\news{u}(A \Par B)\sigma}_\empg \big)\\
          &= \news{ \prop_1, \dots, c_{25}}\big(\propout{1}{} \inact 
          \Par \news{u_1} \AmeliaMod{1}{\epsilon}{(A \Par B)\sigma'}_\empg \big), \\
          &\text{ where } \sigma = \mathsf{init}(\fn{P}),\ 
          \sigma' = \sigma \cdot \subst{u_1 \dual{u_1}}{u\dual{u}}
  \end{align*}

  \noindent We have:
  \begin{align*}
      \AmeliaMod{1}{\epsilon}{(A \Par B)\sigma'}_\empg \big) &= 
      \propinp{1}{} \propout{2}{}  \apropout{13}{}  \Par 
      \AmeliaMod{2}{\epsilon}{A \sigma'}_\empg \Par \AmeliaMod{13}{\epsilon}{B \sigma'}_\empg
  \end{align*}

  \noindent We use some abbreviations for 
  subprocesses of $A$ and $B$ : 
  \begin{align*}
    A' &= \binp{\dual{w}_1}{t}A''   
    \qquad A'' = \bout{\dual w_1}
    {\unaryint{t}}\inact  \\
    B' &= \bout{x_1}{5} B''  
    \qquad B'' = \binp{x_1}{b}\inact 
  \end{align*}

  \noindent The breakdown of $A$ is:
  \begin{align*}
  % A
  \AmeliaMod{2}{\epsilon}{A}_\empg &= \propinp{2}{} \news{a_1}\big(\bout{u_1}{a_1} \big( 
      \apropout{5}{} \Par \AmeliaMod{5}{\epsilon}{A'}_\empg 
      \Par \binp{a_1}{y_1} \binp{y_1}{z_1} \apropout{3}{z_1} \Par \\
      & \quad \propinp{3}{z_1} \binp{z_1}{x} \apropout{4}{x} \Par 
      \propinp{4}{x} \news{s} \big(\bout{x}{s} \about{\dual s}{w_1, w_2}\big) \big) \big)\\
  % next row
  \AmeliaMod{5}{\epsilon}{A'}_\empg &= 
  \propinp{5}{} \binp{\dual{w_1}}{y_2} \apropout{6}{y_2} \Par 
  \news{s_1} \big( \propinp{6}{y_2} \propout{7}{y_2} \apropbout{8}{} \Par \\
      & \quad \propinp{7}{y_2} \news{s'}\big( \bout{y_2}{s'}  \bout{\dual{s'}}{s_1} \inact \big) \big) 
      \Par \propinp{8}{} \news{a_2} \big( \bout{\dual{s_1}}{a_2} \big(\apropout{10}{} 
      \Par \propinp{10}{} \inact \Par \\
      & \quad \binp{a_2}{y_3} \binp{y_3}{t_1} 
      \big( \apropout{9}{} \Par
      \AmeliaMod{9}{\epsilon}{A''}_\empg  \big) \big) \big)  \\
      %  third row
       \AmeliaMod{9}{\epsilon}{A''}_\empg &= 
    \propinp{9}{} \news{a} \big(\bout{\dual w_2}{a}
    \big( \apropout{12}{} \Par \propinp{12}{}\inact \Par 
     \\
     & \qquad \binp{a}{y} \binp{y}{z_1} \apropout{11}{z_1} \Par
     \propinp{10}{z_1} \binp{z_1}{x} \apropout{11}{x} \Par
    %  \\
    %  &
    %  \qquad \qquad \qquad \qquad 
     \propinp{11}{x} 
     \news{s} \big(\bout{x}{s} \about{ \dual{s} }{\unaryint{t}}\big) \big) \big)
  \end{align*}

  % \begin{align*}
  %   \AmeliaMod{9}{\epsilon}{\bout{\dual w_2}{\textsf{true}}\inact }_g &= 
  %   \propinp{9}{} \news{a} \big(\bout{\dual w_2}{a}
  %   ( \apropout{12}{} \Par \propinp{12}{}\inact \Par 
  %    \\
  %    & \qquad \binp{a}{y} \binp{y}{z_1} \apropout{11}{z_1} \Par
  %    \propinp{10}{z_1} \binp{z_1}{x} \apropout{11}{x} \Par
  %    \\
  %    &\qquad \qquad \qquad \qquad \propinp{11}{x} 
  %    \news{s} (\bout{x}{s} \about{ \dual{s} }{\textsf{true}}) ) \big)
  % \end{align*}
  
  \noindent The breakdown of $B$ is:
  \begin{align*}
    \AmeliaMod{13}{\epsilon}{B}_\empg &= 
    \propinp{13}{}\binp{\dual u_1}{y_4}\apropout{14}{y_4}  \Par 
    \news{s_1}\big( \propinp{14}{y}\propout{15}{y}\apropout{16}{} 
    \Par \\
    & \quad \propinp{15}{y_4} \news{s''} \big(\bout{y_4}{s''} 
      \bout{\dual{s''}}{s_1} \inact \big) \Par 
      \propinp{16}{} \news{a_3} \big(\bout{s_1}{a_3} \big( \apropout{21}{} \Par \\
    & \quad \propinp{21}{} \inact \Par 
    \binp{a_3}{y_5} \binp{y_5}{x_1, x_2} 
    \big(\apropout{17}{} \Par \AmeliaMod{17}{\epsilon}{B'}_\empg \big) \big) \big) \big) 
    \smallskip \bigskip \\
    % new row
  \AmeliaMod{17}{\epsilon}{B'}_\empg &=  
      \propinp{17}{} \news{a_4} \big( \bout{x_1}{a_4} \big( \apropout{20}{}  
      \Par \AmeliaMod{20}{\epsilon}{B''}_\empg  
      \Par \binp{a_4}{y_6} \binp{y_6}{z_1} 
      \apropout{18}{z_1} \Par \\
      & \quad \propinp{18}{z_1} \binp{z_1}{x} \apropout{19}{x} \Par 
      \propinp{19}{x} \news{s'''} \big(\bout{x}{s'''} \about{\dual{s'''}}{\textsf{5} } \big) \big) \big)
      \\
      % new row 
      \AmeliaMod{20}{\epsilon}{B''}_\empg &= 
      \propinp{20}{}\binp{x_2}{y} \apropout{21}{y} \Par
      \\
      &\qquad \news{s_1} \big(\propinp{21}{y} \propout{22}{y} \apropout{23}{} \Par
       \propinp{22}{y} \news{s}\big(\bout{y}{s} \about{\dual{s}}{s_1}   \big) \Par
      \\
      &\qquad \qquad \qquad \propinp{23}{\wtd x} \news{a}  \big(\bout{\dual{s_1}}{a} 
      \big( \apropout{25}{} \Par \propinp{25}{} \inact \Par \\
      & \qquad \qquad \qquad \binp{a}{y'} \binp{y'}
        {b_1} \big( \apropout{24}{} \Par
        \propinp{24}{}\inact \big)   \big) \big) \big) 
  \end{align*}

% \begin{align*}
%   \AmeliaMod{20}{\epsilon}{\binp{x_2}{b} \inact}_\empg &= 
%   \propinp{20}{}\binp{x_2}{y} \apropout{21}{y} \Par
%   \\
%   &\qquad \news{s_1} \big(\propinp{21}{y} \propout{22}{y} \apropout{23}{} \Par
%    \propinp{22}{y} \news{s}(\bout{y}{s} \about{\dual{s}}{s_1}   ) \Par
%   \\
%   &\qquad \qquad \qquad \propinp{23}{\wtd x} \news{a}  (\bout{\dual{s_1}}{a} 
%   ( \apropout{25}{} \Par \propinp{25}{} \inact \Par \\
%   & \qquad \qquad \qquad \binp{a}{y'} \binp{y'}
%     {b_1} \big( \apropout{24}{} \Par
%     \propinp{24}{}\inact \big)   ) ) \big) 
%   % &\text{where}
%   % \\
%   %   \widehat{Q}_{\tilde{x}} &= \binp{a}{y'} \binp{y'}
%   %   {b_1} \big( \apropout{k+4}{} \Par
%   %   \AmeliaMod{k+4}{}{Q \subst{w_1}{w} \sigma }_\empg \big) 
% \end{align*}
  \noindent Names $\dual w_1$ and $\dual w_2$ are typed, respectively, with 
  \begin{align*}
  M_1 & = \bbtinp{ \lrangle{ \btinp{ \btinp{ \lrangle{ \btinp{ \textsf{Int} }{\tinact} } }{\tinact} }{\tinact} } }{\tinact}
  \\
  M_2 & = \bbtout{ \lrangle{ \btinp{ \btinp{ \lrangle{ \btinp{ \textsf{Bool}}{\tinact} } }{\tinact} }{\tinact} } }{\tinact}
    \end{align*}
    Name $u_1$ is typed with 
  $\bbtout{ \lrangle{ \btinp{ \btinp{ \lrangle{ \btinp{ \dual M_1, \dual M_2 }{\tinact} } }{\tinact} }{\tinact} } }{\tinact}$. 
  Now let us observe the reduction chain. The collection of processes
  synchronizes on $\prop_1, \prop_2, \prop_{13}$ after three reductions.
  \begin{align*}
    \F{P} &\red^{3} \news{\widetilde c} \big( \ \news{a_1} \big( \highlighta{\bout{u_1}{a_1}} \big( 
      \apropout{5}{} \Par 
      \AmeliaMod{5}{\epsilon}{A' }_\empg \Par
      % \\
      % & \quad  
      \binp{a_1}{y_1} \binp{y_1}{z_1} \apropout{3}{z_1} \Par 
       \propinp{3}{z_1} \binp{z_1}{x} \apropout{4}{x} \Par 
       \\
      & \quad
      \propinp{4}{x} \news{s} \big(\bout{x}{s} \about{\dual s}{w_1, w_2}\big) \big) \big) \Par 
     \highlighta{\binp{\dual u_1}{y_4}}\apropout{14}{y_4}    \Par 
    %  \\
    %   & \quad 
    \news{s_1}\big( \propinp{14}{y}\propout{15}{y}\apropout{16}{} 
    \Par  
    \\
    & \qquad 
    \propinp{15}{y_4} \news{s''} \big(\bout{y_4}{s''} 
      \bout{\dual{s''}}{s_1} \inact \big) \Par 
    %   \\
    % & \qquad
      \propinp{16}{} \news{a_3} \big(\bout{s_1}{a_3} \big( \apropout{21}{} \Par \\
    & \qquad \quad \propinp{21}{} \inact \Par 
    \binp{a_3}{y_5} \binp{y_5}{x_1, x_2} 
    \big(\apropout{17}{} \Par 
    \AmeliaMod{17}{\epsilon}{B'}_\empg \big) \big) \big) \big)
    \smallskip \bigskip  
      \\ \bigskip & \quad \quad 
      \text{where $\widetilde c = (\prop_3, \dots, \prop_{12}, \prop_{14}, \dots, c_{25})$}
  \end{align*}
  
  \noindent Then, the broken down process $A$ communicates with process $B$
  through channel $u_1$ by passing name $a_1$ (highlighted above).
  % which is
  % further sent on $\prop_{14}$
  % and $\prop_{15}$. 
  Here we notice that the original transmission of value $w$ 
  is not immediately mimicked on channel $u$, but it is delegated to 
  some other channel through series of channel redirections 
  starting with the transmission of name $a_1$. 
  % Further, by breaking down sequential prefixes involved in channel redirections 
  % redundant communications on propagators are introduced. 
  Further,  received name $a_1$ is locally propagated by $\prop_{14}$
  and $\prop_{15}$. This represents redundant communications on propagators 
  induced by breaking down sequential prefixes produced by 
  two encodings $\map{\cdot}^1_g$ and $\map{\cdot}^{2}$
  (not present in the original process). 
  Another synchronization occurs on $\prop_{16}$.
  \begin{align*}
    \F{P} &\red^{7} \news{\widetilde c_*}\news{a_1} \big( \  
    \apropout{5}{} \Par  
    \AmeliaMod{5}{\epsilon}{A'}_\empg  \Par 
    \highlighta{\binp{a_1}{y_1}} \binp{y_1}{z_1} \apropout{3}{z_1}
     \Par 
    %  \\
    % & 
     \propinp{3}{z_1} \binp{z_1}{x} \apropout{4}{x} \Par 
     \\
     &   
     \propinp{4}{x} \news{s} \big(\bout{x}{s} \about{\dual s}{w_1, w_2} \big) 
    \Par 
    % \\
    % &
    \news{s_1}\big(  \news{s''} \big(\highlighta{\bout{a_1}{s''}} 
    \bout{\dual{s''}}{s_1} \inact \big) \Par 
     \news{a_3} \big(\bout{s_1}{a_3} \big( \apropout{21}{} \Par 
    \\
    & 
    \qquad 
    \propinp{21}{} \inact \Par 
    \binp{a_3}{y_5} \binp{y_5}{x_1, x_2} \big(\apropout{17}{} 
    \Par \AmeliaMod{17}{\epsilon}{B'}_\empg \big) \big) \big) \big)  \big) \smallskip 
    \\ \bigskip & \quad \quad \text{where 
    $\widetilde c_* = (\prop_3, \dots, c_{12}, c_{17}, \dots, c_{25})$}
\end{align*}

  % \begin{align*}
  %     \F{P} &\red^{7} \news{\widetilde c_*}\news{a_1} ( \  
  %     \apropout{5}{} \Par  
  %     \AmeliaMod{5}{\epsilon}{A' }_\empg  \Par 
  %     \highlighta{\binp{a_1}{y_1}} \binp{y_1}{z_1} \apropout{3}{z_1} \Par \propinp{3}{z_1} \binp{z_1}{x} \apropout{4}{x} \Par \\
  %     & \quad \propinp{4}{x} \news{s} (\bout{x}{s} \about{\dual s}{w_1, w_2}) 
  %     \Par \news{s_1}\big(  \news{s''} (\highlighta{\bout{a_1}{s''}} \bout{\dual{s''}}{s_1} \inact) \Par \\
  %     & \quad  \news{a_3} (\bout{s_1}{a_3} \big( \apropout{21}{} \Par 
  %     \propinp{21}{} \inact \Par \binp{a_3}{y_5} \binp{y_5}{x_1, x_2} (\apropout{17}{} 
  %     \Par \AmeliaMod{17}{\epsilon}{B'}_\empg ) \big) ) \big) \ ) \smallskip 
  %     \\ \bigskip & \quad \quad \text{where 
  %     $\widetilde c_* = (\prop_3, \dots, c_{12}, c_{17}, \dots, c_{25})$}
  % \end{align*}

  \noindent 
  The next step involves communication on $a_1$: session name $s''$ is passed and substitutes variable $y_1$.
  \begin{align*}
    \F{P} &\red^{8} \news{\widetilde c_*} \news{s''} \big( \ 
    \apropout{5}{} \Par 
    \AmeliaMod{5}{\epsilon}{A'}_\empg       \Par 
    % \\
    % &
    \highlighta{ \binp{s''}{z_1}} \apropout{3}{z_1} \Par \propinp{3}{z_1} \binp{z_1}{x} \apropout{4}{x} \Par 
    \\
    &  
    \propinp{4}{x} \news{s} \big(\bout{x}{s} \about{\dual s}{w_1, w_2} \big) 
    \Par 
    % \\
    % &
 \news{s_1}\big(  \highlighta{\bout{\dual{s''}}{s_1}} \inact \Par 
    \news{a_3} \big(\bout{s_1}{a_3} \big( \apropout{21}{} \Par \propinp{21}{} \inact \Par \\
    & \quad \binp{a_3}{y_5} \binp{y_5}{x_1, x_2} \big( \ \apropout{17}{} \Par 
    \AmeliaMod{17}{\epsilon}{B' }_\empg  \big) \big) \big) \big) \big) \smallskip 
 %   \\ \bigskip & \quad \quad 
 %   \text{where $\wtd \prop = (\prop_3, \dots, \prop_{12}, \prop_{17}, \dots, \prop_{25})$}
\end{align*}

  % \begin{align*}
  %     \F{P} &\red^{8} \news{\widetilde c_*} \news{s''} ( \ 
  %     \apropout{5}{} \Par 
  %     \AmeliaMod{5}{\epsilon}{A'}_\empg \Par 
  %     \highlighta{ \binp{s''}{z_1}} \apropout{3}{z_1} \Par \propinp{3}{z_1} \binp{z_1}{x} \apropout{4}{x} \Par \\
  %     & \quad \propinp{4}{x} \news{s} (\bout{x}{s} \about{\dual s}{w_1, w_2}) 
  %     \Par \news{s_1}\big(  \highlighta{\bout{\dual{s''}}{s_1}} \inact \Par 
  %     \news{a_3} (\bout{s_1}{a_3} \big( \apropout{21}{} \Par \propinp{21}{} \inact \Par \\
  %     & \quad \binp{a_3}{y_5} \binp{y_5}{x_1, x_2} ( \ \apropout{17}{} \Par 
  %     \AmeliaMod{17}{\epsilon}{B' }_\empg \  ) \big) ) \big) \ ) \smallskip 
  %     % \\ \bigskip & \quad \quad 
  %     % \text{where $\wtd \prop = (\prop_3, \dots, \prop_{12}, \prop_{17}, \dots, \prop_{25})$}
  % \end{align*}

  \noindent 
  The process then synchronizes on channel $s''$. After $z_1$ is replaced by
  $s_1$, it is further sent to the next parallel process through the propagator
  $c_3$.
  \begin{align*}
    \F{P} &\red^{10} \news{\widetilde c_{**}} \news{s_1} \big( \ 
    \apropout{5}{} \Par
     \AmeliaMod{5}{\epsilon}{A' }_\empg 
    \Par 
    % \\
    % &
    \highlighta{\binp{s_1}{x}} \apropout{4}{x} \Par \propinp{4}{x} 
    \news{s} \big(\bout{x}{s} \about{\dual s}{w_1, w_2}\big)  \Par \\
    & \news{a_3} \big(\highlighta{\bout{s_1}{a_3}} \big( \apropout{21}{} 
    \Par \propinp{21}{} \inact \Par  
    \\
    & 
    \qquad 
    \binp{a_3}{y_5} \binp{y_5}{x_1, x_2} 
    \big(\apropout{17}{} \Par 
    \AmeliaMod{17}{\epsilon}{B'}_\empg \big) \big) \big)  \big)\smallskip 
    \\ \bigskip & \quad \quad \text{where 
    $\widetilde c_{**} = (\prop_4, \dots, \prop_{12}, \prop_{17}, \dots, \prop_{25})$}
\end{align*}

  % \begin{align*}
  %     \F{P} &\red^{10} \news{\widetilde c_{**}} \news{s_1} ( \ 
  %     \apropout{5}{} \Par
  %      \AmeliaMod{5}{\epsilon}{A'}_\empg 
  %     \Par 
  %     \highlighta{\binp{s_1}{x}} \apropout{4}{x} \Par \propinp{4}{x} 
  %     \news{s} (\bout{x}{s} \about{\dual s}{w_1, w_2})  \Par \\
  %     & \quad \news{a_3} (\highlighta{\bout{s_1}{a_3}} \big( \apropout{21}{} 
  %     \Par \propinp{21}{} \inact \Par  \binp{a_3}{y_5} \binp{y_5}{x_1, x_2} 
  %     (\apropout{17}{} \Par 
  %     \AmeliaMod{17}{\epsilon}{B'}_\empg ) \big) ) \ )\smallskip 
  %     \\ \bigskip & \quad \quad \text{where 
  %     $\widetilde c_{**} = (\prop_4, \dots, \prop_{12}, \prop_{17}, \dots, \prop_{25})$}
  % \end{align*}

  \noindent 
  Communication on $s_1$ leads to variable $x$ being substituted by name $a_3$,
  which is then passed on $c_{4}$ to the next process. In addition, inaction is
  simulated by synchronization on $\prop_{21}$.
  \begin{align*}
      \F{P} &\red^{13} \news{\widetilde c_{\bullet}} \news{a_3} ( \
      \apropout{5}{} \Par 
      \AmeliaMod{5}{\epsilon}{A' }_\empg \Par 
      \news{s} (
        \highlighta{\bout{a_3}{s}} \about{\dual s}{w_1, w_2})  \Par \\
      & \quad 
      \highlighta{\binp{a_3}{y_5}} \binp{y_5}{x_1, x_2} (\apropout{17}{} 
      \Par \AmeliaMod{17}{\epsilon}{B'  }_\empg ) \ ) \smallskip 
      \\ \bigskip & 
      \quad \quad \text{where $\widetilde c_{\bullet} = (\prop_5, \dots, c_{12}, c_{17}, \dots, c_{25})$}
  \end{align*}
  
  \noindent 
  Now, the distribution of the decomposition of $w$ from one process to another
  can finally be simulated by two reductions: first, a synchronization on $a_3$
  sends the endpoint of session $s$, which replaces variable $y_5$; afterwards,
  the dual endpoint is used to send the names $w_1,w_2$, substituting the
  variables $x_1,x_2$. 
  % Here, we remark that prefix $\abinp{s}{x_1,x_2}$ bounds 
  % variables $x_1,x_2$ in the breakdown of the continuation. 

  \begin{align*}
    \F{P} &\red^{14} \news{\widetilde c_{\bullet\bullet}} \news{s} ( \ 
    \apropout{5}{} \Par 
    \AmeliaMod{5}{\epsilon}{A' }_\empg 
    \Par \\
    & \qquad 
    \highlighta{\about{\dual s}{w_1, w_2}} \Par 
    \highlighta{\binp{s}{x_1, x_2}}
     \big(\apropout{17}{} \Par 
     \AmeliaMod{17}{\epsilon}{B' }_\empg \big)  \big) \smallskip 
 %   \\ \bigskip & \quad \quad \text{where 
    %$\widetilde c = (\prop_5, \dots, c_{12}, c_{17}, \dots, c_{25})$}
    \\
    %next reduction
     \F{P} &\red^{15} \news{\widetilde c_{\bullet\bullet}}\big( \ 
        \apropout{5}{} \Par \AmeliaMod{5}{\epsilon}{A' }_\empg \Par   
        \\
        &
        \qquad \apropout{17}{} \Par 
        \AmeliaMod{17}{\epsilon}{B'}_\empg \subst{w_1 w_2}{x_1 x_2}  \big) 
        = Q \smallskip 
      \\ \bigskip & \quad \quad \text{where 
      $\widetilde c_{\bullet \bullet} = (\prop_5, \dots, c_{12}, c_{17}, \dots, c_{25})$}
  \end{align*}

  \noindent 
  Here, we remark that as prefix $\abinp{s}{x_1,x_2}$ bounds 
  variables $x_1,x_2$ in the breakdown of the continuation 
  ($\AmeliaMod{17}{\epsilon}{B' }_\empg$). 
  Thus, there is no need for propagators to pass contexts: 
  propagators here only serve to enforce the ordering of actions. 
  On the other hand, this rely on arbitrary process nesting
  which is induced by the final application of encoding 
  $\map{\cdot}^2$ in the composition. 
   Thus the trio structure is lost. 
  % ( which is by the final application of encoding 
  % $\map{\cdot}^2$ in the composition.  )

  Undoubtedly, the first action of the original first-order process 
  has been simulated. We may notice that in $Q$ names $w_1$, $w_2$ substitute 
  $x_1$, $x_2$ and subsequent $\tau$-action on $w$ can be simulated on name $w_1$. 
  The following reductions follow the same pattern. 
  % Futher, we remark that prefix 
  % Undoubtedly, the behaviour of the initial first-order process has been 
  % simulated. 
  Thus, the outcome of our decomposition function is a functionally
  equivalent process that is typed with minimal session types.

\end{example}

  \smallskip

% \subsection{First Decomposition: Recursion}
% \label{pi:app:ss:exrec}

% \input{example-am-rec}

\subsection{First Decomposition: Labelled Choice}
\label{pi:app:ss:exsb}
% \label{pi:app:ss:exsb}
% Second Step Example
\noindent We now  illustrate how the approach in \Cref{pi:s:dbc} can be extended to account for labelled (deterministic) choice (selection and branching constructs).
In \HOp, these constructs are denoted
$$\bsel{u}{l} P \qquad \bbra{u}{l_i:P_i}_{i \in I}  $$
with reduction rule
$$
\bsel{n}{l_j} Q \Par \bbra{\dual{n}}{l_i : P_i}_{i \in I}  \red  Q \Par P_j ~~(j \in I)
$$

\begin{example}[First Decomposition: Labelled Choice]
%\emph{Example to be added}
\label{pi:ex:selbra-comp}
Let $P$ and $Q$ be \sessp processes which incorporate branching and selection:
\begin{align*}
	P = & ~\bbra{u}{l_1 : \news{h}(\bout{h}{m} \binp{h}{t} \inact \Par \binp{\dual{h}}{x} \bout{\dual h}{x} \inact), l_2 : \bout{s}{m} \binp{\dual{s}}{x} \inact } % = \bbra{u}{l_1: P_1, l_2 : P_2}$$
	\\
Q = & ~\bsel{\dual{u}}{l_1} \inact
\end{align*}

Let $R$ denote the restricted parallel composition of $P$ and $Q$: $R = \news{u}(P \Par Q)$. The respective process degrees have the same values as before.
\noindent The decomposition of $R$ is:
\begin{align*}
    \F{R} &= \news{c_1, \dots, c_5}(\propout{1}{} \inact \Par        \AmeliaMod{1}{\epsilon}{\news{u} (P \Par Q) \sigma}_g), \text{ where } \sigma = \subst{u_1 \dual{u_1}}{u \dual{u}}\\
                    &= \news{c_1, \dots, c_5}(\propout{1}{} \inact \Par \news{u_1} (\propinp{1}{} \propout{2}{} \apropbout{3}{} \Par \AmeliaMod{2}{\epsilon}{P}_g \Par \AmeliaMod{3}{\epsilon}{Q}_g))
\end{align*}
We consider $P$ and $Q$ separately. We begin with the breakdown of $Q$. 
\begin{align*}
% CHANGE THE INDEX OF a_1
    \AmeliaMod{3}{\epsilon}{Q}_g &= \propinp{3}{} \news{a_1} \big(\propout{4}{a_1} \big( \news{u_2} 
    \big( \propinp{4}{y} \news{s} \big(\bout{y}{s} \about{ \dual{s} }{ \dual u_2 } \big) \big) 
    \Par \propinp{5}{} \inact
        \Par \\ & \quad \binp{a_1}{y'} \binp{y'}{y_1} \bsel{u_1}{l_1} \binp{u_1}{z} \propout{5}{} 
        \news{s'} \big(\bout{z}{s'} \about{\dual s'}{y_1} \big) \big) \big)
\end{align*}
The breakdown of process $P$ is:
\begin{align*}
    \AmeliaMod{2}{\epsilon}{P}_g &= \propinp{2}{} \bbra{u_1}{l_1: \news{a_2} \bout{u_1}{a_2} \binp{a_2}{y''} 
    \binp{y''}{ y_1}  
    \news{c_3, \dots, c_{21}}\big( \apropout{3}{} \Par \AmeliaMod{3}{\epsilon}{P_1 \subst{y_1}{u_1}}_g \big),\\
    & \qquad \qquad \qquad  l_2 : \news{a_2} \bout{u_1}{a_2} \binp{a_2}{y''} \binp{y''}{y_1}   
    \news{c_3, \dots, c_{11}} \big( \apropout{3}{} \Par \AmeliaMod{3}{\epsilon}{P_2 \subst{y_1}{u_1}}_g \big)}
\end{align*}
As in the previous approach of this example, we are interested in the breakdown of $P_1$, because it belongs to the selected branch.
\begin{align*}
 \AmeliaMod{3}{\epsilon}{P_1 \subst{y_1}{u_1}}_g &= \news{h_1, h_2} 
        \AmeliaMod{3}{\epsilon}{\bout{h_1}{m_1} \binp{h_1}{t} \inact \Par \binp{\dual{h_1}}{x} \bout{\dual h_1}{x} \inact}_g\\
        &= \news{h_1, h_2} \big(\propinp{3}{} \propout{4}{} \apropout{13}{} 
        \Par \AmeliaMod{4}{\epsilon}{\bout{h_1}{m_1} \binp{h_1}{t} \inact}_g 
        \Par \AmeliaMod{13}{\epsilon}{\binp{\dual{h_1}}{x} \bout{\dual{ h_1}}{x} \inact}_g \big)
\end{align*}
\begin{align*}
    \AmeliaMod{4}{\epsilon}{\bout{h_1}{m_1}_g \binp{h_1}{t} \inact} &= 
      \propinp{4}{} \news{a_3} \big(\bout{h_1}{a_3} 
      \big( \apropout{7}{} \Par \AmeliaMod{7}{\epsilon}{\binp{h_2}{t} \inact}_g 
      \Par \binp{a_3}{y_2} \binp{y_2}{z_1} \apropout{5}{z_1} \Par \\
                    & \qquad \propinp{5}{z_1} \binp{z_1}{x} 
                    \apropbout{6}{x} \Par \propinp{6}{x} \news{s_1} 
                    \big(\bout{x}{s_1} \bout{ \dual{s_1} }{m_1} \inact ) \big) \big)\\
    \AmeliaMod{7}{\epsilon}{\binp{h_2}{t} \inact}_g &=  
                \propinp{7}{}\binp{h_2}{y_3} \apropout{8}{ y_3} \Par 
                \newsp{s_2} {\propinp{8}{y_3} \propout{9}{y_3} \apropout{10}{} \Par \\
               & \quad {} \propinp{9}{y_3} \news{s_3} \big(\bout{y_3}{s_3} \bout{\dual{s_3}}{s_2} \inact \big) 
               \Par \propinp{10}{} \news{a_4} \big(\bout{\dual{s_2}}{a_4} \big( \apropout{12}{} \Par \\
               & \quad  \propinp{12}{} \inact \Par \binp{a_4}{y_4} \binp{y_4}{t_1} 
               \apropout{11}{} \Par \propinp{11}{} \inact \  \big) }\\
    \AmeliaMod{13}{\epsilon}{\binp{\dual{h_1}}{x} \bout{\dual{ h_1}}{x} \inact}_g &= 
             \propinp{13}{}\binp{\dual{h_1}}{y_5} \apropout{14}{y_5} \Par \newsp{s_4} {\propinp{14}{y_5} \propout{15}{y_5} \apropout{16}{} \Par \\
               & \quad {} \propinp{15}{y_5} \news{s_5}\big(\bout{y_5}{s_5} \bout{\dual{s_5}}{s_4} \inact \big) 
               \Par \propinp{16}{} \news{a_5} \big(\bout{\dual{s_4}}{a_5} \big( \apropout{21}{} \Par \\
               & \quad  \propinp{21}{} \inact \Par 
               \binp{a_5}{y_6} \binp{y_6}{x_1} \apropout{17}{x_1} 
               \Par \AmeliaMod{17}{x_1}{ \bout{\dual{ h_2}}{x_1} \inact }_g  \ \big) \big) }\\
    \AmeliaMod{17}{x_1}{ \bout{\dual{ h_2}}{x_1} \inact }_g &= 
                    \propinp{17}{x_1} \news{a_6} \big(\bout{\dual{h_2}}{a_6} 
                    \big( \apropout{20}{x_1} \Par\propinp{20}{} \inact 
                    \Par \binp{a_6}{y_7} \binp{y_7}{z_2} \apropout{18}{z_2} \Par \\
                    & \qquad \propinp{18}{z_2} \binp{z_2}{x'} \apropbout{19}{x'} 
                    \Par \propinp{19}{x'} \news{s_6} (\bout{x'}{s_6} \bout{ \dual{s_6} }{x_1} \inact \big) \big) \big)
\end{align*}
In order to verify that the decomposition of $R$ simulates the behaviour of the initial process, we refer to its reduction chain. The first transitions involve synchronization on $c_1, c_2, c_3$ and $c_4$. The trigger name $a_2$ is passed through propagator $c_4$, such that it replaces variable $y$.
\begin{align*}
    \F{R} &\red^4 \news{c_5} \news{u_1} \big(\bbra{u_1}{l_1: \news{a_2} \ 
    \bout{u_1}{a_2} \binp{a_2}{y''} \binp{y''}{ y_1}  
    \news{c_3, \dots, c_{21}}\big( \apropout{3}{} \Par \\
    &  \qquad \AmeliaMod{3}{\epsilon}{P_1 \subst{y_1}{u_1}}_g ), \ l_2 : \news{a_2} \ \bout{u_1}{a_2} \binp{a_2}{y''} \binp{y''}{y_1}   
      \news{c_3, \dots, c_{11}}\big( \apropout{3}{} \Par\\
       &  \qquad \AmeliaMod{3}{\epsilon}{P_2 \subst{y_1}{u_1}}_g )} \Par \news{a_1} \big( \news{u_2} 
       \big( \news{s} \big(\bout{a_1}{s} \about{ \dual{s} }{ \dual u_2 } \big) \big) \Par \propinp{5}{} \inact
        \Par \\ & \qquad \binp{a_1}{y'} \binp{y'}{y_1} \bsel{u_1}{l_1} \binp{u_1}{z} \propout{5}{} \news{s'} 
        \big(\bout{z}{s'} \about{\dual s'}{y_1} \big) \big)  ) 
\end{align*}
The next step involves synchronization on $a_1$, which leads to the variable $y'$ being substituted by session name $s$.
\begin{align*}
    \F{R} &\red^5 \news{c_5} \news{u_1} \big(\bbra{u_1}{l_1: \news{a_2} \ 
    \bout{u_1}{a_2} \binp{a_2}{y''} \binp{y''}{ y_1}  
    \news{c_3, \dots, c_{21}} \big( \apropout{3}{} \Par \\
    &  \qquad \AmeliaMod{3}{\epsilon}{P_1 \subst{y_1}{u_1}}_g ), \ l_2 : \news{a_2} \ \bout{u_1}{a_2} \binp{a_2}{y''} \binp{y''}{y_1}   
      \news{c_3, \dots, c_{11}} \big( \apropout{3}{} \Par\\
       &  \qquad \AmeliaMod{3}{\epsilon}{P_2 \subst{y_1}{u_1}}_g \big)} \Par \news{s} \big( \news{u_2} 
       \big(   \about{ \dual{s} }{ \dual u_2 }  \big) \Par \propinp{5}{} \inact
        \Par \\ & \qquad  \binp{s}{y_1} \bsel{u_1}{l_1} \binp{u_1}{z} \propout{5}{} \news{s'} 
        \big(\bout{z}{s'} \about{\dual s'}{y_1} \big) \big)  \big) 
\end{align*}
Now, session name $s$ and its dual endpoint can communicate - channel name $\dual{u_2}$ is sent, replacing $y_1$.
\begin{align*}
    \F{R} &\red^6 \news{c_5} \news{u_1} \big(\bbra{u_1}{l_1: \news{a_2} \ 
    \bout{u_1}{a_2} \binp{a_2}{y''} \binp{y''}{ y_1}  
    \news{c_3, \dots, c_{21}} \big( \apropout{3}{} \Par \\
    &  \qquad \AmeliaMod{3}{\epsilon}{P_1 \subst{y_1}{u_1}}_g ), \ l_2 : \news{a_2} \ \bout{u_1}{a_2} \binp{a_2}{y''} \binp{y''}{y_1}   
      \news{c_3, \dots, c_{11}} \big( \apropout{3}{} \Par\\
       &  \qquad \AmeliaMod{3}{\epsilon}{P_2 \subst{y_1}{u_1}}_g \big)} \Par \news{u_2} \big(\propinp{5}{} \inact
        \Par  \bsel{u_1}{l_1} \binp{u_1}{z} \propout{5}{} \news{s'} \big(\bout{z}{s'} \about{\dual s'}{\dual{u_2}} 
        \big) \big)  \big) 
\end{align*}
At this point, the action of choosing the first branch can be simulated by selecting label $l_1$ on channel name $u_1$.
\begin{align*}
    \F{R} &\red^7 \news{c_5} \news{u_1} \big( \news{a_2} \ \bout{u_1}{a_2} \binp{a_2}{y''} \binp{y''}{ y_1}  
    \news{c_3, \dots, c_{21}}( \apropout{3}{} \Par \\
    &  \qquad \AmeliaMod{3}{\epsilon}{P_1 \subst{y_1}{u_1}}_g ) \Par \news{u_2} \big(\propinp{5}{} \inact
        \Par \binp{u_1}{z} \propout{5}{} \news{s'} \big(\bout{z}{s'} \about{\dual s'}{\dual{u_2}} \big) \big)  ) 
\end{align*}
The following two reductions consist of synchronizations on $u_1$ and $c_5$. As a result, variable $z$ is replaced by the trigger name $a_2$.
\begin{align*}
    \F{R} &\red^9 \news{a_2} \big(\binp{a_2}{y''} \binp{y''}{ y_1}  
    \news{c_3, \dots, c_{21}} \big( \apropout{3}{} \Par \\
    &  \qquad \AmeliaMod{3}{\epsilon}{P_1 \subst{y_1}{u_1}}_g \big) \Par \news{u_2} 
    \big( \news{s'} \big(\bout{a_2}{s'} \about{\dual s'}{\dual{u_2}} \big) \big)  ) 
\end{align*}
Communication on $a_2$ allows for synchronization on $s'$. Channel $a_2$ receives the session name $s'$, which further receives the dual endpoint $\dual{u_2}$.
\begin{align*}
    \F{R} &\red^{11} \news{c_3, \dots, c_{21}} \news{u_2} \big( \apropout{3}{} 
    \Par \AmeliaMod{3}{\epsilon}{P_1 \subst{\dual{u_2}}{u_1}}_g \big) \\
                    &= \news{c_3, \dots, c_{21}} \news{u_2} \big( \apropout{3}{} \Par \news{h_1, h_2} 
                    \big(\propinp{3}{} \propout{4}{} \apropout{13}{} \Par \\ & \quad 
                    \AmeliaMod{4}{\epsilon}{\bout{h_1}{m_1} \binp{h_1}{t} \inact}_g \Par 
                    \AmeliaMod{13}{\epsilon}{\binp{\dual{h_1}}{x} \bout{\dual{ h_1}}{x} \inact}_g \big)  \big)
\end{align*}
Remarkably, the obtained result reflects the broken down version of process
$P_1$. Following three more reductions, in which $c_3, c_4$ and $c_{13}$
synchronize with their respective duals, the breakdown of each parallel
sub-process will be activated. We refrain from presenting the remaining
reduction steps, as they represent a standard case of name-passing. Clearly, the
decomposed process $\F{R}$ behaves in a similar manner to the initial process
$R$.
\end{example}

\newpage
