# Supplementary material for: Minimal Session Types for the $\pi$-calculus (Extended Version)
Source: arXiv:2107.10936 source file (2024-01-22)
Supplement: Supplementary file 2 [file appendix-mst-prelim.tex]

\newpage

% \subsection{First Decomposition: Recursion}
% \label{app:ss:exrec}

% \input{example-am-rec}

\section{Relevant notions from~\cite{DBLP:journals/iandc/KouzapasPY19}}
\label{top:app:relexp}

\subsection{Session Types for \HOp} \label{top:app:typing}
\input{type_system}

\subsection{Labelled Transition System for \HOp}

%%%%%%%%%%%%%%%%%%%% LTS Figure %%%%%%%%%%%%%%%%%%%%%%%%%%%%%%%%%%%%%
\begin{figure}[h]
  \begin{mdframed}
	\begin{mathpar}
		\inferrule[\ltsrule{App}]{
		}{
			\appl{(\abs{x}{P})}{V} \by{\tau} P \subst{V}{x}
		}
		\and
		\inferrule[\ltsrule{Snd}]{
		}{
			\bout{n}{V} P \by{\bactout{n}{V}} P
		}
		\and
		\inferrule[\ltsrule{Rv}]{
		}{
			\binp{n}{x} P \by{\bactinp{n}{V}} P\subst{V}{x}
		}
		\and
		\inferrule[\ltsrule{Sel}]{
		}{
			\bsel{s}{l}{P} \by{\bactsel{s}{l}} P
		}
		\and
		\inferrule[\ltsrule{Bra}]{j\in I
		}{
			\bbra{s}{l_i:P_i}_{i \in I} \by{\bactbra{s}{l_j}} P_j 
		}
		\and
		\inferrule[\ltsrule{Alpha}]{
			P \scong_\alpha Q
			\and
			Q\by{\ell} P'
		}{
			P \by{\ell} P'
		}
		\and
		\inferrule[\ltsrule{Res}]{
			P \by{\ell} P'
			\and
			n \notin \fn{\ell}
		}{
			\news{n} P \by{\ell} \news{n} P'
		}
		\and
		\inferrule[\ltsrule{New}]{
			P \by{\news{\widetilde{m}} \bactout{n}{V}} P'
			\and
			m_1 \in \fn{V}
		}{
			\news{m_1} P \by{\news{m_1\cat\widetilde{m}} \bactout{n}{V}} P'
		}
		\and
		\inferrule[\ltsrule{Par${}_L$}]{
			P \by{\ell} P'
			\and
			\bn{\ell} \cap \fn{Q} = \es
		}{
			P \Par Q \by{\ell} P' \Par Q
		}
		\and
		\inferrule[\ltsrule{Tau}]{
			P \by{\ell_1} P'
			\and
			Q \by{\ell_2} Q'
			\and
			\ell_1 \asymp \ell_2
		}{
			P \Par Q \by{\tau} \newsp{\bn{\ell_1} \cup \bn{\ell_2}}{P' \Par Q'}
		}
		\and
		\inferrule[\ltsrule{Rec}]{
			P\subst{\recp{X}{P}}{\rvar{X}} \by{\ell} P'
		}{
			\recp{X}{P}  \by{\ell} P'
		}
	\end{mathpar}
\end{mdframed}
\caption{The Untyped LTS for \HOp processes. We omit Rule $\ltsrule{Par${}_R$}$.  
%\label{top:fig:untyped_LTS}
}
\end{figure}

%%%%%%%%%%%%%%%%%%%% End LTS Figure %%%%%%%%%%%%%%%%%%%%%%%%%%%%%%%%%

%%%%%%%%%%%%%%%%%%%% Environment LTS Figure %%%%%%%%%%%%%%%%%%%%%%%%%
\begin{figure}[h]
  \begin{mdframed}
  \begin{mathpar}
    \inferrule[\eltsrule{SRv}]{
      \dual{s} \notin \dom{\Delta}
      \and
      \Gamma; \Lambda'; \Delta' \proves V \hastype U
    }{
      (\Gamma; \Lambda; \Delta \cat s: \btinp{U} S) \by{\bactinp{s}{V}} (\Gamma; \Lambda\cat\Lambda'; \Delta\cat\Delta' \cat s: S)
    }
    \and
    \inferrule[\eltsrule{ShRv}]{
      \Gamma; \es; \es \proves a \hastype \chtype{U}
      \and
      \Gamma; \Lambda'; \Delta' \proves V \hastype U
    }{
      (\Gamma; \Lambda; \Delta) \by{\bactinp{a}{{V}}} (\Gamma; \Lambda\cat\Lambda'; \Delta\cat\Delta')
    }
    \and
    \inferrule[\eltsrule{SSnd}]{
      \begin{array}{l}
        \Gamma \cat \Gamma'; \Lambda'; \Delta' \proves V \hastype U
        \and
        \Gamma'; \es; \Delta_j \proves m_j  \hastype U_j
        \and
        \dual{s} \notin \dom{\Delta}
        \\
        \Delta'\backslash (\cup_j \Delta_j) \subseteq (\Delta \cat s: S)
        \and
        \Gamma'; \es; \Delta_j' \proves \dual{m}_j  \hastype U_j'
        \and
        \Lambda' \subseteq \Lambda
      \end{array}
    }{
      (\Gamma; \Lambda; \Delta \cat s: \btout{U} S)
      \by{\news{\widetilde{m}} \bactout{s}{V}}
      (\Gamma \cat \Gamma'; \Lambda\backslash\Lambda'; (\Delta \cat s: S \cat \cup_j \Delta_j') \backslash \Delta')
    }
    \and
    \inferrule[\eltsrule{ShSnd}]{
      \begin{array}{l}
        \Gamma \cat \Gamma' ; \Lambda'; \Delta' \proves V \hastype U
        \and
        \Gamma'; \es; \Delta_j \proves m_j \hastype U_j
        \and
        \Gamma ; \es ; \es \proves a \hastype \chtype{U}
        \\
        \Delta'\backslash (\cup_j \Delta_j) \subseteq \Delta
        \and
        \Gamma'; \es; \Delta_j' \proves \dual{m}_j\hastype U_j'
        \and
        \Lambda' \subseteq \Lambda
      \end{array}
    }{
      (\Gamma ; \Lambda; \Delta) \by{\news{\widetilde{m}}
      \bactout{a}{V}}
      (\Gamma \cat \Gamma'; \Lambda\backslash\Lambda'; (\Delta \cat \cup_j \Delta_j') \backslash \Delta')
    }
    \and
    \inferrule[\eltsrule{Sel}]{
      \dual{s} \notin \dom{\Delta}
      \and
      j \in I
    }{
      (\Gamma; \Lambda; \Delta \cat s: \btsel{l_i: S_i}_{i \in I}) \by{\bactsel{s}{l_j}} (\Gamma; \Lambda; \Delta \cat s:S_j)
    }
    \and
    \inferrule[\eltsrule{Bra}]{
      \dual{s} \notin \dom{\Delta} \quad j \in I
    }{
      (\Gamma; \Lambda; \Delta \cat s: \btbra{l_i: T_i}_{i \in I}) \by{\bactbra{s}{l_j}} (\Gamma; \Lambda; \Delta \cat s:S_j)
    }
    \and
    \inferrule[\eltsrule{Tau}]{
      \Delta_1 \red \Delta_2 \vee \Delta_1 = \Delta_2
    }{
      (\Gamma; \Lambda; \Delta_1) \by{\tau} (\Gamma; \Lambda; \Delta_2)
    }
  \end{mathpar}
\end{mdframed}
\caption{Labelled Transition System for Typed Environments. 
  \label{top:fig:envLTS}}
  \end{figure}

  %%%%%%%%%%%%%%%%%%%% End Environment LTS Figure %%%%%%%%%%%%%%%%%%%%%%

\noi
The typed LTS  combines
the LTSs in~\Cref{top:fig:untyped_LTS}
and~\Cref{top:fig:envLTS}. 

\begin{definition}[Typed Transition System]
	\label{top:d:tlts}
	A {\em typed transition relation} is a typed relation
	$\horel{\Gamma}{\Delta_1}{P_1}{\by{\ell}}{\Delta_2}{P_2}$
	where:
	\begin{enumerate}
		\item
				$P_1 \by{\ell} P_2$ and 
		\item
				$(\Gamma, \emptyset, \Delta_1) \by{\ell} (\Gamma, \emptyset, \Delta_2)$ 
				with $\Gamma; \emptyset; \Delta_i \proves P_i \hastype \Proc$ ($i=1,2$).
%				\dk{We sometimes annotated the output action with
%				the type of value $V$ as in $\widetilde{m} \bactout{n}{V: U}$.}
	\end{enumerate}
	We 
	%extend to $\By{}$ and $\By{\hat{\ell}}$  where we 
	write  $\By{}$ for the reflexive and transitive closure of $\by{}$,
	$\By{\ell}$ for the transitions $\By{}\by{\ell}\By{}$, and $\By{\hat{\ell}}$
	for $\By{\ell}$ if $\ell\not = \tau$ otherwise $\By{}$.
\end{definition}

In this section we recall  relevant notions from ~\cite{DBLP:journals/iandc/KouzapasPY19}. 

\subsection{Encoding of \HOp into \HO}

\begin{figure}[h!]
  \begin{mdframed}
	\begin{align*}
		\auxmapp{\bout{w}{\abs{x}{Q}} P}{{}}{\sigma} & \defeq \bout{u}{\abs{x}{\auxmapp{Q}{{}}{{\sigma \cat x}}}} \auxmapp{P}{{}}{\sigma}
		&
		\auxmapp{\bbra{w}{l_i:P_i}_{i \in I}}{{}}{\sigma} & \defeq \bbra{u}{l_i:\auxmapp{P_i}{{}}{\sigma}}_{i \in I}		
		\\
		\auxmapp{\binp{w}{x} P}{{}}{\sigma} & \defeq \binp{u}{x} \auxmapp{P}{{}}{\sigma} 
		&
		\auxmapp{\bsel{w}{l} P}{{}}{\sigma} & \defeq \bsel{u}{l} \auxmapp{P}{{}}{\sigma} 
		\\
		\auxmapp{\news{n} P}{{}}{\sigma} & \defeq \news{n} \auxmapp{P}{{}}{{\sigma \cat n}}
		&
		\auxmapp{\appl{(\lambda x.Q)}{w}}{{}}{\sigma}  & \defeq \appl{(\lambda x.\auxmapp{Q}{{}}{{\sigma \cat x}})}{u}
		\\
		\auxmapp{P \Par Q}{{}}{\sigma} & \defeq \auxmapp{P}{{}}{\sigma} \Par \auxmapp{Q}{{}}{\sigma} 
		&
		\auxmapp{\appl{x}{w}}{{}}{\sigma} & \defeq \appl{x}{u}
		\\
		\auxmapp{\inact}{{}}{\sigma}  & \defeq  \inact	
		& 
\end{align*}
\begin{center}
	{In all cases: $u = 
	\begin{cases} 
	x_n & \text{if $w$ is a name $n$ and  $n \not\in \sigma$ ($x$ fresh)}
	\\
	w & \text{otherwise: $w$ is a variable or a name $n$ and $n \in \sigma$} 
	 	\end{cases}$}
\end{center}
\end{mdframed}
%\vspace{-3mm}
\caption{\label{top:f:auxmap} Auxiliary mapping used to encode \HOp into \HO (\defref{top:d:auxmap}).}
%\vspace{-1mm}
%\Hlinefig 
\end{figure}

\begin{definition}[Auxiliary Mappings] \label{top:d:trabs}
  \label{top:d:auxmap}
  We define mappings $\vmap{\cdot}$ and $\auxmapp{\cdot}{{}}{\sigma}$ as follows:
  \begin{itemize}
  \item  $\vmap{\cdot}: 2^{\mathcal{N}} \longrightarrow \mathcal{V}^\omega$
    is a map of sequences of lexicographically ordered names to sequences of variables, defined
    inductively 
    as: 
    \begin{align*}
    \vmap{\epsilon} & = \epsilon 
    \\
    \vmap{n \cat \tilde{m}} & = x_n \cat \vmap{\tilde{m}} \quad \text{($x$ fresh)}
    \end{align*}
  
  \item Given a set of session names and variables $\sigma$, 
     the   map
    $\auxmapp{\cdot}{{}}{\sigma}: \HO \to \HO$
    is as in \figref{top:f:auxmap}.
    \end{itemize}
  \end{definition}
