# Supplementary material for: Minimal Session Types for the $\pi$-calculus (Extended Version)
Source: arXiv:2107.10936 source file (2024-01-22)
Supplement: Supplementary file 3 [file appendix-ppdp2021.tex]

\newpage
\section{Additional Examples}

\subsection{First Decomposition: Core Fragment}
\label{app:ss:amcore}

\begin{example}[Core Fragment]
  \label{ex:ex1-decomp}
  % Let $P$ be a \sessp process which incorporates name-passing and $w$ be a
  % channel through which first an integer value, then a boolean value is sent. 
  Let $P$ be a \sessp process which incorporates name-passing 
  and implements channels $u$ and $\dual w$ with types 
    $S = \btout{\dual T}\tinact$ 
  and $T = \btinp{\mathsf{Int}}\btout{\mathsf{Bool}}\tinact$, respectively:
  % The degree of $P$ is $\lenHO{P} = 25$.
  \begin{align*}
    P &= \news{u:S}(\bout{u}{w} \binp{\dual w}{t} \bout{\dual w}{\unaryint{t}} \inact \Par
      \binp{\dual u}{x} \bout{x}{\textsf{5}}\binp{x}{b} \inact) = \news{u}(A \Par B)	
  \end{align*}
  
  \noindent 
  The degree of $P$ is $\lenHO{P} = 25$.
  Then, the decomposition of $P$ into a collection of first-order processes
  typed with minimal session types is:
  \begin{align*}
    \F{P} &= \news{ \prop_1, \dots, c_{25}}\big(\propout{1}{} \inact \Par 
              \AmeliaMod{1}{\epsilon}{P\sigma}_\empg \big)\\
          &= \news{ \prop_1, \dots, c_{25}}\big(\propout{1}{} \inact \Par 
          \AmeliaMod{1}{\epsilon}{\news{u}(A \Par B)\sigma}_\empg \big)\\
          &= \news{ \prop_1, \dots, c_{25}}\big(\propout{1}{} \inact 
          \Par \news{u_1} \AmeliaMod{1}{\epsilon}{(A \Par B)\sigma'}_\empg \big), \\
          &\text{ where } \sigma = \mathsf{init}(\fn{P}),\ 
          \sigma' = \sigma \cdot \subst{u_1 \dual{u_1}}{u\dual{u}}
  \end{align*}

  \noindent We have:
  \begin{align*}
      \AmeliaMod{1}{\epsilon}{(A \Par B)\sigma'}_\empg \big) &= 
      \propinp{1}{} \propout{2}{}  \apropout{13}{}  \Par 
      \AmeliaMod{2}{\epsilon}{A \sigma'}_\empg \Par \AmeliaMod{13}{\epsilon}{B \sigma'}_\empg
  \end{align*}

  \noindent We use some abbreviations for 
  subprocesses of $A$ and $B$ : 
  \begin{align*}
    A' &= \binp{\dual{w}_1}{t}A''   
    \qquad A'' = \bout{\dual w_1}
    {\unaryint{t}}\inact  \\
    B' &= \bout{x_1}{5} B''  
    \qquad B'' = \binp{x_1}{b}\inact 
  \end{align*}

  \noindent The breakdown of $A$ is:
  \begin{align*}
  % A
  \AmeliaMod{2}{\epsilon}{A}_\empg &= \propinp{2}{} \news{a_1}\big(\bout{u_1}{a_1} \big( 
      \apropout{5}{} \Par \AmeliaMod{5}{\epsilon}{A'}_\empg 
      \Par \binp{a_1}{y_1} \binp{y_1}{z_1} \apropout{3}{z_1} \Par \\
      & \quad \propinp{3}{z_1} \binp{z_1}{x} \apropout{4}{x} \Par 
      \propinp{4}{x} \news{s} \big(\bout{x}{s} \about{\dual s}{w_1, w_2}\big) \big) \big)\\
  % next row
  \AmeliaMod{5}{\epsilon}{A'}_\empg &= 
  \propinp{5}{} \binp{\dual{w_1}}{y_2} \apropout{6}{y_2} \Par 
  \news{s_1} \big( \propinp{6}{y_2} \propout{7}{y_2} \apropbout{8}{} \Par \\
      & \quad \propinp{7}{y_2} \news{s'}\big( \bout{y_2}{s'}  \bout{\dual{s'}}{s_1} \inact \big) \big) 
      \Par \propinp{8}{} \news{a_2} \big( \bout{\dual{s_1}}{a_2} \big(\apropout{10}{} 
      \Par \propinp{10}{} \inact \Par \\
      & \quad \binp{a_2}{y_3} \binp{y_3}{t_1} 
      \big( \apropout{9}{} \Par
      \AmeliaMod{9}{\epsilon}{A''}_\empg  \big) \big) \big)  \\
      %  third row
       \AmeliaMod{9}{\epsilon}{A''}_\empg &= 
    \propinp{9}{} \news{a} \big(\bout{\dual w_2}{a}
    \big( \apropout{12}{} \Par \propinp{12}{}\inact \Par 
     \\
     & \qquad \binp{a}{y} \binp{y}{z_1} \apropout{11}{z_1} \Par
     \propinp{10}{z_1} \binp{z_1}{x} \apropout{11}{x} \Par
    %  \\
    %  &
    %  \qquad \qquad \qquad \qquad 
     \propinp{11}{x} 
     \news{s} \big(\bout{x}{s} \about{ \dual{s} }{\unaryint{t}}\big) \big) \big)
  \end{align*}

  % \begin{align*}
  %   \AmeliaMod{9}{\epsilon}{\bout{\dual w_2}{\textsf{true}}\inact }_g &= 
  %   \propinp{9}{} \news{a} \big(\bout{\dual w_2}{a}
  %   ( \apropout{12}{} \Par \propinp{12}{}\inact \Par 
  %    \\
  %    & \qquad \binp{a}{y} \binp{y}{z_1} \apropout{11}{z_1} \Par
  %    \propinp{10}{z_1} \binp{z_1}{x} \apropout{11}{x} \Par
  %    \\
  %    &\qquad \qquad \qquad \qquad \propinp{11}{x} 
  %    \news{s} (\bout{x}{s} \about{ \dual{s} }{\textsf{true}}) ) \big)
  % \end{align*}
  
  \noindent The breakdown of $B$ is:
  \begin{align*}
    \AmeliaMod{13}{\epsilon}{B}_\empg &= 
    \propinp{13}{}\binp{\dual u_1}{y_4}\apropout{14}{y_4}  \Par 
    \news{s_1}\big( \propinp{14}{y}\propout{15}{y}\apropout{16}{} 
    \Par \\
    & \quad \propinp{15}{y_4} \news{s''} \big(\bout{y_4}{s''} 
      \bout{\dual{s''}}{s_1} \inact \big) \Par 
      \propinp{16}{} \news{a_3} \big(\bout{s_1}{a_3} \big( \apropout{21}{} \Par \\
    & \quad \propinp{21}{} \inact \Par 
    \binp{a_3}{y_5} \binp{y_5}{x_1, x_2} 
    \big(\apropout{17}{} \Par \AmeliaMod{17}{\epsilon}{B'}_\empg \big) \big) \big) \big) 
    \smallskip \bigskip \\
    % new row
  \AmeliaMod{17}{\epsilon}{B'}_\empg &=  
      \propinp{17}{} \news{a_4} \big( \bout{x_1}{a_4} \big( \apropout{20}{}  
      \Par \AmeliaMod{20}{\epsilon}{B''}_\empg  
      \Par \binp{a_4}{y_6} \binp{y_6}{z_1} 
      \apropout{18}{z_1} \Par \\
      & \quad \propinp{18}{z_1} \binp{z_1}{x} \apropout{19}{x} \Par 
      \propinp{19}{x} \news{s'''} \big(\bout{x}{s'''} \about{\dual{s'''}}{\textsf{5} } \big) \big) \big)
      \\
      % new row 
      \AmeliaMod{20}{\epsilon}{B''}_\empg &= 
      \propinp{20}{}\binp{x_2}{y} \apropout{21}{y} \Par
      \\
      &\qquad \news{s_1} \big(\propinp{21}{y} \propout{22}{y} \apropout{23}{} \Par
       \propinp{22}{y} \news{s}\big(\bout{y}{s} \about{\dual{s}}{s_1}   \big) \Par
      \\
      &\qquad \qquad \qquad \propinp{23}{\wtd x} \news{a}  \big(\bout{\dual{s_1}}{a} 
      \big( \apropout{25}{} \Par \propinp{25}{} \inact \Par \\
      & \qquad \qquad \qquad \binp{a}{y'} \binp{y'}
        {b_1} \big( \apropout{24}{} \Par
        \propinp{24}{}\inact \big)   \big) \big) \big) 
  \end{align*}

% \begin{align*}
%   \AmeliaMod{20}{\epsilon}{\binp{x_2}{b} \inact}_\empg &= 
%   \propinp{20}{}\binp{x_2}{y} \apropout{21}{y} \Par
%   \\
%   &\qquad \news{s_1} \big(\propinp{21}{y} \propout{22}{y} \apropout{23}{} \Par
%    \propinp{22}{y} \news{s}(\bout{y}{s} \about{\dual{s}}{s_1}   ) \Par
%   \\
%   &\qquad \qquad \qquad \propinp{23}{\wtd x} \news{a}  (\bout{\dual{s_1}}{a} 
%   ( \apropout{25}{} \Par \propinp{25}{} \inact \Par \\
%   & \qquad \qquad \qquad \binp{a}{y'} \binp{y'}
%     {b_1} \big( \apropout{24}{} \Par
%     \propinp{24}{}\inact \big)   ) ) \big) 
%   % &\text{where}
%   % \\
%   %   \widehat{Q}_{\tilde{x}} &= \binp{a}{y'} \binp{y'}
%   %   {b_1} \big( \apropout{k+4}{} \Par
%   %   \AmeliaMod{k+4}{}{Q \subst{w_1}{w} \sigma }_\empg \big) 
% \end{align*}
  \noindent Names $\dual w_1$ and $\dual w_2$ are typed with 
  $M_1 = \bbtinp{ \lrangle{ \btinp{ \btinp{ \lrangle{ \btinp{ \textsf{Int} }{\tinact} } }{\tinact} }{\tinact} } }{\tinact}$ and 
  $M_2 = \bbtout{ \lrangle{ \btinp{ \btinp{ \lrangle{ \btinp{ \textsf{Bool}}{\tinact} } }{\tinact} }{\tinact} } }{\tinact}$, 
  respectively.
   Name $u_1$ is typed with 
  $\bbtout{ \lrangle{ \btinp{ \btinp{ \lrangle{ \btinp{ \dual M_1, \dual M_2 }{\tinact} } }{\tinact} }{\tinact} } }{\tinact}$. 
  Now let us observe the reduction chain. The collection of processes
  synchronizes on $\prop_1, \prop_2, \prop_{13}$ after three reductions.
  \begin{align*}
    \F{P} &\red^{3} \news{\widetilde c} \big( \ \news{a_1} \big( \highlighta{\bout{u_1}{a_1}} \big( 
      \apropout{5}{} \Par 
      \AmeliaMod{5}{\epsilon}{A' }_\empg \Par
      % \\
      % & \quad  
      \binp{a_1}{y_1} \binp{y_1}{z_1} \apropout{3}{z_1} \Par 
       \propinp{3}{z_1} \binp{z_1}{x} \apropout{4}{x} \Par 
       \\
      & \quad
      \propinp{4}{x} \news{s} \big(\bout{x}{s} \about{\dual s}{w_1, w_2}\big) \big) \big) \Par 
     \highlighta{\binp{\dual u_1}{y_4}}\apropout{14}{y_4}    \Par 
    %  \\
    %   & \quad 
    \news{s_1}\big( \propinp{14}{y}\propout{15}{y}\apropout{16}{} 
    \Par  
    \\
    & \qquad 
    \propinp{15}{y_4} \news{s''} \big(\bout{y_4}{s''} 
      \bout{\dual{s''}}{s_1} \inact \big) \Par 
    %   \\
    % & \qquad
      \propinp{16}{} \news{a_3} \big(\bout{s_1}{a_3} \big( \apropout{21}{} \Par \\
    & \qquad \quad \propinp{21}{} \inact \Par 
    \binp{a_3}{y_5} \binp{y_5}{x_1, x_2} 
    \big(\apropout{17}{} \Par 
    \AmeliaMod{17}{\epsilon}{B'}_\empg \big) \big) \big) \big)
    \smallskip \bigskip  
      \\ \bigskip & \quad \quad 
      \text{where $\widetilde c = (\prop_3, \dots, \prop_{12}, \prop_{14}, \dots, c_{25})$}
  \end{align*}
  
  \noindent Then, the broken down process $A$ communicates with process $B$
  through channel $u_1$ by passing name $a_1$ (highlighted above).
  % which is
  % further sent on $\prop_{14}$
  % and $\prop_{15}$. 
  Here we notice that the original transmission of value $w$ 
  is not immediately mimicked on channel $u$, but it is delegated to 
  some other channel through series of channel redirections 
  starting with the transmission of name $a_1$. 
  % Further, by breaking down sequential prefixes involved in channel redirections 
  % redundant communications on propagators are introduced. 
  Further,  received name $a_1$ is locally propagated by $\prop_{14}$
  and $\prop_{15}$. This represents redundant communications on propagators 
  induced by breaking down sequential prefixes produced by 
  two encodings $\map{\cdot}^1_g$ and $\map{\cdot}^{2}$
  (not present in the original process). 
  Another synchronization occurs on $\prop_{16}$.
  \begin{align*}
    \F{P} &\red^{7} \news{\widetilde c_*}\news{a_1} \big( \  
    \apropout{5}{} \Par  
    \AmeliaMod{5}{\epsilon}{A'}_\empg  \Par 
    \highlighta{\binp{a_1}{y_1}} \binp{y_1}{z_1} \apropout{3}{z_1}
     \Par 
    %  \\
    % & 
     \propinp{3}{z_1} \binp{z_1}{x} \apropout{4}{x} \Par 
     \\
     &   
     \propinp{4}{x} \news{s} \big(\bout{x}{s} \about{\dual s}{w_1, w_2} \big) 
    \Par 
    % \\
    % &
    \news{s_1}\big(  \news{s''} \big(\highlighta{\bout{a_1}{s''}} 
    \bout{\dual{s''}}{s_1} \inact \big) \Par 
     \news{a_3} \big(\bout{s_1}{a_3} \big( \apropout{21}{} \Par 
    \\
    & 
    \qquad 
    \propinp{21}{} \inact \Par 
    \binp{a_3}{y_5} \binp{y_5}{x_1, x_2} \big(\apropout{17}{} 
    \Par \AmeliaMod{17}{\epsilon}{B'}_\empg \big) \big) \big) \big)  \big) \smallskip 
    \\ \bigskip & \quad \quad \text{where 
    $\widetilde c_* = (\prop_3, \dots, c_{12}, c_{17}, \dots, c_{25})$}
\end{align*}

  % \begin{align*}
  %     \F{P} &\red^{7} \news{\widetilde c_*}\news{a_1} ( \  
  %     \apropout{5}{} \Par  
  %     \AmeliaMod{5}{\epsilon}{A' }_\empg  \Par 
  %     \highlighta{\binp{a_1}{y_1}} \binp{y_1}{z_1} \apropout{3}{z_1} \Par \propinp{3}{z_1} \binp{z_1}{x} \apropout{4}{x} \Par \\
  %     & \quad \propinp{4}{x} \news{s} (\bout{x}{s} \about{\dual s}{w_1, w_2}) 
  %     \Par \news{s_1}\big(  \news{s''} (\highlighta{\bout{a_1}{s''}} \bout{\dual{s''}}{s_1} \inact) \Par \\
  %     & \quad  \news{a_3} (\bout{s_1}{a_3} \big( \apropout{21}{} \Par 
  %     \propinp{21}{} \inact \Par \binp{a_3}{y_5} \binp{y_5}{x_1, x_2} (\apropout{17}{} 
  %     \Par \AmeliaMod{17}{\epsilon}{B'}_\empg ) \big) ) \big) \ ) \smallskip 
  %     \\ \bigskip & \quad \quad \text{where 
  %     $\widetilde c_* = (\prop_3, \dots, c_{12}, c_{17}, \dots, c_{25})$}
  % \end{align*}

  \noindent 
  The next step involves communication on $a_1$: session name $s''$ is passed and substitutes variable $y_1$.

  \begin{align*}
    \F{P} &\red^{8} \news{\widetilde c_*} \news{s''} \big( \ 
    \apropout{5}{} \Par 
    \AmeliaMod{5}{\epsilon}{A'}_\empg       \Par 
    % \\
    % &
    \highlighta{ \binp{s''}{z_1}} \apropout{3}{z_1} \Par \propinp{3}{z_1} \binp{z_1}{x} \apropout{4}{x} \Par 
    \\
    &  
    \propinp{4}{x} \news{s} \big(\bout{x}{s} \about{\dual s}{w_1, w_2} \big) 
    \Par 
    % \\
    % &
 \news{s_1}\big(  \highlighta{\bout{\dual{s''}}{s_1}} \inact \Par 
    \news{a_3} \big(\bout{s_1}{a_3} \big( \apropout{21}{} \Par \propinp{21}{} \inact \Par \\
    & \quad \binp{a_3}{y_5} \binp{y_5}{x_1, x_2} \big( \ \apropout{17}{} \Par 
    \AmeliaMod{17}{\epsilon}{B' }_\empg  \big) \big) \big) \big) \big) \smallskip 
 %   \\ \bigskip & \quad \quad 
 %   \text{where $\wtd \prop = (\prop_3, \dots, \prop_{12}, \prop_{17}, \dots, \prop_{25})$}
\end{align*}

  % \begin{align*}
  %     \F{P} &\red^{8} \news{\widetilde c_*} \news{s''} ( \ 
  %     \apropout{5}{} \Par 
  %     \AmeliaMod{5}{\epsilon}{A'}_\empg \Par 
  %     \highlighta{ \binp{s''}{z_1}} \apropout{3}{z_1} \Par \propinp{3}{z_1} \binp{z_1}{x} \apropout{4}{x} \Par \\
  %     & \quad \propinp{4}{x} \news{s} (\bout{x}{s} \about{\dual s}{w_1, w_2}) 
  %     \Par \news{s_1}\big(  \highlighta{\bout{\dual{s''}}{s_1}} \inact \Par 
  %     \news{a_3} (\bout{s_1}{a_3} \big( \apropout{21}{} \Par \propinp{21}{} \inact \Par \\
  %     & \quad \binp{a_3}{y_5} \binp{y_5}{x_1, x_2} ( \ \apropout{17}{} \Par 
  %     \AmeliaMod{17}{\epsilon}{B' }_\empg \  ) \big) ) \big) \ ) \smallskip 
  %     % \\ \bigskip & \quad \quad 
  %     % \text{where $\wtd \prop = (\prop_3, \dots, \prop_{12}, \prop_{17}, \dots, \prop_{25})$}
  % \end{align*}

  \noindent 
  The process then synchronizes on channel $s''$. After $z_1$ is replaced by
  $s_1$, it is further sent to the next parallel process through the propagator
  $c_3$.
  \begin{align*}
    \F{P} &\red^{10} \news{\widetilde c_{**}} \news{s_1} \big( \ 
    \apropout{5}{} \Par
     \AmeliaMod{5}{\epsilon}{A' }_\empg 
    \Par 
    % \\
    % &
    \highlighta{\binp{s_1}{x}} \apropout{4}{x} \Par \propinp{4}{x} 
    \news{s} \big(\bout{x}{s} \about{\dual s}{w_1, w_2}\big)  \Par \\
    & \news{a_3} \big(\highlighta{\bout{s_1}{a_3}} \big( \apropout{21}{} 
    \Par \propinp{21}{} \inact \Par  
    \\
    & 
    \qquad 
    \binp{a_3}{y_5} \binp{y_5}{x_1, x_2} 
    \big(\apropout{17}{} \Par 
    \AmeliaMod{17}{\epsilon}{B'}_\empg \big) \big) \big)  \big)\smallskip 
    \\ \bigskip & \quad \quad \text{where 
    $\widetilde c_{**} = (\prop_4, \dots, \prop_{12}, \prop_{17}, \dots, \prop_{25})$}
\end{align*}

  % \begin{align*}
  %     \F{P} &\red^{10} \news{\widetilde c_{**}} \news{s_1} ( \ 
  %     \apropout{5}{} \Par
  %      \AmeliaMod{5}{\epsilon}{A'}_\empg 
  %     \Par 
  %     \highlighta{\binp{s_1}{x}} \apropout{4}{x} \Par \propinp{4}{x} 
  %     \news{s} (\bout{x}{s} \about{\dual s}{w_1, w_2})  \Par \\
  %     & \quad \news{a_3} (\highlighta{\bout{s_1}{a_3}} \big( \apropout{21}{} 
  %     \Par \propinp{21}{} \inact \Par  \binp{a_3}{y_5} \binp{y_5}{x_1, x_2} 
  %     (\apropout{17}{} \Par 
  %     \AmeliaMod{17}{\epsilon}{B'}_\empg ) \big) ) \ )\smallskip 
  %     \\ \bigskip & \quad \quad \text{where 
  %     $\widetilde c_{**} = (\prop_4, \dots, \prop_{12}, \prop_{17}, \dots, \prop_{25})$}
  % \end{align*}

  \noindent 
  Communication on $s_1$ leads to variable $x$ being substituted by name $a_3$,
  which is then passed on $c_{4}$ to the next process. In addition, inaction is
  simulated by synchronization on $\prop_{21}$.
  \begin{align*}
      \F{P} &\red^{13} \news{\widetilde c_{\bullet}} \news{a_3} ( \
      \apropout{5}{} \Par 
      \AmeliaMod{5}{\epsilon}{A' }_\empg \Par 
      \news{s} (
        \highlighta{\bout{a_3}{s}} \about{\dual s}{w_1, w_2})  \Par \\
      & \quad 
      \highlighta{\binp{a_3}{y_5}} \binp{y_5}{x_1, x_2} (\apropout{17}{} 
      \Par \AmeliaMod{17}{\epsilon}{B'  }_\empg ) \ ) \smallskip 
      \\ \bigskip & 
      \quad \quad \text{where $\widetilde c_{\bullet} = (\prop_5, \dots, c_{12}, c_{17}, \dots, c_{25})$}
  \end{align*}
  
  \noindent 
  Now, the distribution of the decomposition of $w$ from one process to another
  can finally be simulated by two reductions: first, a synchronization on $a_3$
  sends the endpoint of session $s$, which replaces variable $y_5$; afterwards,
  the dual endpoint is used to send the names $w_1,w_2$, substituting the
  variables $x_1,x_2$. 
  % Here, we remark that prefix $\abinp{s}{x_1,x_2}$ bounds 
  % variables $x_1,x_2$ in the breakdown of the continuation. 

  \begin{align*}
    \F{P} &\red^{14} \news{\widetilde c_{\bullet\bullet}} \news{s} ( \ 
    \apropout{5}{} \Par 
    \AmeliaMod{5}{\epsilon}{A' }_\empg 
    \Par \\
    & \qquad 
    \highlighta{\about{\dual s}{w_1, w_2}} \Par 
    \highlighta{\binp{s}{x_1, x_2}}
     \big(\apropout{17}{} \Par 
     \AmeliaMod{17}{\epsilon}{B' }_\empg \big)  \big) \smallskip 
 %   \\ \bigskip & \quad \quad \text{where 
    %$\widetilde c = (\prop_5, \dots, c_{12}, c_{17}, \dots, c_{25})$}
    \\
    %next reduction
     \F{P} &\red^{15} \news{\widetilde c_{\bullet\bullet}}\big( \ 
        \apropout{5}{} \Par \AmeliaMod{5}{\epsilon}{A' }_\empg \Par   
        \\
        &
        \qquad \apropout{17}{} \Par 
        \AmeliaMod{17}{\epsilon}{B'}_\empg \subst{w_1 w_2}{x_1 x_2}  \big) 
        = Q \smallskip 
      \\ \bigskip & \quad \quad \text{where 
      $\widetilde c_{\bullet \bullet} = (\prop_5, \dots, c_{12}, c_{17}, \dots, c_{25})$}
  \end{align*}

  \noindent 
  Here, we remark that as prefix $\abinp{s}{x_1,x_2}$ bounds 
  variables $x_1,x_2$ in the breakdown of the continuation 
  ($\AmeliaMod{17}{\epsilon}{B' }_\empg$). 
  Thus, there is no need for propagators to pass contexts: 
  propagators here only serve to enforce the ordering of actions. 
  On the other hand, this rely on arbitrary process nesting
  which is induced by the final application of encoding 
  $\map{\cdot}^2$ in the composition. 
   Thus the trio structure is lost. 
  % ( which is by the final application of encoding 
  % $\map{\cdot}^2$ in the composition.  )

  Undoubtedly, the first action of the original first-order process 
  has been simulated. We may notice that in $Q$ names $w_1$, $w_2$ substitute 
  $x_1$, $x_2$ and subsequent $\tau$-action on $w$ can be simulated on name $w_1$. 
  The following reductions follow the same pattern. 
  % Futher, we remark that prefix 
  % Undoubtedly, the behaviour of the initial first-order process has been 
  % simulated. 
  Thus, the outcome of our decomposition function is a functionally
  equivalent process that is typed with minimal session types.

\end{example}

  \smallskip

% \subsection{First Decomposition: Recursion}
% \label{app:ss:exrec}

% \input{example-am-rec}

\subsection{First Decomposition: Labelled Choice}
\label{app:ss:exsb}
% \label{pi:app:ss:exsb}
% Second Step Example
\noindent We now  illustrate how the approach in \Cref{pi:s:dbc} can be extended to account for labelled (deterministic) choice (selection and branching constructs).
In \HOp, these constructs are denoted
$$\bsel{u}{l} P \qquad \bbra{u}{l_i:P_i}_{i \in I}  $$
with reduction rule
$$
\bsel{n}{l_j} Q \Par \bbra{\dual{n}}{l_i : P_i}_{i \in I}  \red  Q \Par P_j ~~(j \in I)
$$

\begin{example}[First Decomposition: Labelled Choice]
%\emph{Example to be added}
\label{pi:ex:selbra-comp}
Let $P$ and $Q$ be \sessp processes which incorporate branching and selection:
\begin{align*}
	P = & ~\bbra{u}{l_1 : \news{h}(\bout{h}{m} \binp{h}{t} \inact \Par \binp{\dual{h}}{x} \bout{\dual h}{x} \inact), l_2 : \bout{s}{m} \binp{\dual{s}}{x} \inact } % = \bbra{u}{l_1: P_1, l_2 : P_2}$$
	\\
Q = & ~\bsel{\dual{u}}{l_1} \inact
\end{align*}

Let $R$ denote the restricted parallel composition of $P$ and $Q$: $R = \news{u}(P \Par Q)$. The respective process degrees have the same values as before.
\noindent The decomposition of $R$ is:
\begin{align*}
    \F{R} &= \news{c_1, \dots, c_5}(\propout{1}{} \inact \Par        \AmeliaMod{1}{\epsilon}{\news{u} (P \Par Q) \sigma}_g), \text{ where } \sigma = \subst{u_1 \dual{u_1}}{u \dual{u}}\\
                    &= \news{c_1, \dots, c_5}(\propout{1}{} \inact \Par \news{u_1} (\propinp{1}{} \propout{2}{} \apropbout{3}{} \Par \AmeliaMod{2}{\epsilon}{P}_g \Par \AmeliaMod{3}{\epsilon}{Q}_g))
\end{align*}
We consider $P$ and $Q$ separately. We begin with the breakdown of $Q$. 
\begin{align*}
% CHANGE THE INDEX OF a_1
    \AmeliaMod{3}{\epsilon}{Q}_g &= \propinp{3}{} \news{a_1} \big(\propout{4}{a_1} \big( \news{u_2} 
    \big( \propinp{4}{y} \news{s} \big(\bout{y}{s} \about{ \dual{s} }{ \dual u_2 } \big) \big) 
    \Par \propinp{5}{} \inact
        \Par \\ & \quad \binp{a_1}{y'} \binp{y'}{y_1} \bsel{u_1}{l_1} \binp{u_1}{z} \propout{5}{} 
        \news{s'} \big(\bout{z}{s'} \about{\dual s'}{y_1} \big) \big) \big)
\end{align*}
The breakdown of process $P$ is:
\begin{align*}
    \AmeliaMod{2}{\epsilon}{P}_g &= \propinp{2}{} \bbra{u_1}{l_1: \news{a_2} \bout{u_1}{a_2} \binp{a_2}{y''} 
    \binp{y''}{ y_1}  
    \news{c_3, \dots, c_{21}}\big( \apropout{3}{} \Par \AmeliaMod{3}{\epsilon}{P_1 \subst{y_1}{u_1}}_g \big),\\
    & \qquad \qquad \qquad  l_2 : \news{a_2} \bout{u_1}{a_2} \binp{a_2}{y''} \binp{y''}{y_1}   
    \news{c_3, \dots, c_{11}} \big( \apropout{3}{} \Par \AmeliaMod{3}{\epsilon}{P_2 \subst{y_1}{u_1}}_g \big)}
\end{align*}
As in the previous approach of this example, we are interested in the breakdown of $P_1$, because it belongs to the selected branch.
\begin{align*}
 \AmeliaMod{3}{\epsilon}{P_1 \subst{y_1}{u_1}}_g &= \news{h_1, h_2} 
        \AmeliaMod{3}{\epsilon}{\bout{h_1}{m_1} \binp{h_1}{t} \inact \Par \binp{\dual{h_1}}{x} \bout{\dual h_1}{x} \inact}_g\\
        &= \news{h_1, h_2} \big(\propinp{3}{} \propout{4}{} \apropout{13}{} 
        \Par \AmeliaMod{4}{\epsilon}{\bout{h_1}{m_1} \binp{h_1}{t} \inact}_g 
        \Par \AmeliaMod{13}{\epsilon}{\binp{\dual{h_1}}{x} \bout{\dual{ h_1}}{x} \inact}_g \big)
\end{align*}
\begin{align*}
    \AmeliaMod{4}{\epsilon}{\bout{h_1}{m_1}_g \binp{h_1}{t} \inact} &= 
      \propinp{4}{} \news{a_3} \big(\bout{h_1}{a_3} 
      \big( \apropout{7}{} \Par \AmeliaMod{7}{\epsilon}{\binp{h_2}{t} \inact}_g 
      \Par \binp{a_3}{y_2} \binp{y_2}{z_1} \apropout{5}{z_1} \Par \\
                    & \qquad \propinp{5}{z_1} \binp{z_1}{x} 
                    \apropbout{6}{x} \Par \propinp{6}{x} \news{s_1} 
                    \big(\bout{x}{s_1} \bout{ \dual{s_1} }{m_1} \inact ) \big) \big)\\
    \AmeliaMod{7}{\epsilon}{\binp{h_2}{t} \inact}_g &=  
                \propinp{7}{}\binp{h_2}{y_3} \apropout{8}{ y_3} \Par 
                \newsp{s_2} {\propinp{8}{y_3} \propout{9}{y_3} \apropout{10}{} \Par \\
               & \quad {} \propinp{9}{y_3} \news{s_3} \big(\bout{y_3}{s_3} \bout{\dual{s_3}}{s_2} \inact \big) 
               \Par \propinp{10}{} \news{a_4} \big(\bout{\dual{s_2}}{a_4} \big( \apropout{12}{} \Par \\
               & \quad  \propinp{12}{} \inact \Par \binp{a_4}{y_4} \binp{y_4}{t_1} 
               \apropout{11}{} \Par \propinp{11}{} \inact \  \big) }\\
    \AmeliaMod{13}{\epsilon}{\binp{\dual{h_1}}{x} \bout{\dual{ h_1}}{x} \inact}_g &= 
             \propinp{13}{}\binp{\dual{h_1}}{y_5} \apropout{14}{y_5} \Par \newsp{s_4} {\propinp{14}{y_5} \propout{15}{y_5} \apropout{16}{} \Par \\
               & \quad {} \propinp{15}{y_5} \news{s_5}\big(\bout{y_5}{s_5} \bout{\dual{s_5}}{s_4} \inact \big) 
               \Par \propinp{16}{} \news{a_5} \big(\bout{\dual{s_4}}{a_5} \big( \apropout{21}{} \Par \\
               & \quad  \propinp{21}{} \inact \Par 
               \binp{a_5}{y_6} \binp{y_6}{x_1} \apropout{17}{x_1} 
               \Par \AmeliaMod{17}{x_1}{ \bout{\dual{ h_2}}{x_1} \inact }_g  \ \big) \big) }\\
    \AmeliaMod{17}{x_1}{ \bout{\dual{ h_2}}{x_1} \inact }_g &= 
                    \propinp{17}{x_1} \news{a_6} \big(\bout{\dual{h_2}}{a_6} 
                    \big( \apropout{20}{x_1} \Par\propinp{20}{} \inact 
                    \Par \binp{a_6}{y_7} \binp{y_7}{z_2} \apropout{18}{z_2} \Par \\
                    & \qquad \propinp{18}{z_2} \binp{z_2}{x'} \apropbout{19}{x'} 
                    \Par \propinp{19}{x'} \news{s_6} (\bout{x'}{s_6} \bout{ \dual{s_6} }{x_1} \inact \big) \big) \big)
\end{align*}
In order to verify that the decomposition of $R$ simulates the behaviour of the initial process, we refer to its reduction chain. The first transitions involve synchronization on $c_1, c_2, c_3$ and $c_4$. The trigger name $a_2$ is passed through propagator $c_4$, such that it replaces variable $y$.
\begin{align*}
    \F{R} &\red^4 \news{c_5} \news{u_1} \big(\bbra{u_1}{l_1: \news{a_2} \ 
    \bout{u_1}{a_2} \binp{a_2}{y''} \binp{y''}{ y_1}  
    \news{c_3, \dots, c_{21}}\big( \apropout{3}{} \Par \\
    &  \qquad \AmeliaMod{3}{\epsilon}{P_1 \subst{y_1}{u_1}}_g ), \ l_2 : \news{a_2} \ \bout{u_1}{a_2} \binp{a_2}{y''} \binp{y''}{y_1}   
      \news{c_3, \dots, c_{11}}\big( \apropout{3}{} \Par\\
       &  \qquad \AmeliaMod{3}{\epsilon}{P_2 \subst{y_1}{u_1}}_g )} \Par \news{a_1} \big( \news{u_2} 
       \big( \news{s} \big(\bout{a_1}{s} \about{ \dual{s} }{ \dual u_2 } \big) \big) \Par \propinp{5}{} \inact
        \Par \\ & \qquad \binp{a_1}{y'} \binp{y'}{y_1} \bsel{u_1}{l_1} \binp{u_1}{z} \propout{5}{} \news{s'} 
        \big(\bout{z}{s'} \about{\dual s'}{y_1} \big) \big)  ) 
\end{align*}
The next step involves synchronization on $a_1$, which leads to the variable $y'$ being substituted by session name $s$.
\begin{align*}
    \F{R} &\red^5 \news{c_5} \news{u_1} \big(\bbra{u_1}{l_1: \news{a_2} \ 
    \bout{u_1}{a_2} \binp{a_2}{y''} \binp{y''}{ y_1}  
    \news{c_3, \dots, c_{21}} \big( \apropout{3}{} \Par \\
    &  \qquad \AmeliaMod{3}{\epsilon}{P_1 \subst{y_1}{u_1}}_g ), \ l_2 : \news{a_2} \ \bout{u_1}{a_2} \binp{a_2}{y''} \binp{y''}{y_1}   
      \news{c_3, \dots, c_{11}} \big( \apropout{3}{} \Par\\
       &  \qquad \AmeliaMod{3}{\epsilon}{P_2 \subst{y_1}{u_1}}_g \big)} \Par \news{s} \big( \news{u_2} 
       \big(   \about{ \dual{s} }{ \dual u_2 }  \big) \Par \propinp{5}{} \inact
        \Par \\ & \qquad  \binp{s}{y_1} \bsel{u_1}{l_1} \binp{u_1}{z} \propout{5}{} \news{s'} 
        \big(\bout{z}{s'} \about{\dual s'}{y_1} \big) \big)  \big) 
\end{align*}
Now, session name $s$ and its dual endpoint can communicate - channel name $\dual{u_2}$ is sent, replacing $y_1$.
\begin{align*}
    \F{R} &\red^6 \news{c_5} \news{u_1} \big(\bbra{u_1}{l_1: \news{a_2} \ 
    \bout{u_1}{a_2} \binp{a_2}{y''} \binp{y''}{ y_1}  
    \news{c_3, \dots, c_{21}} \big( \apropout{3}{} \Par \\
    &  \qquad \AmeliaMod{3}{\epsilon}{P_1 \subst{y_1}{u_1}}_g ), \ l_2 : \news{a_2} \ \bout{u_1}{a_2} \binp{a_2}{y''} \binp{y''}{y_1}   
      \news{c_3, \dots, c_{11}} \big( \apropout{3}{} \Par\\
       &  \qquad \AmeliaMod{3}{\epsilon}{P_2 \subst{y_1}{u_1}}_g \big)} \Par \news{u_2} \big(\propinp{5}{} \inact
        \Par  \bsel{u_1}{l_1} \binp{u_1}{z} \propout{5}{} \news{s'} \big(\bout{z}{s'} \about{\dual s'}{\dual{u_2}} 
        \big) \big)  \big) 
\end{align*}
At this point, the action of choosing the first branch can be simulated by selecting label $l_1$ on channel name $u_1$.
\begin{align*}
    \F{R} &\red^7 \news{c_5} \news{u_1} \big( \news{a_2} \ \bout{u_1}{a_2} \binp{a_2}{y''} \binp{y''}{ y_1}  
    \news{c_3, \dots, c_{21}}( \apropout{3}{} \Par \\
    &  \qquad \AmeliaMod{3}{\epsilon}{P_1 \subst{y_1}{u_1}}_g ) \Par \news{u_2} \big(\propinp{5}{} \inact
        \Par \binp{u_1}{z} \propout{5}{} \news{s'} \big(\bout{z}{s'} \about{\dual s'}{\dual{u_2}} \big) \big)  ) 
\end{align*}
The following two reductions consist of synchronizations on $u_1$ and $c_5$. As a result, variable $z$ is replaced by the trigger name $a_2$.
\begin{align*}
    \F{R} &\red^9 \news{a_2} \big(\binp{a_2}{y''} \binp{y''}{ y_1}  
    \news{c_3, \dots, c_{21}} \big( \apropout{3}{} \Par \\
    &  \qquad \AmeliaMod{3}{\epsilon}{P_1 \subst{y_1}{u_1}}_g \big) \Par \news{u_2} 
    \big( \news{s'} \big(\bout{a_2}{s'} \about{\dual s'}{\dual{u_2}} \big) \big)  ) 
\end{align*}
Communication on $a_2$ allows for synchronization on $s'$. Channel $a_2$ receives the session name $s'$, which further receives the dual endpoint $\dual{u_2}$.
\begin{align*}
    \F{R} &\red^{11} \news{c_3, \dots, c_{21}} \news{u_2} \big( \apropout{3}{} 
    \Par \AmeliaMod{3}{\epsilon}{P_1 \subst{\dual{u_2}}{u_1}}_g \big) \\
                    &= \news{c_3, \dots, c_{21}} \news{u_2} \big( \apropout{3}{} \Par \news{h_1, h_2} 
                    \big(\propinp{3}{} \propout{4}{} \apropout{13}{} \Par \\ & \quad 
                    \AmeliaMod{4}{\epsilon}{\bout{h_1}{m_1} \binp{h_1}{t} \inact}_g \Par 
                    \AmeliaMod{13}{\epsilon}{\binp{\dual{h_1}}{x} \bout{\dual{ h_1}}{x} \inact}_g \big)  \big)
\end{align*}
Remarkably, the obtained result reflects the broken down version of process
$P_1$. Following three more reductions, in which $c_3, c_4$ and $c_{13}$
synchronize with their respective duals, the breakdown of each parallel
sub-process will be activated. We refrain from presenting the remaining
reduction steps, as they represent a standard case of name-passing. Clearly, the
decomposed process $\F{R}$ behaves in a similar manner to the initial process
$R$.
\end{example}

\newpage

\section{Relevant notions from~\cite{DBLP:journals/iandc/KouzapasPY19}}
\label{app:relexp}

\subsection{Session Types for \HOp} \label{app:typing}
\input{type_system}

\subsection{Labelled Transition System for \HOp}

%%%%%%%%%%%%%%%%%%%% LTS Figure %%%%%%%%%%%%%%%%%%%%%%%%%%%%%%%%%%%%%
\begin{figure}[h]
  \begin{mdframed}
	\begin{mathpar}
		\inferrule[\ltsrule{App}]{
		}{
			\appl{(\abs{x}{P})}{V} \by{\tau} P \subst{V}{x}
		}
		\and
		\inferrule[\ltsrule{Snd}]{
		}{
			\bout{n}{V} P \by{\bactout{n}{V}} P
		}
		\and
		\inferrule[\ltsrule{Rv}]{
		}{
			\binp{n}{x} P \by{\bactinp{n}{V}} P\subst{V}{x}
		}
		\and
		\inferrule[\ltsrule{Sel}]{
		}{
			\bsel{s}{l}{P} \by{\bactsel{s}{l}} P
		}
		\and
		\inferrule[\ltsrule{Bra}]{j\in I
		}{
			\bbra{s}{l_i:P_i}_{i \in I} \by{\bactbra{s}{l_j}} P_j 
		}
		\and
		\inferrule[\ltsrule{Alpha}]{
			P \scong_\alpha Q
			\and
			Q\by{\ell} P'
		}{
			P \by{\ell} P'
		}
		\and
		\inferrule[\ltsrule{Res}]{
			P \by{\ell} P'
			\and
			n \notin \fn{\ell}
		}{
			\news{n} P \by{\ell} \news{n} P'
		}
		\and
		\inferrule[\ltsrule{New}]{
			P \by{\news{\widetilde{m}} \bactout{n}{V}} P'
			\and
			m_1 \in \fn{V}
		}{
			\news{m_1} P \by{\news{m_1\cat\widetilde{m}} \bactout{n}{V}} P'
		}
		\and
		\inferrule[\ltsrule{Par${}_L$}]{
			P \by{\ell} P'
			\and
			\bn{\ell} \cap \fn{Q} = \es
		}{
			P \Par Q \by{\ell} P' \Par Q
		}
		\and
		\inferrule[\ltsrule{Tau}]{
			P \by{\ell_1} P'
			\and
			Q \by{\ell_2} Q'
			\and
			\ell_1 \asymp \ell_2
		}{
			P \Par Q \by{\tau} \newsp{\bn{\ell_1} \cup \bn{\ell_2}}{P' \Par Q'}
		}
		\and
		\inferrule[\ltsrule{Rec}]{
			P\subst{\recp{X}{P}}{\rvar{X}} \by{\ell} P'
		}{
			\recp{X}{P}  \by{\ell} P'
		}
	\end{mathpar}
	\caption{The Untyped LTS for \HOp processes. We omit Rule $\ltsrule{Par${}_R$}$.  
  \label{fig:untyped_LTS}}
\end{mdframed}
\end{figure}

%%%%%%%%%%%%%%%%%%%% End LTS Figure %%%%%%%%%%%%%%%%%%%%%%%%%%%%%%%%%

%%%%%%%%%%%%%%%%%%%% Environment LTS Figure %%%%%%%%%%%%%%%%%%%%%%%%%
\begin{figure}[h]
  \begin{mdframed}
  \begin{mathpar}
    \inferrule[\eltsrule{SRv}]{
      \dual{s} \notin \dom{\Delta}
      \and
      \Gamma; \Lambda'; \Delta' \proves V \hastype U
    }{
      (\Gamma; \Lambda; \Delta \cat s: \btinp{U} S) \by{\bactinp{s}{V}} (\Gamma; \Lambda\cat\Lambda'; \Delta\cat\Delta' \cat s: S)
    }
    \and
    \inferrule[\eltsrule{ShRv}]{
      \Gamma; \es; \es \proves a \hastype \chtype{U}
      \and
      \Gamma; \Lambda'; \Delta' \proves V \hastype U
    }{
      (\Gamma; \Lambda; \Delta) \by{\bactinp{a}{{V}}} (\Gamma; \Lambda\cat\Lambda'; \Delta\cat\Delta')
    }
    \and
    \inferrule[\eltsrule{SSnd}]{
      \begin{array}{l}
        \Gamma \cat \Gamma'; \Lambda'; \Delta' \proves V \hastype U
        \and
        \Gamma'; \es; \Delta_j \proves m_j  \hastype U_j
        \and
        \dual{s} \notin \dom{\Delta}
        \\
        \Delta'\backslash (\cup_j \Delta_j) \subseteq (\Delta \cat s: S)
        \and
        \Gamma'; \es; \Delta_j' \proves \dual{m}_j  \hastype U_j'
        \and
        \Lambda' \subseteq \Lambda
      \end{array}
    }{
      (\Gamma; \Lambda; \Delta \cat s: \btout{U} S)
      \by{\news{\widetilde{m}} \bactout{s}{V}}
      (\Gamma \cat \Gamma'; \Lambda\backslash\Lambda'; (\Delta \cat s: S \cat \cup_j \Delta_j') \backslash \Delta')
    }
    \and
    \inferrule[\eltsrule{ShSnd}]{
      \begin{array}{l}
        \Gamma \cat \Gamma' ; \Lambda'; \Delta' \proves V \hastype U
        \and
        \Gamma'; \es; \Delta_j \proves m_j \hastype U_j
        \and
        \Gamma ; \es ; \es \proves a \hastype \chtype{U}
        \\
        \Delta'\backslash (\cup_j \Delta_j) \subseteq \Delta
        \and
        \Gamma'; \es; \Delta_j' \proves \dual{m}_j\hastype U_j'
        \and
        \Lambda' \subseteq \Lambda
      \end{array}
    }{
      (\Gamma ; \Lambda; \Delta) \by{\news{\widetilde{m}}
      \bactout{a}{V}}
      (\Gamma \cat \Gamma'; \Lambda\backslash\Lambda'; (\Delta \cat \cup_j \Delta_j') \backslash \Delta')
    }
    \and
    \inferrule[\eltsrule{Sel}]{
      \dual{s} \notin \dom{\Delta}
      \and
      j \in I
    }{
      (\Gamma; \Lambda; \Delta \cat s: \btsel{l_i: S_i}_{i \in I}) \by{\bactsel{s}{l_j}} (\Gamma; \Lambda; \Delta \cat s:S_j)
    }
    \and
    \inferrule[\eltsrule{Bra}]{
      \dual{s} \notin \dom{\Delta} \quad j \in I
    }{
      (\Gamma; \Lambda; \Delta \cat s: \btbra{l_i: T_i}_{i \in I}) \by{\bactbra{s}{l_j}} (\Gamma; \Lambda; \Delta \cat s:S_j)
    }
    \and
    \inferrule[\eltsrule{Tau}]{
      \Delta_1 \red \Delta_2 \vee \Delta_1 = \Delta_2
    }{
      (\Gamma; \Lambda; \Delta_1) \by{\tau} (\Gamma; \Lambda; \Delta_2)
    }
  \end{mathpar}
  \caption{Labelled Transition System for Typed Environments. 
  \label{fig:envLTS}}
\end{mdframed}
  \end{figure}

  %%%%%%%%%%%%%%%%%%%% End Environment LTS Figure %%%%%%%%%%%%%%%%%%%%%%

\noi
The typed LTS  combines
the LTSs in \figref{fig:untyped_LTS}
and \figref{fig:envLTS}. 

\begin{definition}[Typed Transition System]
	\label{d:tlts}
	A {\em typed transition relation} is a typed relation
	$\horel{\Gamma}{\Delta_1}{P_1}{\by{\ell}}{\Delta_2}{P_2}$
	where:
	\begin{enumerate}
		\item
				$P_1 \by{\ell} P_2$ and 
		\item
				$(\Gamma, \emptyset, \Delta_1) \by{\ell} (\Gamma, \emptyset, \Delta_2)$ 
				with $\Gamma; \emptyset; \Delta_i \proves P_i \hastype \Proc$ ($i=1,2$).
%				\dk{We sometimes annotated the output action with
%				the type of value $V$ as in $\widetilde{m} \bactout{n}{V: U}$.}
	\end{enumerate}
	We 
	%extend to $\By{}$ and $\By{\hat{\ell}}$  where we 
	write  $\By{}$ for the reflexive and transitive closure of $\by{}$,
	$\By{\ell}$ for the transitions $\By{}\by{\ell}\By{}$, and $\By{\hat{\ell}}$
	for $\By{\ell}$ if $\ell\not = \tau$ otherwise $\By{}$.
\end{definition}

In this section we recall  relevant notions from ~\cite{DBLP:journals/iandc/KouzapasPY19}. 

\subsection{Encoding of \HOp into \HO}

\begin{figure}[h!]
  \begin{mdframed}
	\begin{align*}
		\auxmapp{\bout{w}{\abs{x}{Q}} P}{{}}{\sigma} & \defeq \bout{u}{\abs{x}{\auxmapp{Q}{{}}{{\sigma \cat x}}}} \auxmapp{P}{{}}{\sigma}
		&
		\auxmapp{\bbra{w}{l_i:P_i}_{i \in I}}{{}}{\sigma} & \defeq \bbra{u}{l_i:\auxmapp{P_i}{{}}{\sigma}}_{i \in I}		
		\\
		\auxmapp{\binp{w}{x} P}{{}}{\sigma} & \defeq \binp{u}{x} \auxmapp{P}{{}}{\sigma} 
		&
		\auxmapp{\bsel{w}{l} P}{{}}{\sigma} & \defeq \bsel{u}{l} \auxmapp{P}{{}}{\sigma} 
		\\
		\auxmapp{\news{n} P}{{}}{\sigma} & \defeq \news{n} \auxmapp{P}{{}}{{\sigma \cat n}}
		&
		\auxmapp{\appl{(\lambda x.Q)}{w}}{{}}{\sigma}  & \defeq \appl{(\lambda x.\auxmapp{Q}{{}}{{\sigma \cat x}})}{u}
		\\
		\auxmapp{P \Par Q}{{}}{\sigma} & \defeq \auxmapp{P}{{}}{\sigma} \Par \auxmapp{Q}{{}}{\sigma} 
		&
		\auxmapp{\appl{x}{w}}{{}}{\sigma} & \defeq \appl{x}{u}
		\\
		\auxmapp{\inact}{{}}{\sigma}  & \defeq  \inact	
		& 
\end{align*}
\begin{center}
	{In all cases: $u = 
	\begin{cases} 
	x_n & \text{if $w$ is a name $n$ and  $n \not\in \sigma$ ($x$ fresh)}
	\\
	w & \text{otherwise: $w$ is a variable or a name $n$ and $n \in \sigma$} 
	 	\end{cases}$}
\end{center}
\end{mdframed}
%\vspace{-3mm}
\caption{\label{f:auxmap} Auxiliary mapping used to encode \HOp into \HO (\defref{d:auxmap}).}
%\vspace{-1mm}
%\Hlinefig 
\end{figure}

\begin{definition}[Auxiliary Mappings] \label{d:trabs}
  \label{d:auxmap}
  We define mappings $\vmap{\cdot}$ and $\auxmapp{\cdot}{{}}{\sigma}$ as follows:
  \begin{itemize}
  \item  $\vmap{\cdot}: 2^{\mathcal{N}} \longrightarrow \mathcal{V}^\omega$
    is a map of sequences of lexicographically ordered names to sequences of variables, defined
    inductively 
    as: 
    \begin{align*}
    \vmap{\epsilon} & = \epsilon 
    \\
    \vmap{n \cat \tilde{m}} & = x_n \cat \vmap{\tilde{m}} \quad \text{($x$ fresh)}
    \end{align*}
  
  \item Given a set of session names and variables $\sigma$, 
     the   map
    $\auxmapp{\cdot}{{}}{\sigma}: \HO \to \HO$
    is as in \figref{f:auxmap}.
    \end{itemize}
  \end{definition}

\newpage
\section{Proofs}

\subsection{Auxiliary Results}

\begin{restatable}[Substitution Lemma]{lemm}{lemsubst}
  \label{lem:subst}
  $\Gamma;\Delta \cat x:S \proves P \hastype \Proc$ and 
  $u \notin \dom{\Gamma,\Delta}$ implies 
  $\Gamma; \Delta \cat u:S \proves P\subst{u}{x} \hastype \Proc$.
  \end{restatable}
  
  The following property follows immediately from 
  \defref{def:typesdecomp} and 
  \defref{def:typesdecompenv}:
  
  \begin{restatable}[Typing Broken-down Variables]{lemm}{lemvarbreak}
  \label{lem:varbreak}
    If $\Gamma;\Delta \proves z_i \hastype C$ then 
    $\Gt{\Gamma};\Gt{\Delta} \proves \wtd z \hastype \Gt{C}$ 
    where $\wtd z = (z_i,\ldots,z_{i + \len{\Gt{C}} - 1})$.
  \end{restatable}

  \begin{restatable}[Shared environment weakening]{lemm}{lemweaken}
    \label{lem:weaken}
    If $\Gamma;\Delta \proves P \hastype \Proc$
    then
    $\Gamma \cat u:\chtype{C}; \Delta \proves P \hastype \Proc$.
  \end{restatable}
  
  \begin{restatable}[Shared environment strengthening]{lemm}{lemstrength}
    \label{lem:strength}
    If $\Gamma;\Delta \proves P \hastype \Proc$ and
    $u \notin \fn{P}$ then $\Gamma \setminus u;\Delta \proves P \hastype \Proc$.
  \end{restatable}

\begin{restatable}[]{lemm}{}
	\label{lem:indexcor}
	Let $\widetilde r$ be tuple of channel names and $S$ a recursive 	session type.
	If $\widetilde r : \Rtsopt{}{s}{\btout{C}S}$ and $k = f(\btout{C}S)$
	then $r_k:\trec{t}\btout{\Gt{C}}\vart{t}$.
\end{restatable}

\subsection{Decompose by Composition}

  \thmamtyprec* 

  \begin{proof}
    \label{app:thmamtyprec}
    \begin{align}
        \Gamma; \Delta, \envR &\proves P \hastype \Proc & &( \text{Assumption}) \\
        \tmap{\Gamma}{1}; \tmap{\Delta}{1}, \tmap{\envR}{1} 
        &\proves \map{P}^1_g \hastype \Proc 
        & &(\text{Theorem 5.1 \cite{DBLP:journals/iandc/KouzapasPY19}, (10)}) \\
        \Gt{\tmap{\Gamma}{1}}, \Phi; \ 
        \Gt{\tmap{\Delta}{1}}, \Theta &\proves \B{k}{\epsilon}{ \map{P}^1_g } 
        \hastype \Proc & &( \text{Theorem 3.27 \cite{APV19}, (11)}) \\
        \map{ \Gt{\tmap{\Gamma}{1}} }^2, \map{\Phi}^2 ; 
        \map{ \Gt{\tmap{\Delta}{1}} }^2, \ \map{\Theta}^2 &\proves 
        \map{\B{k}{\epsilon}{\map{P}^1_g}}^2 \hastype \Proc 
        & &(\text{Theorem 5.2 \cite{DBLP:journals/iandc/KouzapasPY19}, (12)}) \\
        \mGt{\Gamma}, \Phi'; \mGt{\Delta}, \Theta' 
        &\proves \AmeliaMod{k}{\epsilon}{P}_g \hastype \Proc 
        & &(\text{ Definition of } \AmeliaMod{k}{\epsilon}{\cdot}_g,\\
        & & &\text{Definition \ref{decomp:firstordertypes}, 
        Definition \ref{ThetaPrimeDef}, (4)}) \nonumber 
    \end{align}
\end{proof}

\thmamtyprecdec*

\begin{proof}
  \label{app:thmamtyprecdec}
  \begin{align}
       \Gamma; \Delta &\proves P \hastype \Proc & &( \text{Assumption}) \\
       \Gamma \sigma; \Delta \sigma &\proves P \sigma \hastype \Proc 
       & &( \text{Lemma \ref{lem:subst}, (6)}) \\
       \mGt{\Gamma \sigma} \cat \Phi'; \mGt{\Delta \sigma}, \Theta' 
       &\proves \AmeliaMod{k}{\epsilon}{P \sigma}_g \hastype \Proc 
       & &( \text{P is initialized, Theorem \ref{t:am-typ-rec}})
       \label{eq:am-dec-rec1}
  \end{align}

% By \thmref{t:decompcore} we have that: 

% We shall show the following: 

% $$\mGt{\Gamma \sigma}; \mGt{\Delta \sigma}
%       \cat \mGt{\envR\sigma} \proves 
%       \news{\widetilde \prop}
%     \news{\widetilde \prop_r}
%     \big(
%       \prod_{r \in \tilde{v} } P^r \Par   
%     \propout{k}{} \inact 
%     \Par \AmeliaMod{k}{\epsilon}{P\sigma}_g \big)$$

  To complete the proof, let us construct a well-formed derivation tree 
  by using the appropriate typing rules for the higher-order calculus. 
  Note that we apply one of the polyadic rules, i.e. PolyResS, used for typing \HOp, 
  derived by Arslanagi\'{c} et al.~\cite{APV19}.

  \begin{align}
    \AxiomC{for $r \in \widetilde v$} 
    \AxiomC{$
            \mGt{\Gamma \sigma} \cat \Phi'; \wtd r : \mGt{S} 
           \proves  \proprinp{r}{b}\news{s}(\bout{b}{s}\about{\dual s}{\wtd r}) 
           \hastype \Proc$} 
    \LeftLabel{\scriptsize Par ($\len{\widetilde v}-1$ times)}
    \BinaryInfC{$\mGt{\Gamma \sigma} \cat \Phi'; 
    \mGt{\Delta_\mu \sigma}
     \proves
     \prod_{r \in \tilde{v} } P^r$} 
    \DisplayProof
    \label{pt:am-dec-rec2}
  \end{align}
  \noindent where $S = \envR(r)$. 
  By the definition of $\Phi'$ we have 
  $c^r:\chtype{\chtype{\btinp{\mRts{}{}{\envR(r)}}\tinact}} \in \Phi'$ 
  and by  \defref{decomp:firstordertypes} we have $\mRts{}{}{\envR(r)} = \mGt{S}$, 
   so the right-hand of \eqref{pt:am-dec-rec2} is well-typed.

  \begin{align}
    \AxiomC{} 
    \LeftLabel{\scriptsize Nil}
    \UnaryInfC{$
    \mGt{\Gamma \sigma} \cat \Phi'; 
      \mGt{\Delta \sigma} 
       \proves \inact \hastype \Proc$}
    \LeftLabel{\scriptsize Send}
    \UnaryInfC{$
      \mGt{\Gamma \sigma} \cat \Phi'; 
      \mGt{\Delta \sigma}, \apropout{k}{\cdot};
      \tinact \proves\apropout{k}{\cdot}
    $} 
    \AxiomC{\eqref{pt:am-dec-rec2}} 
    \LeftLabel{\scriptsize Par}
    \BinaryInfC{ $\mGt{\Gamma \sigma} \cat \Phi'; 
    \mGt{\Delta \sigma} \cat \mGt{\Delta_\mu \sigma} 
    \cat \apropout{k}{\cdot};
     \tinact \proves
     \propout{k}{\cdot}
      \inact \Par 
      \prod_{r \in \tilde{v} } P^r$}
      \DisplayProof
      \label{pt:am-dec-rec1}
  \end{align}
  
  \begin{align*}
    \AxiomC{
     \eqref{pt:am-dec-rec1}
    } 
    \AxiomC{\eqref{eq:am-dec-rec1}}
    \LeftLabel{\scriptsize Par}
    \BinaryInfC{
      $\mGt{\Gamma \sigma} \cat \Phi'; 
      \mGt{\Delta \sigma} \cat  \mGt{\envR\sigma} \cat \apropout{k}{\cdot};
       \tinact, \Theta' \proves \propout{k}{\cdot}
        \inact \Par 
        \prod_{r \in \tilde{v} } P^r \Par  
        \AmeliaMod{k}{\epsilon}{P \sigma}_g \hastype \Proc$
    } 
    \LeftLabel{\scriptsize PolyResS}
    \UnaryInfC{
      $\mGt{\Gamma \sigma}; \mGt{\Delta \sigma}
      \cat \mGt{\envR\sigma} \proves 
      \news{\widetilde \prop}
    \news{\widetilde \prop_r}
    \big(
      \prod_{r \in \tilde{v} } P^r \Par   
    \propout{k}{} \inact 
    \Par \AmeliaMod{k}{\epsilon}{P\sigma}_g \big)
      $
    }
    \DisplayProof 
  \end{align*}

\end{proof}

\subsection{Measuring the Optimization}
\label{app:propopt}
\propopt* 

\begin{proof}%(Sketch)
  \label{p:propopt}
  Because $\numpropam{Q} \geq
     \lenHO{P} + 2 \cdot \len{\lentr{P}}$, it suffices to show that 
     $\lenHO{P} + 2 \cdot \len{\lentr{P}} \geq \frac{5}{3} \cdot \numprop{P}$.
     The proof is by induction on structure of $P$. We show one base case (output prefix followed by 
     inaction) and
     three inductive cases (input, restriction, and parallel composition); other
     cases are similar:
       \begin{itemize}
         \item Case $P = \bout{u}{x}\inact$. Then 
          $\lenHO{P} = 4$, $\len{\lentr{P}} = 0$, and $\lenHOopt{P} = 2$. 
        So, we have $\lenHO{P} + 2 \cdot \len{\lentr{P}} \geq \frac{5}{3} \cdot \numprop{P}$
  
         \item Case $P = \bout{u}{x}P'$ with $P' \not\equiv \inact$.
         By IH we know $\lenHO{P'} + \lentr{P'} \geq \frac{5}{3} \cdot \numprop{P'}$.
         We know $\lenHO{P} = \lenHO{P'} + 3$ 
         , $\lenHOopt{P} = \lenHOopt{P'} + 1$ and $\lenrecpx{P} = \lenrecpx{P'}$. 
         So,  
         $\lenHO{P'} + 2 \cdot \len{\lentr{P'}} + 3 \geq \frac{5}{3} \cdot \numprop{P} + 1 
         > \frac{5}{3}\cdot(\numprop{P} + 1)$. 
   
         \item  Case $P = \news{r:S}P'$ with  $\tr(S)$. 
       Then $\lenHO{P} = \lenHO{P'}$ (by \defref{def:am-sizeproc})
       and  $\len{\lentr{P}} = \len{\lentr{P'}} + 1$. 
       Further, we have $\lenrecpx{P} = \lenrecpx{P'}$ and $\lenHOopt{P} = \lenHOopt{P'} +
       1$. 
  %      (by \defref{def:sizeproc}).
       Now, by IH 
  %      we have  $\lenHO{Q} + \lentr{Q} > \numprop{Q}$. So, 
      we can
       conclude that $\lenHO{P} + 2 \cdot (\len{\lentr{P}} + 1)  \geq 
        \frac{5}{3} \cdot \numprop{P} + 1
       > \frac{5}{3} \cdot (\numprop{P} + 1)$.
  
       \item Case $P = P_1 \Par \ldots \Par P_n$. 
       By IH we know 
       \begin{align}
          \lenHO{P_i} + 2 \cdot \len{\lentr{P_i}} \geq \frac{5}{3} \cdot \numprop{P_i}
          \label{eq:optproof-1}
       \end{align}
      %  $$\lenHO{Q_i} + 2 \cdot \lentr{Q_i} \geq \frac{5}{3} \cdot \numprop{Q_i}$$ 
       \noindent for $i \in \{1,\ldots,n\}$. 
       We know 
       $\lenHO{P} = \sum_{i=1}^{n} \lenHO{P_i} + (n-1)$, 
       $\len{\lentr{P}} = \sum_{i=1}^{n} \len{\lentr{P_i}}$,  
       and $\lenHOopt{P} = \sum_{i=1}^{n}\numprop{P_i} + (n-1)$.
       So, we should show 
       \begin{align}
         \sum_{i=1}^{n} \lenHO{P_i} + 2 \cdot \sum_{i=1}^{n} \len{\lentr{P_i}}
         + (n-1) \geq 
         \frac{5}{3} \cdot \big(\sum_{i=1}^{n}\numprop{P_i} + (n-1)\big)
         \label{eq:measure-prop1}
       \end{align}
       % $$\sum_{i=1}^{n} \lenHO{Q_i} + (n-1) \geq k \cdot \big(\sum_{i=1}^{n}\lenHOopt{Q_i} + (n-1)\big)$$
  
       That is, 
       $$\sum_{i=1}^{n} (\lenHO{P_i} + 2 \cdot \len{\lentr{P_i}} + 1) \geq 
       \frac{5}{3} \cdot \sum_{i=1}^{n} \big(\numprop{P_i} + 1\big)$$
  
       Equivalent to 
       $$\sum_{i=1}^{n} (\lenHO{P_i} + 2 \cdot \len{\lentr{P_i}} + 1) \geq 
       \sum_{i=1}^{n} \big(\frac{5}{3} \cdot (\numprop{P_i} + 1)\big)$$
  
       We show that for each $i = \{1, \ldots, n\}$ the following holds:  
       $$\lenHO{P_i} + 2 \cdot \len{\lentr{P_i}} + 1 \geq  \frac{5}{3} \cdot (\numprop{P_i} + 1)$$ 
  
       That is 
       $$A = \frac{\lenHO{P_i} + 2 \cdot \len{\lentr{P_i}} + 1}{\numprop{P_i} + 1} \geq  \frac{5}{3}$$ 
  
      %  That is we need to detect $Q_i$ for which $\frac{\lenHO{Q_i} + 2 \cdot \lentr{Q_i}}{\lenHOopt{Q_i}}$
      %  is the least.
        As $P$ is in the normal form, 
       we know that $P_i \equiv \alpha.P_i'$
       where $\alpha$ is some sequential prefix. So,
       by \defref{def:am-sizeproc} and $\defref{def:sizeproc}$ we know that 
      for some $p^*$ and $p$ we have 
       $\lenHOopt{P_i} = p^* + \lenHOopt{P_i'}$, $\lenrecpx{P_i} = \lenrecpx{P_i'}$, 
       and $\lenHO{P_i} = p + \lenHO{P_i'}$. 
       We can distinguish two sub-cases: \rom{1} $P'_i \not\equiv \inact$ 
       and \rom{2} otherwise. 
       We consider sub-case \rom{1}. 
       By \eqref{eq:optproof-1} we have: 
       $$A \geq \frac{\frac{5}{3}\cdot \numprop{P'_i} + p + 1}{\numprop{P'_i} + p^* + 1} \geq  \frac{5}{3}$$ 
  
       We need to find prefix $\alpha$ such that $p$ and $\frac{p}{p^*}$ are the least. 
       We notice that for 
       the output prefix we have $p = 3$ and $\frac{p}{p^*} = \frac{3}{1}$. 
       So, the following holds 
       $$\frac{\frac{5}{3}\cdot \numprop{P'_i} + 4}{\numprop{P'_i} + 2} = 
       \frac{5}{3} \cdot \frac{\numprop{P'_i} + \frac{12}{5}}{\numprop{P'_i} + 2} \geq  \frac{5}{3}$$ 
  
       Now, we consider sub-case \rom{2} when $P'_i = \inact$. 
      %  We may notice that this term $A$ is the least when $Q'_i  = \inact$. 
       In this case we have $\lenHO{P'_i} + 2 \cdot \lentr{P_i'}= \numprop{P'_i} = 1$. 
       We pick $p$ and $p^*$ as in the previous sub-case. 
       So, we have 
       $$\frac{\lenHO{P_i} + 2 \cdot \len{\lentr{P_i}} + 1}{\numprop{P_i} + 1} = 
       \frac{1 + 3 + 1}{1 + 1} = \frac{5}{3}$$ 
  
      %  Now, we need to find $Q_i'$ for which $\lenHOopt{Q'_i}$ is the least, 
      %  and prefix $\alpha$ such that $p$ and $\frac{p}{p^*}$ are the least. We 
      %  can see that $Q_i' = \inact$ we have $\lenHOopt{Q'_i} = 1$ 
      %  and for the output prefix we have $p = 3$ and $\frac{p}{p^*} = \frac{3}{1}$.  
      %  Now, by substituting those values we have: 
      % %  $$\frac{\frac{5}{3}\cdot 1 + 3 + 1}{1 + 1 + 1} =  \frac{5}{3}$$ 

      %  Now, by IH we know that when
      %  $Q_i' = \inact$ then $\frac{\lenHO{Q_i'} + 2 \cdot \lentr{Q_i}}{\lenHOopt{Q_i'}} = 1$, 
      %  (otherwise $\frac{\lenHO{Q_i} + 2 \cdot \lentr{Q_i}}{\lenHOopt{Q_i}} \geq k$). 
      %  Also, for 
      %  $\alpha$ we take output. 
      %  % and $Q_i' = \inact$ then $\frac{\lenHO{Q_i}}{\lenHOopt{Q_i}}$ is the least. 
      %  That is, we have $\lenHO{Q_i} + 2 \cdot \lentr{Q_i}= 4$ and $\lenHOopt{Q_i} = 2$. 
       So, we can conclude that 
      inequality \eqref{eq:measure-prop1} holds. 
       \end{itemize}
         \end{proof} 

\subsection{Typability of the Optimized Breakdown Function}

\begin{restatable}[Typability of Breakdown: $\Brec{k}{\tilde y}{\cdot}_g$]{lemm}{lemmbrec}
  \label{lem:brec}
    Let $P$ be an initialized process. 
    If $\Gamma \cdot X : \envR;\Delta \proves P \hastype \Proc$ 
    then: 
    \begin{align*}
      \Gt{\Gamma \setminus \wtd x};\Theta 
      \proves \Brec{k}{\tilde y}{P}_g \hastype \Proc \quad (k > 0)
    \end{align*}
    \noindent where 
    % $g = \{X \mapsto \wtd m\}$,
    $\wtd x \subseteq \fn{P}$
    such that 
    $\Delta \setminus \wtd x = \emptyset$ 
    , $\wtd y = \wtd v \cdot \wtd m$ where 
    $\wtd v$ is such that
    and $\indexed{\wtd v}{\wtd x}{\Gamma, \Delta}$
    and $\wtd m = \codom{g}$. Also,  
    $\Theta = \thetaR \cat \thetax(g)$ 
    where 
    % $\Theta = \thetaR \cat 
    % \dual{\prop^r_X}:\trec{t}{\btout{\wtd M}}\tvar{t}$ where 
    $\balan{\thetaR}$ with 
    $\dom{\thetaR} = \{\prop^r_k,\prop^r_{k+1},\ldots,\prop^r_{k+\lenHOopt{P}-1} \} \cup 
    \{\dual{\prop^r_{k+1}},\ldots,\dual{\prop^r_{k+\lenHOopt{P}-1}}\}$ and 
    $\thetaR (\prop^r_k)=\trec{t}\btinp{\wtd N}\tvar{t}$
    if $g \not= \es$, otherwise 
    $\thetaR (\prop^r_k)=\chtype{\wtd N}$ 
    where $\wtd N = (\Gt{\Gamma},\Gt{\envR \cdot \Delta})(\wtd y)$. 
    % and $\thetax = \dual{\prop^r_X}:\trec{t}{\btout{\wtd M}}\tvar{t}$ with 
    %  $\wtd M = (\Gt{\Gamma},\Gt{\envR})(\wtd m)$
    and 
    %  $\thetax(g) = \bigcup_{X \in \dom{g}}\dual{\prop^r_X}:\trec{t}{\btout{\wtd M_X}}\tvar{t}$
     $\thetax(g) = \bigcup_{X \in \dom{g}}\prop^r_X:\chtype{\wtd M_X}$
     where 
     $\wtd M_X = (\Gt{\Gamma},\Gt{\envR})(g(X))$. 
  \end{restatable}
  \begin{proof}
    The proof is by the induction of the structure of $P$. 
    We consider cases when $g \not= \es$, as cases 
    when $g = \es$ are similar. 
    % We have five cases, depending on shape of $P$: 
  %   We 
 	% consider following cases: 
 	\begin{enumerate}
    % \item Case $P = \inact$. Directly by taking $g = \es$
    % and as $\wtd x = \es$
    %  thus $\wtd y = \es$ and $\Theta = \prop^r_k : \btinp{}\tinact$. 
 	\item Case $P = X$. The only rule that can be applied here is 
 			\textsc{RVar}: 
 			\begin{align}
 			\AxiomC{} 
 			\LeftLabel{\scriptsize RVar}
 				\UnaryInfC{$\Gamma \cdot X:\Delta;\Delta \proves X \hastype \Proc$}
 				\DisplayProof
 			\end{align}
 	
  Let $\wtd x = \emptyset$ as $\fn{P}=\emptyset$. 
  So, $\wtd y = \wtd m$ where $\wtd m = g(X)$. 
  Since $\lenHOopt{X}=1$ we have
 	$\thetaR = \{\prop^r_k:\trec{t}\btinp{\wtd N}\tvar{t}\}$ where $\wtd N =
 	(\Gt{\Gamma},\Gt{\Delta})(\wtd y)$. 
   In this case $\envR = \Delta$, thus $\wtd N = \wtd M$. 
 			We shall then prove the following judgment: 
 			\begin{align}
 				\Gt{\Gamma \setminus x}; 
         \Theta
         \proves \Brec{k}{\tilde y}{X}_g	\hastype \Proc 
 			\end{align}
 			By \tabref{t:bdowncorec}, we have: 
 			$$\Brec{k}{\tilde y}{X}_g = 
       \recp{X}\proprinpk{r}{k}{\wtd y}\propoutrecsh{\rvar{X}}{\wtd y}\rvar{X}$$
       \begin{align}
        \AxiomC{}
        \LeftLabel{\scriptsize RVar}
        \UnaryInfC{$\Gt{\Gamma \setminus x}\cat X : \Theta; 
       \Theta \proves
      \rvar{X}$}
      \AxiomC{}
      \LeftLabel{\scriptsize PolySend}
        \UnaryInfC{$\Gt{\Gamma \setminus x}\cat X : \Theta; 
        \wtd y : \wtd M \proves
        \wtd y \hastype \wtd M$}
        \LeftLabel{\scriptsize Req}
        \BinaryInfC{$\Gt{\Gamma \setminus x}\cat X : \Theta; 
        {\prop^r_X}:\chtype{\wtd M} \cat \wtd y : \wtd M \proves
        \propoutrecsh{\rvar{X}}{\wtd y}\rvar{X}$}
         \DisplayProof
         \label{pt:recvar-send1}
       \end{align}

 			The following tree proves this case: 
 			\begin{align}
        \AxiomC{\eqref{pt:recvar-send1}} 
        \AxiomC{} 
        \LeftLabel{\scriptsize PolySend}
        \UnaryInfC{$\Gt{\Gamma \setminus x}\cat X : \Theta;\wtd y : \wtd M \proves \wtd y \hastype \wtd M$}
        \LeftLabel{\scriptsize Rcv}
 			\BinaryInfC{$\Gt{\Gamma \setminus x}\cat X: \Theta;\Theta
       \proves \proprinpk{r}{k}{\wtd y}
       \propoutrecsh{\rvar{X}}{\wtd y}\rvar{X}	\hastype \Proc$} 
 			\LeftLabel{\scriptsize Rec}
 				\UnaryInfC{$\Gt{\Gamma \setminus x};\Theta
         \proves \recp{X}\proprinpk{r}{k}{\wtd y}
         \propoutrecsh{\rvar{X}}{\wtd y}\rvar{X}	\hastype \Proc$}
 				\DisplayProof
 			\end{align}
       \noindent where $\Theta=\thetaR \cat \dual{\prop^r_X}:\trec{t}\btout{\wtd M}\tvar{t}$.

 		\item Case $P = \bout{u_i}{z_j}P'$. 
 		Let $u_i :C$. 
     We distinguish three sub-cases: \rom{1} 
     $C = S = \trec{t}\btout{C_z}S'$, 
     \rom{2} 
     $C = S = \btout{C_z}S'$, and 
     \rom{3} 
     $C = \chtype{C_z}$. 
     We consider first two sub-cases, as \rom{3} is shown similarly. 
     The only rule that can be applied here is 
 		\textsc{Send}: 
 		\begin{align}
 		\label{pt:brec-out-inv}
 			\AxiomC{$\Gamma \cdot X:\envR; \Delta \cdot u_i:{S'}
 			\proves P' \hastype \Proc 
 			$} 
 			\AxiomC{$\Gamma \cdot X:\envR; \Delta_z \proves z_j \hastype C$} 
 			\LeftLabel{\scriptsize Send}
 			\BinaryInfC{$\Gamma \cdot X:\envR;\Delta \cdot u_i:S
 			\cdot \Delta_z \proves \bout{u_i}{z_j}P' \hastype \Proc $} 
 			\DisplayProof	
 		\end{align}
   	Then, by IH on the right assumption of \eqref{pt:brec-out-inv} we have: 
 	\begin{align}
 		\label{pt:brec-out-ih}
 		\Gt{\Gamma \setminus \wtd x'}; \Theta' 
    %  \cdot \Gt{\Delta \cat r : S'}
 			\proves \Brec{k+1}{\tilde y'}{P'}_g \hastype \Proc 
 	\end{align}
 	\noindent where $\wtd x' \subseteq \fn{P}$ such that 
		$(\Delta \cat r:{S'}) \setminus \wtd x' = \emptyset$, 
    and $\wtd y' = \wtd v' \cup \wtd m$ where  
		 $\indexed{\wtd v'}{\wtd x'}{\Gamma,\Delta \cat r:{S'}}$. 
		Also, $\Theta' = \thetaR'  \cat \thetax$
    where $\thetaR'$ such that 
 	$\balan{\thetaR'}$ with 
 	$$\dom{\thetaR'} = \{\prop^r_{k+1},\prop^r_{k+2},\ldots,\prop^r_{k+\lenHOopt{P'}+1} \} \cup 
 	\{\dual{\prop^r_{k+2}},\ldots,\dual{\prop^r_{k+\lenHOopt{P'}-1}},\dual{\prop^r_{k+\lenHOopt{P'}+1}} \}$$ 
 	and 
 	$\thetaR' (\prop^r_{k+1})=\trec{t}\btinp{\wtd N'}\tvar{t}$
 	where 
    $\wtd N' = (\Gt{\Gamma},\Gt{\envR \cdot 
    \Delta \cdot u_i:S})(\wtd y')$.
		By applying \lemref{lem:varbreak} on the second assumption of \eqref{pt:brec-out-inv} we have: 
 		\begin{align}
 		\label{eq:rec-out-ih2}
 		\Gt{\Gamma \cdot X : \envR} ; \Gt{\Delta_z} \proves \wtd z \hastype \Gt{C_z}
 		\hastype \Proc 
 		\end{align}

 		Let $\sigma = \nextn{u_i}$ 
     and in sub-case \rom{1} $\sigma_1 = \subst{\tilde n}{\tilde u}$ 
     where $\wtd n = (u_{i+1}, \ldots, u_{i + {\Gt{S}}})$ 
     and $\wtd u = (u_{i}, \ldots, u_{i + {\Gt{S}}-1})$, 
     otherwise \rom{2} $\sigma_1 = \epsilon$. 
 		We define $\wtd x = \wtd x' \cat z$ and 
 		$\wtd y = \wtd y'\sigma_1 \cat \wtd z \cdot u_i$. 

    By construction $\wtd x \subseteq P$ and 
    $(\Delta \cdot u_i:S \cdot \Delta_z) \setminus \wtd x = \emptyset$. 
    Further, we may notice that $\wtd y = \wtd v \cdot \wtd m$ such that 
 		 		$\indexed{\wtd v}{\wtd x}{\Gamma, \Delta \cat u_i:{S} \cat \Delta_z}$ and 
 		$\wtd y' = \wtd m \cup \fnb{P'}{\wtd y}$. 
 		% Let $\thetaR = \thetaR' \cat \Theta'$ where: 
     Let $\Theta = \thetaR  \cat \thetax$ where 
 		$$\thetaR = \thetaR' \cat 
     \prop^r_{k}:\trec{t}\btinp{\wtd N}\tvar{t} 
     \cat \dual{\prop^r_{k+1}}:\trec{t}\btout{\wtd N'}\tvar{t}$$
 		
	\noindent where 
  $\wtd N = (\Gt{\Gamma},\Gt{\envR \cdot \Delta \cdot u_i:{S} \cdot \Delta_z})(\wtd y)$. 
  By construction and since $\lenHOopt{P}=\lenHOopt{P'}+1$ we have 
	$$\dom{\thetaR} = \{\prop^r_k,\prop^r_{k+1},\ldots,\prop^r_{k+\lenHOopt{P}-1} \} \cup 
 	\{\dual{\prop^r_{k+1}},\ldots,\dual{\prop^r_{k+\lenHOopt{P}-1}} \}$$
 	
 	and $\balan{\thetaR}$. 
	By \tabref{t:bdowncorec} we have: 
 		\begin{align}
 			\Brec{k}{\tilde y}{P}_g = \recp{X}\binp{\prop^r_k}{\wtd y}
      		\bout{u_l}{\wtd z} 
      		\bout{\prop^r_{k+1}}{\wtd y'\sigma_1}X
      	 \Par
        \Brec{k+1}{\tilde y'\sigma_1}{P'\sigma}_g
 		\end{align}
     \noindent where in sub-case \rom{1} $l = i$ and 
     in sub-case \rom{2} $l = f(S)$. 
	We shall prove the following judgment: 
	\begin{align}
		\Gt{\Gamma \setminus \wtd x}; \Theta \proves \Brec{k}{\tilde y}{P}_g \hastype \Proc 
	\end{align}
	
	Let $\Delta_1 = \Delta \cat u_i:{S} \cat \Delta_z$ 
  and $\wtd u_i = \bname{u_i : S}$. 
  % Let $\sigma = \nextn{u_i}$. 
  We use some auxiliary
 			sub-trees: 
	\begin{align}
	\label{pt:brec-out4}
		\AxiomC{} 
		\LeftLabel{\scriptsize RVar}
		\UnaryInfC{$\Gt{\Gamma \setminus \wtd x} \cdot X : \Theta;\Theta 	\proves  
      		X \hastype \Proc $}	
		\DisplayProof
	\end{align}

	\begin{align}
	\label{pt:brec-out2}
		\AxiomC{\eqref{pt:brec-out4}} 
		\AxiomC{} 
		\LeftLabel{\scriptsize PolyVar}
		\UnaryInfC{$\Gt{\Gamma \setminus \wtd x} \cdot X : \Theta;
		\Gt{\Delta \cat u_i\sigma:{S'}}  \proves 
		\wtd y'\sigma_1 \hastype \wtd N'$} 
		\LeftLabel{\scriptsize PolySend}
		\BinaryInfC{$\Gt{\Gamma \setminus \wtd x} \cdot X : \Theta;\Theta \cat 
	\Gt{\Delta \cat u_i\sigma:{S'}}
	\proves  
  \proproutk{r}{k+1}{\wtd y'\sigma_1}X \hastype \Proc $}	
		\DisplayProof
	\end{align}

    Here, in typing the right-hand assumption, we may notice that in 
    sub-case \rom{1} 
    $\Gt{u_i:S} = \wtd u_i : \btout{\Gt{C_z}}\tinact \cat \Gt{S'} $ and 
    $\Gt{u_{i}\sigma:S'} =\wtd u_{i+1}:\Gt{S'}$
    where $\wtd u_{i+1} = (u_{i+1}, \ldots, u_{i + \len{\Gt{S'}}})$. 
    So right-hand side follows by  \defref{def:indexed} and \lemref{lem:subst}.
    % and by definition $\wtd u_{i+1} \subseteq \wtd y'\sigma_1$
    Otherwise, in sub-case \rom{2} 
    by \defref{def:typesdecompenv} and \defref{f:tdec} we know 
    $\Gt{u_i:S} = \Gt{u_i\sigma:S'}$ and 
    by definition $\wtd u_i \subseteq \wtd m \subseteq \wtd y'\sigma_1$.

	\begin{align}
	\label{pt:brec-out1}
	\AxiomC{\eqref{pt:brec-out2}}
	\AxiomC{\eqref{eq:rec-out-ih2}} 
	\LeftLabel{\scriptsize PolySend} 
	\BinaryInfC{$\Gt{\Gamma \setminus \wtd x} \cdot X : 
  \Theta;\Theta \cat \Gt{\Delta_1}\proves  
      		\bout{u_l}{\wtd z} 
          \proproutk{r}{k+1}{\wtd y'\sigma_1}X \hastype \Proc $}
	\DisplayProof	
	\end{align}

	\begin{align}
	\label{pt:brec-out0}
	\AxiomC{\eqref{pt:brec-out1}} 
	\AxiomC{}
	\LeftLabel{\scriptsize PolyVar} 
	\UnaryInfC{$\Gt{\Gamma \setminus \wtd x} \cdot X : \Theta;\Gt{\Delta_1}
	\proves 
	\wtd y \hastype \wtd N$} 
	\LeftLabel{\scriptsize PolyRcv}
		\BinaryInfC{$\Gt{\Gamma \setminus \wtd x} \cdot X : \Theta; \Theta \proves 
      		\binp{\prop^r_k}{\wtd y}
      		\bout{u_l}{\wtd z} 
          \proproutk{r}{k+1}{\wtd y'\sigma_1}X \hastype \Proc $}
		\LeftLabel{\scriptsize Rec}
		\UnaryInfC{$\Gt{\Gamma \setminus \wtd x};\Theta \proves 
		\recp{X}\binp{\prop^r_k}{\wtd y}
      		\bout{u_l}{\wtd z} 
      	\proproutk{r}{k+1}{\wtd y'\sigma_1}X \hastype \Proc $}
		\DisplayProof
	\end{align}
We may notice that 
by \defref{def:typesdecompenv} and \defref{f:tdec} we have 
$\Gt{\Delta_1}=\Gt{\Delta} \cat \wtd u_i : \Gt{S} \cat \Gt{\Delta_z}$
% where $\wtd u_i = \bname{u_i : S}$. 
So, in sub-case \rom{1} as $u_i = u_l$ we have $\Gt{\Delta_1}(u_l) = \btout{\Gt{C_z}}\tinact$. 
 			% $\Gt{\Delta_1}=\Gt{\Delta} \cat \wtd r : \Rtsopt{}{}{S} \cat 
 			% \Gt{\Delta_z}$
       In sub-case \rom{2}, by \lemref{lem:indexcor}
       and as $u_l = u_{f(S)}$
 			we know $\Gt{\Delta_1}(u_l) = \trec{t}\btout{\Gt{C_z}}\vart{t}$. 
      %  Also, by \defref{def:typesdecompenv} and \defref{f:tdec} we know 
      %   $\Gt{u_i:S} = \Gt{u_i\sigma:S'}$ and 
      %   by definition. 
The following tree proves this case:

	\begin{align}
		\AxiomC{\eqref{pt:brec-out0}}
		\AxiomC{\eqref{pt:brec-out-ih}} 
		\LeftLabel{\scriptsize Par}
		\BinaryInfC{$\Gt{\Gamma \setminus \wtd x}; \Theta \proves 
		\recp{X}\binp{\prop^r_k}{\wtd y}
      		\bout{u_l}{\wtd z} 
      		\bout{\prop^r_{k+1}}{\wtd y'\sigma_1}X 
          \Par \Brec{k+1}{\tilde y'\sigma_1}{P'\sigma}_g \hastype \Proc $} 
		\DisplayProof	
    \label{pt:brec-out-ptree}
	\end{align}

  Note that we have used the following for the right assumption
  of \eqref{pt:brec-out-ptree}:  
  $$\Brec{k+1}{\tilde y'}{P'} \equiv_{\alpha} \Brec{k+1}{\tilde y'\sigma_1}{P'\sigma}$$

		\item Case $P = \binp{u_i}{z}P'$. 
    We distinguish three sub-cases: \rom{1} 
    $C = S = \trec{t}\btinp{C_z}S'$, 
    \rom{2} 
    $C = S = \btinp{C_z}S'$, and 
    \rom{3} 
    $C = \chtype{C_z}$. 
    The only rule that can be applied here is 
 		\textsc{Rcv}: 
 		\begin{align}
 		\label{pt:brec-inp-inv}
 			\AxiomC{$\Gamma \cdot X:\envR; \Delta \cat u_i:{S'}
 			\cat 
 			\Delta_z 
 			\proves P' \hastype \Proc 
 			$} 
 			\AxiomC{$\Gamma \cdot X:\envR; \Delta_z \proves z \hastype C$} 
 			\LeftLabel{\scriptsize Rcv}
 			\BinaryInfC{$(\Gamma \setminus z)\cdot X:\envR;\Delta \cat u_i:S
 		 \proves \binp{u_i}{z}P' \hastype \Proc $} 
 			\DisplayProof	
 		\end{align}
 		
		Let $\wtd x' \subseteq \fn{P'}$ such that 
		$(\Delta \cdot u_i:{S'} \cdot \Delta_z) \setminus \wtd x' = \emptyset$ 
		and $\wtd y' = \wtd v \cup \wtd m$ such that
     $\indexed{\wtd v'}{\wtd x'}{\Gamma,\Delta \cat u_i:{S'}}$. 
     Also, $\Theta' = \thetaR' \cat \thetax(g)$ where 
 	$\balan{\thetaR'}$ with 
 	$$\dom{\thetaR'} = \{\prop^r_{k+1},\prop^r_{k+2},\ldots,\prop^r_{k+\lenHOopt{P'}+1} \} \cup 
 	\{\dual{\prop^r_{k+2}},\ldots,\dual{\prop^r_{k+\lenHOopt{P'}+1}} \}$$ 
 	and 
 	$\thetaR' (\prop^r_{k+1})=\trec{t}\btinp{\wtd N'}\tvar{t}$, 
 	where  $\wtd N' = (\Gt{\Gamma} \cat \Gt{\envR \cdot \Delta \cdot u_i:{S} })(\wtd y')$.
 	Then, by IH on the right assumption of \eqref{pt:brec-out-inv} we have: 
 	\begin{align}
 		\label{pt:brec-inp-ih}
 		\Gt{\Gamma \setminus \wtd x'}; \thetaR' 
 			\proves \Brec{k+1}{\tilde y'}{P'}
 			\hastype \Proc 
 	\end{align}
		
 		 By applying \lemref{lem:varbreak}  to the second 
 		 assumption of \eqref{pt:brec-out-inv}, we have: 
 		 \begin{align}
 		 \label{pt:brecinp-ih2}
 		 	\Gt{\Gamma} \cdot X : \thetaR; \Gt{\Delta_z} \proves \wtd z \hastype \Gt{C}
 		 \end{align}

 		Let $\sigma = \nextn{u_i}$ 
     and in sub-case \rom{1} $\sigma_1 = \subst{\tilde n}{\tilde u}$ 
     where $\wtd n = (u_{i+1}, \ldots, u_{i + {\Gt{S}}})$ 
     and $\wtd u = (u_{i}, \ldots, u_{i + {\Gt{S}}-1})$, 
     otherwise in sub-case \rom{2} $\sigma_1 = \epsilon$. 
 		We define $\wtd x = \wtd x'\sigma \setminus z$ and 
 		$\wtd y = \wtd y'\sigma_1 \setminus \wtd z$ with 
 		$\len{\wtd z} = \len{\Gt{C}}$. By construction 
     $\wtd x \subseteq \fn{P}$ and $(\Delta \cat r:S) \setminus \wtd x = \es$. 
 		Further, we may notice that $\wtd y=\wtd v \cdot \wtd m$ where $\wtd v$ is 
     such that 
     $\indexed{\wtd v}{\wtd x}{\Gamma, \Delta \cat r:{S} \cat \Delta_z}$
 		and  
 		$\wtd y = \wtd m \cup \fnb{P'}{\wtd y \wtd z}$. 
     Let $\Theta = \thetaR  \cat \thetax$ where 
 		$$\thetaR = \thetaR' \cat \prop^r_{k}:\trec{t}\btinp{\wtd N}\tvar{t} \cat 
     \dual{\prop^r_{k+1}}:\trec{t}\btout{\wtd N'}\tvar{t}$$
 		
	\noindent where 
  $\wtd N = (\Gt{\Gamma},\Gt{\envR \cdot \Delta \cdot u_i:{S} \cat \Delta_z})(\wtd y)$. 
  By construction and since $\lenHOopt{P}=\lenHOopt{P'}+1$ we have 
	$$\dom{\thetaR} = \{\prop^r_k,\prop^r_{k+1},\ldots,\prop^r_{k+\lenHOopt{P}-1} \} \cup 
 	\{\dual{\prop^r_{k+1}},\ldots,\dual{\prop^r_{k+\lenHOopt{P}-1}} \}$$
 	
 	and $\balan{\thetaR}$. 
% 	Since $\wtd x = \wt$
% 	Since $\mathsf{tr}(S)$ we know
% 	$\fn{P} = \fn{P'} \cat z$ and by this 
% 	$(\Delta \cat r:S' \cat \Delta_z) \setminus \wtd x = \emptyset$.
	By \tabref{t:bdowncorec}, we have: 
 		\begin{align}
 		\Brec{k}{\tilde y}{P}_g = 
 			\recp{X}\binp{\prop^r_k}{\wtd y}
      		\binp{u_l}{\wtd z} 
      		\bout{\prop^r_{k+1}}{\wtd y'\sigma_1}X
      	 \Par
        \Brec{k+1}{\tilde y}{P'\sigma}_g
 		\end{align}
     \noindent where in sub-case \rom{1} $l = i$ and 
     in sub-case \rom{2} $l = f(S)$. 
Let $\Gamma_1 = \Gamma \setminus \wtd x$.
	We shall prove the following judgment: 
	\begin{align}
		\Gt{\Gamma_1 \setminus z}; \Theta \proves \Brec{k}{\tilde y}{P}_g \hastype \Proc 
	\end{align}
	
	%  Let $\Delta_1 = \Delta \cat u_i:{S} 
 	% 		\cat \Delta_z$. 
	We use some auxiliary sub-trees: 
	\begin{align}
	\label{pt:brec-inp4}
		\AxiomC{} 
		\LeftLabel{\scriptsize RVar}
		\UnaryInfC{$\Gt{\Gamma} \cdot X : \Theta;\Theta 	\proves  
      		X \hastype \Proc$}	
		\DisplayProof
	\end{align}

	\begin{align}
	\label{pt:brec-inp2}
		\AxiomC{\eqref{pt:brec-inp4}} 
		\AxiomC{} 
		\LeftLabel{\scriptsize PolyVar}
		\UnaryInfC{$\Gt{\Gamma} \cdot X : \Theta;
		\Gt{\Delta \cat u_l:{S'} 
    \cat \Delta_z} \proves 
		\wtd y'\sigma_1 \hastype \wtd N'$} 
		\LeftLabel{\scriptsize PolySend}
		\BinaryInfC{$\Gt{\Gamma} \cdot X : \Theta;\Theta 
		\cat 
	\Gt{\Delta_1}
	\proves  
      		\bout{\prop^r_{k+1}}{\wtd y'\sigma_1}X
      		\hastype \Proc$}	
		\DisplayProof
	\end{align}

  Here, in typing the right-hand assumption, we may notice that in 
  sub-case \rom{1} 
  $\Gt{u_i:S} = \wtd u_i : \btinp{\Gt{C_z}}\tinact \cat \Gt{S'} $ and 
  $\Gt{u_{i}\sigma:S'} =\wtd u_{i+1}:\Gt{S'}$
  where $\wtd u_{i+1} = (u_{i+1}, \ldots, u_{i + \len{\Gt{S'}}})$
  and by definition $\wtd u_{i+1} \subseteq \wtd y'\sigma_1$. 
  So right-hand side follows by  \defref{def:indexed} and \lemref{lem:subst}.
  Otherwise, in sub-case \rom{2} 
  by \defref{def:typesdecompenv} and \defref{f:tdec} we know 
  $\Gt{u_i:S} = \Gt{u_i\sigma:S'}$. 
  % So right-hand side follows by  \defref{def:indexed} and \lemref{lem:subst}.
  % by definition $\wtd u_i \subseteq \wtd m \subseteq \wtd y'\sigma_1$. 
  % Further, we may notice that 
  % $\Gt{\Delta_z}(\wtd z) = \Gt{C_z}$ and 
  % in \rom{1} and \rom{2} $\wtd z \subseteq \wtd y'\sigma_1$.

	\begin{align}
	\label{pt:brec-inp1}
	\AxiomC{\eqref{pt:brec-inp2}}
	\AxiomC{\eqref{pt:brecinp-ih2}} 
	\LeftLabel{\scriptsize PolyRcv} 
	\BinaryInfC{$\Gt{\Gamma \setminus z} \cdot X : \Theta;\Theta \cat 
	\Gt{\Delta \cat u_i : S}
	\proves  
      		\binp{u_l}{\wtd z} 
      		\bout{\prop^r_{k+1}}{\wtd y'\sigma_1}X
      		\hastype \Proc$}
	\DisplayProof	
	\end{align}

	\begin{align}
	\label{pt:brec-inp0}
	\AxiomC{\eqref{pt:brec-inp1}} 
	\AxiomC{}
	\LeftLabel{\scriptsize PolyVar} 
	\UnaryInfC{$\Gt{\Gamma \setminus z} \cdot X : \Theta;
	\Gt{\Delta \cat r : S}
	\proves 
	\wtd y \hastype \wtd N$} 
	\LeftLabel{\scriptsize PolyRcv}
		\BinaryInfC{$\Gt{\Gamma_1 \setminus z} \cdot X : \Theta;\Theta \proves 
      		\binp{\prop^r_k}{\wtd y}
      		\binp{u_l}{\wtd z} 
      		\bout{\prop^r_{k+1}}{\wtd y'\sigma_1}X \hastype \Proc $}
		\LeftLabel{\scriptsize Rec}
		\UnaryInfC{$\Gt{\Gamma_1 \setminus z};\Theta \proves 
		\recp{X}\binp{\prop^r_k}{\wtd y}
      		\binp{u_l}{\wtd z} 
      		\bout{\prop^r_{k+1}}{\wtd y'\sigma_1}X
      		\hastype \Proc $}
		\DisplayProof
	\end{align}
% We may notice that 
% by \defref{def:typesdecompenv} and \defref{f:tdec} we have 
%  			$\Gt{\Delta \cat r:S}=\Gt{\Delta} \cat \wtd r : \Rtsopt{}{}{S}$.
%  			 Further, by \lemref{lem:indexcor}
%  			we know $\Gt{\Delta \cat r:S}(r_{f(S)}) = \trec{t}\btinp{\Gt{C}}\vart{t}$.
We may notice that 
by \defref{def:typesdecompenv} and \defref{f:tdec} we have 
$\Gt{\Delta_1}=\Gt{\Delta} \cat \wtd u_i : \Gt{S} \cat \Gt{\Delta_z}$
% where $\wtd u_i = \bname{u_i : S}$. 
So, in sub-case \rom{1} as $u_i = u_l$ we have
 $\Gt{\Delta_1}(u_l) = \btinp{\Gt{C_z}}\tinact$. 
       In sub-case \rom{2}, by \lemref{lem:indexcor}
       and as $u_l = u_{f(S)}$
 			we know $\Gt{\Delta_1}(u_l) = \trec{t}\btinp{\Gt{C_z}}\vart{t}$. 
The following tree proves this case:

	\begin{align}
		\AxiomC{\eqref{pt:brec-inp0}}
		\AxiomC{\eqref{pt:brec-inp-ih}} 
		\LeftLabel{\scriptsize Par}
		\BinaryInfC{$\Gt{\Gamma_1 \setminus z};\Theta \proves 
		\recp{X}\binp{\prop^r_k}{\wtd y}
      		\binp{u_l}{\wtd z} 
      		\bout{\prop^r_{k+1}}{\wtd y'\sigma_1}X
      	 \Par
        \Brec{k+1}{\tilde y'\sigma_1}{P'\sigma}_g$} 
		\DisplayProof	
    \label{pt:brec-inp-ptree}
	\end{align}

  Note that we have used the following for the right assumption
  of \eqref{pt:brec-inp-ptree}:  
  $$\Brec{k+1}{\tilde y'}{P'} \equiv_{\alpha} \Brec{k+1}{\tilde y'\sigma_1}{P'\sigma}$$

\item Case $P = Q_1 \Par Q_2$. The only rule that can be applied here 
is \textsc{Par}: 

\begin{align}
	\label{pt:brec-par-inv}
	\AxiomC{$\Gamma \cdot X : \envR;\Delta_1 \proves Q_1 \hastype \Proc$}
	\AxiomC{$\Gamma \cdot X : \envR;\Delta_2 \proves Q_2 \hastype \Proc$}
	\LeftLabel{\scriptsize Par}
	\BinaryInfC{$\Gamma \cdot X : \envR;\Delta_1 \cat \Delta_2
					     \proves Q_1 \Par Q_2 \hastype \Proc$}
	\DisplayProof
\end{align}

Here we assume $\recpx{Q_1}$. 
So, by IH on the first and second assumption of \eqref{pt:brec-par-inv} we have: 
\begin{align}
  \label{pt:brec-par-ih1}
  \Gt{\Gamma \setminus x_1};\Theta_1 &\proves \Brec{k}{\tilde y_1}{Q_1}_{g} \hastype \Proc \\
  \label{pt:brec-par-ih2}  
  \Gt{\Gamma \setminus x_1};\Theta_2 &\proves \Brec{k+\degree +1}{\tilde y_2}{Q_2}_{\es} \hastype \Proc
\end{align}
\noindent where for $i \in \{1,2\}$ we have $\wtd x_i \subseteq \fn{Q_i}$ such that 
$\Delta_i \setminus \wtd x = \es$,  
and $\wtd y_i = \wtd v_i \cdot \wtd m_i$ where $\wtd v_i$ is such that 
$\indexed{\wtd v_1}{\wtd x_i}{\Gamma, \Delta_i}$ and 
$\wtd m_i = \codom{g_i}$.
Further, $\Theta_i = \thetaR^i \cdot \thetax(g_i)$ where 
\begin{align*}
  \dom{\thetaR^1} &= \{\prop^r_{k+1},\prop^r_{k+2},\ldots,\prop^r_{k+\lenHOopt{Q_1}} \} \cup 
 	\{\dual{\prop^r_{k+2}},\ldots,\dual{\prop^r_{k+\lenHOopt{Q_1}}} \} \\
   \dom{\thetaR^2} &= \{\prop^r_{k+\degree+1},\prop^r_{k+\degree+2},\ldots,
   \prop^r_{k+\degree+\lenHOopt{Q_2}} \} 
  %  \cup 
 	% \{\dual{\prop^r_{k+2}},\ldots,\dual{\prop^r_{k+\degree+\len{Q_2}}} \}
\end{align*}

 	and 
 	$\thetaR^1 (\prop^r_{k+1})=\trec{t}\btinp{\wtd N^1}\tvar{t}$
   and 
   $\thetaR^2 (\prop^r_{k+\degree+1})=\chtype{\wtd N^2}$
   with $\wtd N^i = (\Gt{\Gamma},\Gt{\envR \cdot \Delta_i})(\wtd y_i)$. 
  Let $\Delta = \Delta_1 \cdot \Delta_2$. 
   We define $\wtd x = \wtd x_1 \cdot \wtd x_2$ 
   and $\wtd y = \wtd y_1 \cdot \wtd y_2$. 
  %  Let $g = g_1 \cdot g_2$.
   By construction $\wtd x \subseteq \fn{P}$ and $(\Delta_1\cdot \Delta_2) \setminus \wtd x = \es$. 
  Further, we may notice that $\wtd y = \wtd v \cdot \wtd m$ where 
  $\wtd m = \codom{g}$ and 
  $\indexed{\wtd v}{\wtd x}{\Gamma, \Delta}$.
   We shall prove the following judgment: 
   \begin{align}
     \Gt{\Gamma \setminus \wtd x}; \Theta \proves \Brec{k}{\tilde y}{P}_g \hastype \Proc 
   \end{align}
   \noindent where 
   $\Theta = \Theta_1 \cdot \Theta_2 \cdot \Theta'$ 
    with 
    $$\Theta'=\prop^r_k:  \trec{t}\btinp{\wtd N}\tvar{t}
    \cdot \dual{\prop^r_{k+1}}: \trec{t}\btout{\wtd N_1}\tvar{t}$$
    %  \cdot \dual{\prop^r_{k+\degree+1}}: \trec{t}\btout{\wtd N_2}\tvar{t}$$
   By \tabref{t:bdowncorec} we have: 
   \begin{align*}
    \Brec{k}{\tilde y}{P}_g = 
      \recp{X}\proprinpk{r}{k}{\wtd y} 
      (\proproutk{r}{k+1}{\wtd y_1}X \Par 
      \apropoutrecsh{k+\degree+1}{\wtd y_2})
      \Par
      \Brec{k+1}{\tilde y_1}{Q_1}_{g}\Par 
      \Brec{k+\degree+1}{\tilde y_2}{Q_2}_{\es}
   \end{align*}

   We use some auxiliary sub-trees: 
   \begin{align}
    \AxiomC{} 
    \LeftLabel{\scriptsize Nil}
    \UnaryInfC{$\Gt{\Gamma \setminus \wtd x} 
    \cdot X : \Theta' \proves \inact \hastype \Proc$} 
    \AxiomC{}
      \LeftLabel{\scriptsize PolyVar}
      \UnaryInfC{$\Gt{\Gamma \setminus \wtd x} 
               \cdot X : \Theta'
                ; \wtd y_2 : \wtd N_2 
                \proves \wtd y_2 \hastype \wtd N_2$} 
    \LeftLabel{\scriptsize Snd}
    \BinaryInfC{$\Gt{\Gamma \setminus \wtd x} 
    \cdot X : \Theta'
    ;  \cdot  \wtd y_2 : \wtd N_2
    \proves
          % \aproproutk{k+\degree+1}{\wtd y_2}\rvar{X}
          \apropoutrecsh{k+\degree+1}{\wtd y_2}
    $} 
     \DisplayProof
     \label{pt:brec-par-2}
   \end{align}

   \begin{align}
    \AxiomC{} 
    \LeftLabel{\scriptsize Rvar}
    \UnaryInfC{$\Gt{\Gamma \setminus \wtd x} 
    \cdot X : \Theta'; \Theta' \proves X \hastype \Proc$} 
    \AxiomC{}
      \LeftLabel{\scriptsize PolyVar}
      \UnaryInfC{$\Gt{\Gamma \setminus \wtd x} 
               \cdot X : \Theta'
                ; \wtd y_1 : \wtd N_1
                \proves \wtd y_1 \hastype \wtd N$} 
    \LeftLabel{\scriptsize Snd}
    \BinaryInfC{$\Gt{\Gamma \setminus \wtd x} 
    \cdot X : \Theta'
    ; \Theta' \cdot  \wtd y_1 : \wtd N_1
    \proves
        \proproutk{r}{k+1}{\wtd y_1}X 
    \hastype \Proc$} 
    \AxiomC{\eqref{pt:brec-par-2}}
    \LeftLabel{\scriptsize Par}
    \BinaryInfC{
      $\Gt{\Gamma \setminus \wtd x} 
      \cdot X : \Theta'
      ; \Theta' \cdot  \wtd y: \wtd N 
      \proves
          \proproutk{r}{k+1}{\wtd y_1}X \Par 
            \proproutk{r}{k+\degree+1}{\wtd y_2}
      \hastype \Proc$
    }
     \DisplayProof
     \label{pt:brec-par-1}
   \end{align}

    \begin{align}
      \AxiomC{\eqref{pt:brec-par-1}} 
      \AxiomC{}
      \LeftLabel{\scriptsize PolyVar}
      \UnaryInfC{$\Gt{\Gamma \setminus \wtd x} 
               \cdot X : \Theta'
                ; \wtd y : \wtd N 
                \proves \wtd y \hastype \wtd N$} 
      \LeftLabel{\scriptsize Rv}
      \BinaryInfC{$\Gt{\Gamma \setminus \wtd x} 
                   \cdot X : \Theta'
                      ; \Theta' \proves 
                  \proprinpk{r}{k}{\wtd y} 
                  (\proproutk{r}{k+1}{\wtd y_1}X \Par 
                    \apropoutrecsh{k+\degree+1}{\wtd y_2})
                    \hastype \Proc$} 
      \LeftLabel{\scriptsize Rec}
      \UnaryInfC{$
          \Gt{\Gamma \setminus \wtd x}; \Theta' \proves 
          \recp{X}\proprinpk{r}{k}{\wtd y} 
          (\proproutk{r}{k+1}{\wtd y_1}X \Par 
          \apropoutrecsh{k+\degree+1}{\wtd y_2})
        \hastype \Proc
      $}
      \DisplayProof
      \label{pt:brec-par-0}
    \end{align}

   The following tree proves this case: 
   \begin{align*}
    \AxiomC{\eqref{pt:brec-par-0}} 
    \AxiomC{\eqref{pt:brec-par-ih1}} 
    \AxiomC{\eqref{pt:brec-par-ih2}}
    \LeftLabel{\scriptsize Par}
    \BinaryInfC{$\Gt{\Gamma \setminus \wtd x}; \Theta \proves
    \Brec{k+1}{\tilde y_1}{Q_1}_{g_1} \Par 
    \Brec{k+\degree+1}{\tilde y_2}{Q_2}_{g_2} \hastype \Proc$}
    \LeftLabel{\scriptsize Par}
    \BinaryInfC{$
        \Gt{\Gamma \setminus \wtd x}; \Theta_1 \cdot \Theta_2 \proves 
        \recp{X}\proprinpk{r}{k}{\wtd y} 
        (\proproutk{r}{k+1}{\wtd y_1}X \Par 
        \apropoutrecsh{k+\degree+1}{\wtd y_2})
        \Par
        \Brec{k+1}{\tilde y_1}{Q_1}_{g}
        \Par 
        \Brec{k+\degree+1}{\tilde y_2}{Q_2}_{\es} \hastype \Proc
    $}
     \DisplayProof
   \end{align*}

   \item Case $P = \news{s:C}P'$. 
   We distinguish two sub-cases: \rom{1} $C = S$ and \rom{2}
   $C = \chtype{C'}$. 
   We only consider sub-case \rom{1} as the other  is similar. 
   First, we $\alpha$-convert $P$ as follows: 
   \begin{align*}
    P \equiv_{\alpha} \news{s_1:C}P'\subst{s_1 \dual{s_1}}{s \dual{s}}
  \end{align*}
  The only can that can be applied is \textsc{ResS}: 
  \begin{align}
    \label{pt:brec-news-inv}
    \AxiomC{$\Gamma; \envR \cdot \Delta \cdot s_1:S \cdot \dual {s_1}:\dual S
          \proves P'\subst{s_1 \dual{s_1}}{s \dual{s}} \hastype \Proc$}
    \LeftLabel{\scriptsize ResS}
    \UnaryInfC{$\Gamma; \envR \cdot \Delta \proves
                \news{s_1:S}P'\subst{s_1 \dual{s_1}}{s \dual{s}} \hastype \Proc$}
    \DisplayProof
  \end{align}

  By IH on the assumption of \eqref{pt:brec-news-inv} we have:
  \begin{align}
    \label{eq:brec-news-ih}
    \Gt{\Gamma \setminus \wtd x};
    % \Gt{s_1:S \cat \dual {s_1}:\dual S}
          \Theta' \proves
          \Brec{k}{\tilde y'}{P'\subst{s_1 \dual{s_1}}{s \dual{s}}}_g \hastype \Proc
  \end{align}

  \noindent where $\wtd x' \subseteq \fn{P}$ such that 
		$(\Delta \cdot s_1:S \cdot \dual{s_1}:\dual S) \setminus \wtd x' = \emptyset$, 
    and $\wtd y' = \wtd v' \cup \wtd m$ where  
		 $\indexed{\wtd v'}{\wtd x'}{\Gamma,\Delta  \cdot s_1:S \cdot \dual{s_1}:\dual S}$. 
		Also, $\Theta' = \thetaR'  \cat \thetax$
    where $\thetaR'$ such that 
 	$\balan{\thetaR'}$ with 
 	$$\dom{\thetaR'} = \{\prop^r_{k+1},\prop^r_{k+2},\ldots,\prop^r_{k+\lenHOopt{P'}+1} \} \cup 
 	\{\dual{\prop^r_{k+2}},\ldots,\dual{\prop^r_{k+\lenHOopt{P'}+1}} \}$$ 
 	and 
 	$\thetaR' (\prop^r_{k+1})=\trec{t}\btinp{\wtd N'}\tvar{t}$
 	where 
    $\wtd N' = (\Gt{\Gamma},\Gt{\envR \cdot 
    \Delta  \cdot s_1:S \cdot \dual{s_1}:\dual S})(\wtd y')$.

    We define $\wtd x = \wtd x' \setminus (s_1, \dual{s_1})$ 
    and $\wtd y = \wtd y' \setminus (\wtd s \cdot \wtd{\dual{s}})$ 
    where $\wtd s = \bname{s_1:S}$ and $\wtd{\dual{s}} = \bname{\dual{s_1}:\dual S}$. 
    By construction $\wtd x \subseteq \fn{P}$ and $\Delta \setminus \wtd x =\es$. 
    Further, $\wtd y = \wtd v \cdot \wtd m$ where
    $\indexed{\wtd v}{\wtd x}{\Gamma,\Delta}$.  
    
    Let $\Theta = \Theta' \cat \thetaR''$ where 
    % $$\thetaR = \thetaR' \cat 
    % \prop^r_{k}:\trec{t}\btinp{\wtd N}\tvar{t} 
    % \cat \dual{\prop^r_{k+1}}:\trec{t}\btout{\wtd N'}\tvar{t}$$
    $$\thetaR'' = 
    \prop^r_{k}:\trec{t}\btinp{\wtd N}\tvar{t} 
    \cat \dual{\prop^r_{k+1}}:\trec{t}\btout{\wtd N'}\tvar{t}$$

	\noindent where 
  $\wtd N = (\Gt{\Gamma},\Gt{\envR \cdot \Delta \cdot u_i:{S}})(\wtd y)$. 
  By construction and since $\lenHOopt{P}=\lenHOopt{P'}+1$ we have 
	$$\dom{\thetaR} = \{\prop^r_k,\prop^r_{k+1},\ldots,\prop^r_{k+\lenHOopt{P}-1} \} \cup 
 	\{\dual{\prop^r_{k+1}},\ldots,\dual{\prop^r_{k+\lenHOopt{P}-1}} \}$$

   By \tabref{t:bdowncorec} we have:
  \begin{align*}
    \Brec{k}{\tilde y}{P}_g = 
      \recp{X}\news{\widetilde{s}:\Gt{C}}\propinp{k}{\wtd y}\propout{k+1}{\wtd y'}X
      \Par
      \Brec{k}{\tilde y'}{P'\subst{s_1 \dual{s_1}}{s \dual{s}}}_g
  \end{align*}

   We shall prove the following judgment: 
   \begin{align}
     \Gt{\Gamma \setminus \wtd x}; \Theta \proves \Brec{k}{\tilde y}{P}_g \hastype \Proc 
   \end{align}

   We use some auxiliary sub-tree:

\begin{align}
  \label{pt:brec-news-pt1}
  \AxiomC{} 
  \LeftLabel{\scriptsize Rvar}
  \UnaryInfC{$\Gt{\Gamma} \cdot X: \thetaR; \thetaR'' 
   \proves X 
  \hastype \Proc$} 
  \AxiomC{} 
  \LeftLabel{\scriptsize PolyVar}
  \UnaryInfC{$\Gt{\Gamma} \cdot X: \thetaR''; \Gt{\Delta}
  \cat 
  \wtd s : \Gt{S} \cat \wtd {\dual s}: \Gt{\dual S} \proves 
  \wtd y' \hastype \wtd N'$} 
  \LeftLabel{\scriptsize PolySend}
  \BinaryInfC{$\Gt{\Gamma}\cdot X:\thetaR;\thetaR \cdot \Gt{\Delta}
\cat 
\wtd s : \Gt{S} \cat \wtd {\dual s}: \Gt{\dual S}
\proves \propout{k+1}{\wtd y'}X
\hastype \Proc$}
  \DisplayProof
\end{align}

   The following tree proves this case: 

   \begin{align*}
    \AxiomC{\eqref{pt:brec-news-pt1}} 
    \AxiomC{} 
   \LeftLabel{\scriptsize PolyVar}
   \UnaryInfC{$\Gt{\Gamma};\Gt{\Delta} \proves \wtd y \hastype \wtd N$} 
    \LeftLabel{\scriptsize PolyRcv}
    \BinaryInfC{$\Gt{\Gamma \setminus \wtd x} \cdot X : \thetaR''; \thetaR'' 
    \cdot \wtd s : \Gt{S} \cat \wtd {\dual s}: \Gt{\dual S}
    \proves 
    \propinp{k}{\wtd y}\propout{k+1}{\wtd y'}X
        \hastype \Proc$}
    \LeftLabel{\scriptsize PolyResS}
    \UnaryInfC{$
    \Gt{\Gamma \setminus \wtd x} \cdot X : \thetaR''; \thetaR'' \proves 
    \news{\wtd{s}:\Gt{S}}
    \propinp{k}{\wtd y}\propout{k+1}{\wtd y'}X
        \hastype \Proc$} 
    \LeftLabel{\scriptsize Rec}
    \UnaryInfC{$	\Gt{\Gamma \setminus \wtd x}; \thetaR'' \proves 
    \recp{X}
    \news{\wtd s:\Gt{S}}
    \propinp{k}{\wtd y}\propout{k+1}{\wtd y'}X
        \hastype \Proc$} 
    \AxiomC{\eqref{eq:brec-news-ih}}
    \LeftLabel{\scriptsize Par}
    \BinaryInfC{$	\Gt{\Gamma \setminus \wtd x}; \Theta \proves 
          \recp{X}
          \news{\wtd s:\Gt{S}}
          \propinp{k}{\wtd y}\propout{k+1}{\wtd y'}X
          \Par
          \Brec{k}{\tilde y'}{P'\subst{s_1 \dual{s_1}}{s \dual{s}}}_g
     \hastype \Proc$}
     \DisplayProof
   \end{align*}

   This concludes the proof.

 	\end{enumerate}
% \qed
  \end{proof}

  \thmtyperecur*
  \label{app:proofbrec}
\begin{proof} 
  % \label{app:proofbrec}
  By induction on the structure of $P$. By assumption $\Gamma;\Delta \proves P
\hastype \Proc$	.
In total we consider nine cases. We separately treat 
 \texttt{Input} and \texttt{Output}  cases 
 depending on whether a subject name of the prefix is recursive. 
%  First, we consider six cases not involving recursive names 
%  in a prefix: 
%  Similarly, \texttt{Restriction} case depending if 
%  restricted name is recursive. 
% We consider six cases, depending on the shape of $P$, when
% subject names are not recursive (where applicable). Then, we separately treat
% \texttt{Input} and \texttt{Output} cases when subject name is recursive, and
% \texttt{Restriction} when restricted name is recursive.  
\begin{enumerate}
	\item Case $P = \inact$. The only rule that can be applied here is \textsc{Nil}.
	 By inversion of this rule, we have:
    $\Gamma;\es \proves \inact$.
    We shall then prove the following judgment:
    \begin{align}
    	\Gt{\Gamma};\Theta \proves \B{k}{\tilde y}{\inact} \hastype \Proc
    \end{align}

    \noindent where $\widetilde x \subseteq \fn{\inact}=\epsilon$ and $\Theta =
    \{c_k:\btinp{\chtype{\tinact}}\tinact\}$.  Since by \remref{r:prefix} we know that
    $\propinp{k}{} \inact$ stands for $\propinp{k}{y} \inact$ with
    $\prop_k : \btinp{\chtype{\tinact}}\tinact$.
    % \ref{t:}
    By \tabref{t:bdowncorec}: 
    $\B{k}{\epsilon}{\inact} =
    \propinp{k}{} \inact$. 

    The following tree proves this case:
    
    \begin{prooftree}
    \AxiomC{}
    \LeftLabel{\scriptsize Nil}
      \UnaryInfC{$\Gamma';\es;\es \proves \inact \hastype \Proc$}
      \AxiomC{$\prop_k \notin \dom{\Gamma}$}
      \LeftLabel{\scriptsize End}
      \BinaryInfC{$\Gamma';\es;\prop_k : \tinact \proves \inact \hastype \Proc$}
      \AxiomC{}
      \LeftLabel{\scriptsize Sh}
      \UnaryInfC{$\Gamma';\es \proves y \hastype \chtype{\tinact}$}
      \LeftLabel{\scriptsize Rcv}
      \BinaryInfC{$\Gt{\Gamma}\cat y : \chtype{\tinact};\Theta \proves \propinp{k}{} \inact \hastype \Proc$}
%      \LeftLabel{\scriptsize \lemref{lem:strength}
%      with $y$}
%      \UnaryInfC{$\Gt{\Gamma};\Theta \proves \propinp{k}{} \inact \hastype \Proc$}
    \end{prooftree}

    \noindent where $\Gamma' = \Gt{\Gamma} \cat y : \chtype{\tinact}$. 
	We know $\prop_k \notin \dom{\Gamma}$ since we use reserved names for 	propagators channels. %In the continuation of the proof 
	%we omit typing terminated processes. 
	
	\item Case $P = \binp{u_i}{z}P'$. We distinguish two sub-cases, depending on whether $u_i$ is linear or not: \rom{1}
  $u_i \in \dom{\Delta}$ and \rom{2} $u_i \in \dom{\Gamma}$.
  We consider
  sub-case \rom{1} first. For this case Rule \textsc{Rcv} can be applied:
    \begin{align}
      \label{pt:inputInv}
      \AxiomC{$\Gamma; \Delta \cat u_i : S  \cat \Delta_z \proves P' \hastype \Proc$}
      \AxiomC{$\Gamma; \Delta_z \proves z \hastype C$}
      \LeftLabel{\scriptsize Rcv}
      \BinaryInfC{$\Gamma \setminus z;
      				\Delta \cat u_i:
                    \btinp{C}S \proves \binp{u_i}{z}P' \hastype \Proc$}
      \DisplayProof
    \end{align}

  By IH on the first assumption of \eqref{pt:inputInv} we know:
  \begin{align}
    \label{eq:input-ih}
    \Gt{\Gamma'_1};\Gt{\Delta'_1} \cat \Theta_1 \proves
    \B{k+1}{\tilde y'}{P'} \hastype \Proc
  \end{align}
  \noindent where  $\li x' \subseteq \fn{P'}$ 
and $\li y'$ such that $\indexed{\wtd y'}{\wtd x'}{\Gamma,\Delta}$. 
Also, 
   $\Gamma_1'=\Gamma \setminus \widetilde x'$, 
   $\Delta_1' = \Delta \setminus \widetilde x'$, and $\balan{\Theta_1}$ 
   with 
   $$
   \dom{\Theta_1}=\{\prop_{k+1},\ldots,\prop_{k+\lenHOopt{P'}}\}
   \cup \{\dual{\prop_{k+2}},\ldots,\dual{\prop_{k+\lenHOopt{P'}}}\}
   $$
   and ${\Theta_1(\prop_{k+1})}=\btinp{\widetilde M'}\tinact$
   where $\widetilde M' = (\Gt{\Gamma},\Gt{\Delta,u_i:S,\Delta_z})(\widetilde y')$.

 By applying \lemref{lem:varbreak} to the second
 assumption of \eqref{pt:inputInv} we have:
  \begin{align}
  	\label{eq:input-ih2}
  	\Gt{\Gamma};\Gt{\Delta_z} \proves \wtd z \hastype \Gt{C}
  \end{align}

Let $\wtd x = \wtd x',u \setminus z$ 
  and $\wtd y = \wtd y' \sigma ,u_i \setminus \wtd z$ such that 
  $\len{\wtd z}=\Gt{C}$ where $\sigma = \subst{\wtd n}{\wtd u}$ with $\widetilde n =
  	(u_{i+1},\ldots,u_{i+\len{\Gt{S}}})$ and $\widetilde u =
  	(u_i,\ldots,u_{i+\len{\Gt{S}}-1})$. We may notice that 
  by \defref{def:indexed} 
   $\indexed{\wtd y}{\wtd x}{\Gamma,\Delta}$ holds. 
  We define $\Theta = \Theta_1 \cat \Theta'$, where
  \begin{align*}
  \Theta' = \prop_k:\btinp{\widetilde M} \tinact \cat \dual {\prop_{k+1}}:\btout{\widetilde M'} \tinact
  \end{align*}
  with $\widetilde M = (\Gt{\Gamma},\Gt{\Delta \cat \cat u_i:
                    \btinp{C}S})(\widetilde y)$.
  By \defref{def:sizeproc},
  $\lenHOopt{P} = \lenHOopt{P'} + 1$ so
  $$\dom{\Theta} = \{\prop_k,\ldots,\prop_{k+\lenHOopt{P}-1}\}
  	\cup \{\dual{\prop_{k+1}},\ldots,\dual{\prop_{k+\lenHOopt{P}-1}}\}$$
  	and $\Theta$ is balanced since $\Theta(\prop_{k+1}) \dualof \Theta(\dual{\prop_{k+1}})$ and
  	 $\Theta_1$ is balanced.
  By \tabref{t:bdowncorec}:
  \begin{align*}
   \B{k}{\tilde y}{\binp{u_i}{z}P'} = \propinp{k}{\widetilde y}
   \binp{u_i}{\widetilde z}
   \propout{k+1}
   {\widetilde y'\sigma} \inact \Par \B{k+1}{\tilde y'\sigma}{P'\incrname{u}{i}}
 \end{align*}

%   Let $\wtd x = \wtd x',u \setminus z$ 
%   and $\wtd y = \wtd y',u_i \setminus \wtd z$ such that 
%   $\len{\wtd z}=\Gt{C}$. We may notice that 
%   by \defref{def:indexed} 
%   $\indexed{\wtd y}{\wtd x}{\Gamma,\Delta}$ holds. 
  Also, let $\Gamma_1 = \Gamma \setminus \widetilde x$ and 
  $\Delta_1 = \Delta \setminus \widetilde x$. We may notice that 
  $\Delta_1 = \Delta'_1$.
  We shall prove the following judgment:
  \begin{align*}
  \Gt{\Gamma_1 \setminus z};\Gt{\Delta_1}
    \cat \Theta
    \proves
    	\B{k}{\tilde y}{\binp{u_i}{z}P'}
  \end{align*}

  %\noindent where $\Gamma_1 = \Gamma \setminus \widetilde x$.
  We type sub-process $ \propinp{k}{\widetilde y}
   \binp{u_i}{\widetilde z}
   \propout{k+1}
   {\widetilde y'} \inact$ 
  with some auxiliary derivations:
   
 \begin{align}
 	\label{pt:input2}
    \AxiomC{}
    \LeftLabel{\scriptsize Nil}
    \UnaryInfC{$\Gt{\Gamma};\es \proves \inact \hastype \Proc$}
    \LeftLabel{\scriptsize End}
    \UnaryInfC{$\Gt{\Gamma};\dual{\prop_{k+1}}:\tinact \proves \inact \hastype \Proc$}
    \DisplayProof
 \end{align}

  \begin{align}
    %\gamma
    \label{st:input1}
%    \AxiomC{}
%    \LeftLabel{\scriptsize Nil}
%    \UnaryInfC{$\Gt{\Gamma};\es \proves \inact \hastype \Proc$}
%    \LeftLabel{\scriptsize End}
%    \UnaryInfC{$\Gt{\Gamma};\dual{\prop_{k+1}}:\tinact \proves \inact \hastype \Proc$}
\AxiomC{\eqref{pt:input2}} 
    \AxiomC{}
    \LeftLabel{\scriptsize PolyVar}
    \UnaryInfC{$\Gt{\Gamma};\Gt{\Delta\setminus\Delta_1\cat u_{i+1}:S} \cat \Gt{\Delta_z}
                \proves \widetilde y'\sigma \hastype \widetilde M'$}
    \LeftLabel{\scriptsize PolySend}
    \BinaryInfC{\begin{tabular}{c}
    $\Gt{\Gamma};
                  \dual {\prop_{k+1}}:\btout{\widetilde M'} \tinact
                  \cat \Gt{\Delta\setminus\Delta_1\cat u_{i+1}:S} \cat \Gt{\Delta_z}
                  \proves$ \\ $
                  \propout{k+1}{\widetilde y'\sigma} \inact \hastype \Proc$
                  \end{tabular}}
    \LeftLabel{\scriptsize End}
    \UnaryInfC{\begin{tabular}{c}$
    \Gt{\Gamma};
                  \dual {\prop_{k+1}}:\btout{\widetilde M'} \tinact
                  \cat u_i:\tinact \cat 
					\Gt{\Delta \setminus \Delta_1 \cat u_{i+1}:S}\cat \Gt{\Delta_z}
                  \proves $ \\ $
                  \propout{k+1}{\widetilde y'\sigma} \inact \hastype \Proc$
                  \end{tabular}}
    \DisplayProof
  \end{align}
  
  \begin{align}
    %beta
    \label{st:input-rcv}
    \AxiomC{\eqref{st:input1}}
	  \AxiomC{\eqref{eq:input-ih2}}
    \LeftLabel{\scriptsize PolyRcv}
    \BinaryInfC{
    \begin{tabular}{c}
        $\Gt{\Gamma \setminus z}; u_i:\btinp{\Gt{U}} \tinact \cat
                \dual {\prop_{k+1}}:\btout{\widetilde M'} \tinact \cat 
%                \widetilde y : \widetilde M
				\Gt{\Delta_2}
                \proves$ \\
                $\binp{u_i}{\widetilde z}\propout{k+1}{\widetilde y'\sigma} \inact \hastype \Proc$
    \end{tabular}
}
     \LeftLabel{\scriptsize End}
    \UnaryInfC{ 
    \begin{tabular}{c}
    $\Gt{\Gamma \setminus z}; 
                \dual {\prop_{k+1}}:\btout{\widetilde M'} \tinact
                \cat \prop_k: \tinact \cat
                \Gt{\Delta_2}
                \proves$ \\ 
                $\binp{u_i}{\widetilde z}\propout{k+1}{\widetilde y'\sigma} \inact \hastype \Proc$
     \end{tabular}}
    \DisplayProof
  \end{align}

  \begin{align}
    \label{st:input3}
    \AxiomC{\eqref{st:input-rcv}}
    \AxiomC{}
    \LeftLabel{\scriptsize PolyVar}
    \UnaryInfC{$\Gt{\Gamma \setminus z};
    \Gt{\Delta_2}
    \proves \widetilde y \hastype \widetilde M$}
    \LeftLabel{\scriptsize PolyRcv}
    \BinaryInfC{$\Gt{\Gamma_1 \setminus z};
     \Theta' \proves \propinp{k}{\widetilde
    y}\binp{u_i}{z}\propout{k+1}{\widetilde y'\sigma} \inact \hastype \Proc$}
  \DisplayProof
  \end{align}
	\noindent 
	where $\Delta_2 = \Delta \cat u_i:\btinp{C}S \setminus \Delta_1$. 
  Using \eqref{st:input3}, 
  the following tree
  proves this case:
  \begin{align}
  	\label{pt:input}
    \AxiomC{\eqref{st:input3}}
    \AxiomC{\eqref{eq:input-ih}}
     \LeftLabel{\scriptsize}
    \UnaryInfC{
    \begin{tabular}{c}
    $\Gt{\Gamma'_1 \setminus z}; \Gt{\Delta_1} \cat \Theta_1 \proves$ \\
    $\B{k+1}{\tilde y'\sigma}{P'\incrname{u}{i}} \hastype \Proc$
    \end{tabular}}
    \LeftLabel{\scriptsize Par}
    \BinaryInfC{\begin{tabular}{c}
    			$\Gt{\Gamma_1 \backslash z};\Gt{\Delta_1}
                  \cat \Theta \proves$ \\
                  $\propinp{k}{\widetilde y}
                  \binp{u_i}{\widetilde z}\propout{k+1}{\widetilde y'\sigma} \inact \Par \B{k+1}
                  {\tilde y'\sigma}{P'\incrname{u}{i}} \hastype \Proc$
                  \end{tabular}}
    \DisplayProof
  \end{align}
  	\noindent

  	Note that we have used the following for the right assumption of \eqref{pt:input}:
  	\begin{align*}
  		% \Gt{\Delta'_1 \cat u_i:S}\subst{\tilde n}{\tilde u} &=
  		% \Gt{\Delta'_1 \cat u_{i+1}:S} \\
  		\B{k+1}{\tilde y'}{P'} &\equiv_{\alpha}
  		\B{k+1}{\tilde y'\sigma}{P'\incrname{u}{i}}
  	\end{align*}

  	Next, we comment the case when $u_i \notin \wtd x$. 
  	In this case $\Delta_1 = \Delta \setminus \widetilde x \cat 
  	u_i:\btinp{C}S$. Hence, in the right hand-side of 
    \eqref{pt:input} instead of $\Gt{\Delta_1}$ we would have 
    $\Gt{\Delta \setminus \widetilde x \cat 
  	u_{i+1}:S}$ and in the left-hand side we have 
  	$u_i : \btinp{\Gt{C}}\tinact$ as a linear environment. 
  	Then, we would need to apply \eqref{lem:subst}  with 
  	$\subst{u_{i}}{u_{i+1}}$ to right-hand side before 
  	invoking \eqref{eq:input-ih}. We remark that similar provisos apply  
  	to the following cases when the assumption is $u_i \notin \wtd x$.

   This concludes sub-case \rom{1}. We now consider sub-case \rom{2}, i.e.,
   $u_i \in \dom{\Gamma}$.
   Here Rule~\textsc{Acc} can be applied:
   \begin{align}
   	\label{pt:inputptr-subcase2}
   	\AxiomC{$\Gamma;\es \proves u_i \hastype \chtype{C}$}
   	\AxiomC{$\Gamma;\Delta \cat z : C \proves P' \hastype \Proc$}
  	\AxiomC{$\Gamma;z:C \proves z \hastype C$}
  	\LeftLabel{\scriptsize Acc}
   	\TrinaryInfC{$\Gamma;\Delta
   				    \proves \binp{u_i}{z}P' \hastype \Proc$}
   	\DisplayProof
   \end{align}

% Let $\widetilde x, \widetilde x', \widetilde y, \widetilde y'$,
%   $\Theta_1$, $\Theta$, $\Gamma_1$, and
%   $\Delta_1$  be defined as in sub-case
%   \rom{1}.
   By IH on the second assumption of \eqref{pt:inputptr-subcase2} we have:
   \begin{align}
   \label{eq:input-ih-2}
    \Gt{\Gamma'_1};\Gt{\Delta'_1} \cat \Theta_1 \proves \B{k+1}{\tilde y'}{P'} \hastype \Proc
   \end{align}
   
\noindent where $\wtd x'$ and $\wtd y'$ are as in sub-case \rom{1}. 
Also, $\Gamma'_1 = \Gamma \setminus \wtd x'$
and $\Delta'_1 = \Delta  \setminus \wtd y'$ 
and $\balan{\Theta_1}$ with
   $$
   \dom{\Theta_1}=\{\prop_{k+1},\ldots,\prop_{k+\lenHOopt{P'}}\}
   \cup \{\dual{\prop_{k+2}},\ldots,\dual{\prop_{k+\lenHOopt{P'}}}\}
   $$
   and ${\Theta_1(\prop_{k+1})}=\btinp{\widetilde M'}\tinact$
   where $\widetilde M' = (\Gt{\Gamma},\Gt{\Delta,z:C})(\widetilde y')$.

	By applying \lemref{lem:varbreak} to the first and third
   	assumptions of \eqref{pt:inputptr-subcase2} we have:
  	\begin{align}
  		\label{eq:input-ih2-2}
  		\Gt{\Gamma};\es \proves u_i \hastype \chtype{\Gt{C}}
\\
  		\label{eq:input-ih3-2}
  		\Gt{\Gamma};\Gt{z:C} \proves \wtd z \hastype \Gt{C}
  	\end{align}

    We define $\wtd x = \wtd x' \cup u \setminus z$ and $\wtd y = \wtd y' \cup u_i 
    \setminus \wtd z$ where $\len{\wtd z} = \len{\Gt{C}}$. 
    Notice that $\indexed{\wtd y}{\wtd x}{\Gamma,\Delta}$.
    Let $\Gamma_1 = \Gamma \setminus x$. 
    We define $\Theta = \Theta_1 \cat \Theta'$, where
  \begin{align*}
  \Theta' = \prop_k:\btinp{\widetilde M} \tinact \cat \dual {\prop_{k+1}}:\btout{\widetilde M'} \tinact
  \end{align*}
  with $\widetilde M = (\Gt{\Gamma},\Gt{\Delta})(\widetilde y)$.
  By \defref{def:sizeproc},
  $\lenHOopt{P} = \lenHOopt{P'} + 1$ so
  $$\dom{\Theta} = \{\prop_k,\ldots,\prop_{k+\lenHOopt{P}-1}\}
  	\cup \{\dual{\prop_{k+1}},\ldots,\dual{\prop_{k+\lenHOopt{P}-1}}\}$$
  	and $\Theta$ is balanced since $\Theta(\prop_{k+1}) \dualof \Theta(\dual{\prop_{k+1}})$ and
  	 $\Theta_1$ is balanced.

 	By \tabref{t:bdowncorec}, we have:
 	\begin{align}
  		\B{k}{\tilde y}{\binp{u_i}{z}P'} = \propinp{k}{\widetilde y}
  		\binp{u_i}{z}\propout{k+1}{\widetilde y'} \inact \Par \B{k+1}{\tilde y'}
  		{P'}
 	\end{align}

 	We shall prove the following judgment:
 	\begin{align}
 		\Gt{\Gamma_1};\Gt{\Delta_1} \cat \Theta \proves
 		\B{k}{\tilde y}{\binp{u_i}{z}P'} \hastype \Proc
 	\end{align}

	To this end, we use some auxiliary derivations: 
	\begin{align}
		\label{st:input1-3}
    \AxiomC{}
    \LeftLabel{\scriptsize Nil}
    \UnaryInfC{$\Gt{\Gamma};\es;\es \proves \inact \hastype \Proc$}
    \LeftLabel{\scriptsize End}
    \UnaryInfC{$\Gt{\Gamma};\es;\dual{\prop_{k+1}}:\tinact \proves \inact \hastype \Proc$}
    \DisplayProof
	\end{align}

  \begin{align}
    %\gamma
    \label{st:input1-2}
%    \AxiomC{}
%    \LeftLabel{\scriptsize Nil}
%    \UnaryInfC{$\Gt{\Gamma};\es;\es \proves \inact \hastype \Proc$}
%    \LeftLabel{\scriptsize End}
%    \UnaryInfC{$\Gt{\Gamma};\es;\dual{\prop_{k+1}}:\tinact \proves \inact \hastype \Proc$}
\AxiomC{\eqref{st:input1-3}} 
    \AxiomC{}
    \LeftLabel{\scriptsize PolyVar}
    \UnaryInfC{$\Gt{\Gamma};\Gt{\Delta_2} \cat z : \Gt{C}
                \proves \widetilde y' \hastype \widetilde M'$}
    \LeftLabel{\scriptsize PolySend}
    \BinaryInfC{$\Gt{\Gamma};
                  \dual {\prop_{k+1}}:\btout{\widetilde M'} \tinact
                  \cat \Gt{\Delta_2}
                  \cat z : \Gt{C}
                  \proves \propout{k+1}{\widetilde y'} \inact \hastype \Proc$}
    \DisplayProof
  \end{align}

  \begin{align}
    %beta
    \label{st:input2-2}
    \AxiomC{\eqref{eq:input-ih2-2}}
    \AxiomC{\eqref{st:input1-2}}
	\AxiomC{\eqref{eq:input-ih3-2}}
    \LeftLabel{\scriptsize PolyAcc}
    \TrinaryInfC{$\Gt{\Gamma};
    			\dual{\prop_{k+1}}:\btout{\widetilde M'} 
                 \tinact \cat \Gt{\Delta_2}
                 \proves \binp{u_i}{z}\propout{k+1}{\widetilde y'} \inact \hastype \Proc$}
     \LeftLabel{\scriptsize End}
    \UnaryInfC{$\Gt{\Gamma};
    			\dual{\prop_{k+1}}:\btout{\widetilde M'}
                 \tinact \cat \prop_k:\tinact 
                 	\cat \Gt{\Delta_2}
                 \proves \binp{u_i}{z}\propout{k+1}{\widetilde y'} \inact \hastype \Proc$}
    \DisplayProof
  \end{align}

  \begin{align}
    \label{st:input3-2}
    \AxiomC{\eqref{st:input2-2}}
    \AxiomC{}
    \LeftLabel{\scriptsize PolyVar}
    \UnaryInfC{$\Gt{\Gamma};
    \Gt{\Delta_2}
    \proves
    			\widetilde y \hastype \widetilde M$}
    \LeftLabel{\scriptsize PolyRcv}
    \BinaryInfC{$\Gt{\Gamma_1};\Theta' \proves
    				\propinp{k}{\widetilde y}
                  	\binp{u_i}{z}\propout{k+1}{\widetilde y'} \inact
                  	\hastype \Proc$}
    \DisplayProof
  \end{align}
  \noindent where $\Delta_2 = \Delta \setminus \Delta_1$.
Using \eqref{eq:input-ih-2} and \eqref{st:input3-2}, 
  the following tree
  proves this sub-case:
  \begin{align}
  	\label{pt:input-2}
    \AxiomC{\eqref{st:input3-2}}
    \AxiomC{\eqref{eq:input-ih-2}}
%    \LeftLabel{\scriptsize (\lemref{lem:strength}) with $y$}
%    \UnaryInfC{$\Gt{\Gamma_1 \setminus y};\es;\Gt{\Delta} \cat \Theta_1 \proves
%                	\B{k+1}{\tilde x'}{P'}$}
    \LeftLabel{\scriptsize Par}
    \BinaryInfC{$\Gt{\Gamma_1};\Gt{\Delta_1}
    \cat \Theta \proves
    \propinp{k}{\widetilde y}\binp{u_i}{z}
    \propout{k+1}{\widetilde y'}
    \inact \Par \B{k+1}{\tilde y'}{P'} \hastype \Proc$}
    \DisplayProof
  \end{align}
%   As in sub-case \rom{1}, we may notice that if $y \in \fv{P'}$ then $\Gamma'_1 = \Gamma_1 \setminus y$.
%   On the other hand, if $y \notin \fv{P'}$ then $\Gamma'_1 = \Gamma_1$ so we need to apply
%   \lemref{lem:strength} with $y$ to \eqref{eq:input-ih-2} in \eqref{pt:input-2}.
Note that if $u \notin \fn{P'}$ we need to apply 
\lemref{lem:strength}  with $u_i$ to the 
right assumption of \eqref{pt:input-2} before applying \eqref{eq:input-ih-2}. 
  This concludes the analysis of the input case.
%  $P = \binp{u_i}{z}P'$.

\item Case $P = \bout{u_i}{z_j}P'$. 
We distinguish two
  sub-cases: \rom{1} $u_i \in \dom{\Delta}$ and \rom{2} $u_i \in \dom{\Gamma}$.
  We consider sub-case \rom{1} first. For this case Rule~\textsc{Send} can be applied:
  \begin{align}
    \label{pt:outputitr}
    \AxiomC{$\Gamma;\Delta_1 \cat  u_i:S \proves P' \hastype \Proc$}
    \AxiomC{$\Gamma;\Delta_z \proves z_j \hastype C$}
    \AxiomC{$u_i:S \in \Delta$}
    \LeftLabel{\scriptsize Send}
    \TrinaryInfC{$\Gamma;\Delta
                  \proves \bout{u_i}{z_j}P' \hastype \Proc$}
    \DisplayProof
  \end{align}
    \noindent where $\Delta = \Delta_1 \cat\Delta_z
                  \cat u_i:\btout{C}S$.

  	By IH on the first assumption of \eqref{pt:outputitr} we have:
  	\begin{align}
  		\label{eq:output-ih-1}
    	\Gt{\Gamma'_1};\Gt{\Delta'_1 } \cat \Theta_1 \proves
    	\B{k+1}{\tilde y'}{P'} \hastype \Proc
  	\end{align}
	\noindent where $\widetilde x' \subseteq \fv{P'}$ 
	and $\widetilde y'$ such that 
	$\indexed{\widetilde y'}{\widetilde x'}{\Gamma,\Delta_1 \cat u_i:S}$. 
	 Also, $\Gamma'_1 =
	\Gamma \setminus \widetilde y'$, 
	$\Delta'_1 = \Delta_1 \setminus \widetilde y'$, and $\balan{\Theta_1}$ 
	with
	$$
	\dom{\Theta_1}=\{\prop_{k+1},\ldots,\prop_{k+\lenHOopt{P'}}\}\cup
	\{\dual{\prop_{k+2}},\ldots,\dual{\prop_{k+\lenHOopt{P'}}}\}
	$$
	and $\Theta_1(\prop_{k+1})=\btinp{\widetilde M_1}\tinact$ where
	$\widetilde M_1 =
	(\Gt{\Gamma},\Gt{\Delta_1, u_i:S})(\widetilde y')$.
  	
  	By \lemref{lem:varbreak} and the first
   	assumption of \eqref{pt:outputitr} we have:
   	\begin{align}
   		\label{eq:output-ih2}
   		\Gt{\Gamma};\Gt{\Delta_z} \proves \widetilde z \hastype \Gt{C}
   	\end{align}

	\noindent where $\wtd z = (z_j,\ldots,z_{j+\len{\Gt{C}}-1})$.
	We assume $\wtd x = \wtd x',u, z$. Since 
	$\wtd x' \subseteq \fn{P'}$ follows that  
   $\widetilde x \subseteq \fn{P}$.
   Let $\wtd y = \wtd y'\sigma, u_i, \wtd z$ where 
   $\sigma = \subst{\wtd n}{\wtd u}$ with $\widetilde n =
  	(u_{i+1},\ldots,u_{i+\len{\Gt{S}}})$ and $\widetilde u =
  	(u_i,\ldots,u_{i+\len{\Gt{S}}-1})$. We have
  	$\wtd z = \fnb{z}{\wtd y}$. 
%   $\len{\wtd z} = \len{\Gt{C}}$. 
   By \defref{def:indexed} follows that  
   $\indexed{\wtd y}{\wtd x}{\Gamma, \Delta}$. 
  	We define $\Theta = \Theta_1 \cat \Theta'$, where:
  	\begin{align*}
    	\Theta' = \prop_{k}: \btinp{\widetilde M} \tinact \cat
    	\dual{\prop_{k+1}}:\btout{\widetilde M_1} \tinact
  	\end{align*}

  \noindent with $\widetilde M = (\Gt{\Gamma}\cat \Gt{\Delta})(\widetilde y)$. By \defref{def:sizeproc}, we know $\lenHOopt{P} =\lenHOopt{P'} + 1$, so
  $$
  \dom{\Theta}=\{\prop_k,\ldots,\prop_{k+\lenHOopt{P}-1}\} \cup
  \{\dual{\prop_{k+1}},\ldots,\dual{\prop_{k+\lenHOopt{P}-1}}\}
  $$
  and $\Theta$ is balanced since $\Theta(\prop_{k+1}) 
  \dualof \Theta(\dual{\prop_{k+1}})$ and $\Theta_1$ is 
  balanced. 

  By \tabref{t:bdowncorec}, we have:
  \begin{align*}
    \B{k}{\tilde y}{\bout{u_i}{z}P'} =
    \propinp{k}{\widetilde y}
    \bbout{u_i}{\wtd z} \propout{k+1}{\widetilde y'\sigma}
    \inact \Par
    \B{k+1}{\tilde y'\sigma}{P'\incrname{u}{i}}
  \end{align*}
% \noindent where $\len{\wtd z}=\len{\Gt{C}}$. 
Let $\Gamma_1 = \Gamma \setminus \widetilde x = \Gamma'_1$ 
 and $\Delta \setminus \wtd x = \Delta'_1$.

 We shall prove the following judgment:
 \begin{align}
    \AxiomC{$\Gt{\Gamma_1}; \Gt{\Delta'_1} \cat \Theta \proves
    \B{k}{\tilde y}{\bout{u_i}{z}P'} \hastype \Proc$}
    \DisplayProof
  \end{align}
%   \noindent where we may notice that following holds: 
  
%   $$\Delta'_1 = \Delta \setminus \wtd y' = (\Delta_1 \cat u_i:\btout{C}S \cat \Delta_z) \setminus \widetilde y $$

  To type the sub-process $ \propinp{k}{\widetilde y}
    \bbout{u_i}{\wtd z} \propout{k+1}{\widetilde y'}
    \inact$ of
  $\B{k}{\tilde y}{\bout{u_i}{z}P'}$
  we use some auxiliary derivations:
  
  \begin{align}
  	\label{pt:send2}
  	\AxiomC{}
  	\LeftLabel{\scriptsize Nil}
  	\UnaryInfC{$\Gt{\Gamma};\es \proves \inact \hastype \Proc$}
  	\LeftLabel{\scriptsize End}
  	\UnaryInfC{$\Gt{\Gamma};\dual{\prop_{k+1}} : \tinact \proves \inact \hastype \Proc$}
  	\DisplayProof
  \end{align}

  \begin{align}
  	\label{pt:zsend}
%  	\AxiomC{}
%  	\LeftLabel{\scriptsize Nil}
%  	\UnaryInfC{$\Gt{\Gamma};\es \proves \inact \hastype \Proc$}
%  	\LeftLabel{\scriptsize End}
%  	\UnaryInfC{$\Gt{\Gamma};\dual{\prop_{k+1}} : \tinact \proves \inact \hastype \Proc$}
\AxiomC{\eqref{pt:send2}} 
  	\AxiomC{}
  	\LeftLabel{\scriptsize PolyVar}
  	\UnaryInfC{$\Gt{\Gamma};\Gt{\Delta_1 \cat u_{i+1}:S \setminus \Delta'_1}
  				\proves \widetilde y'\sigma \hastype \widetilde M_1$}
  	\LeftLabel{\scriptsize PolySend}
  	\BinaryInfC{
  	\begin{tabular}{c}
  	$\Gt{\Gamma};
  				\dual{\prop_{k+1}}:\btout{\widetilde M_1} \tinact
  					\cat \Gt{\Delta_1 \cat u_{i+1}:S \setminus \Delta'_1}
  				\proves$ \\ $\bout{\dual {\prop_{k+1}}}{\widetilde y'\sigma} 
  				\hastype \Proc$
  				\end{tabular}}
  	\LeftLabel{\scriptsize End}
  	\UnaryInfC{
  	\begin{tabular}{c}$\Gt{\Gamma};
  				\dual{\prop_{k+1}}:\btout{\widetilde M_1} 
  				 \tinact
  				\cat u_i:\tinact
  				\cat \Gt{\Delta_1 \cat u_{i+1}:S \setminus \Delta'_1}
  				\proves$ \\ $\bout{\dual {\prop_{k+1}}}{\widetilde y'\sigma} \inact
  				\hastype \Proc$
  				\end{tabular}}
  	\DisplayProof
  \end{align}

  \begin{align}
  	\label{pt:uisend}
  	\AxiomC{\eqref{pt:zsend}}
  	\AxiomC{\eqref{eq:output-ih2}}
%  	\LeftLabel{\scriptsize \lemref{lem:subst} with $\subst{\tilde z_1}{\tilde z}$}
%  	\UnaryInfC{$\Gt{\Gamma};\Gt{\Delta_z \subst{\tilde z}{\tilde z_1}} \proves \widetilde z \hastype \Gt{C}$}
  	\LeftLabel{\scriptsize Send}
  	\BinaryInfC{\begin{tabular}{c}
  				$\Gt{\Gamma};
  				\Gt{\Delta \setminus \Delta'_1}
  			      	\cat
  			       	\dual{\prop_{k+1}}:\btout{\widetilde M_1}\tinact
  			       	\proves$ \\
  			       	$\bbout{u_i}{\widetilde z}
                 	\propout{k+1}{\widetilde y'} \inact \hastype \Proc$
                 	\end{tabular}}
    	\LeftLabel{\scriptsize End}
  	\UnaryInfC{\begin{tabular}{c}
  				$\Gt{\Gamma};
  				\Gt{\Delta \setminus \Delta'_1}
  			      	 \cat
  			       	\dual{\prop_{k+1}}:\btout{\widetilde M_1}\tinact \cat \prop_k:\tinact 
  			       	\proves$ \\
  			       	$\bbout{u_i}{\wtd z}
                 	\propout{k+1}{\wtd y'} \inact \hastype \Proc$
                 	\end{tabular}}
  	\DisplayProof
  \end{align}
  % TODO continue updating proof here 
  \begin{align}
  \label{pt:stvalue}
  \AxiomC{\eqref{pt:uisend}}
  \AxiomC{}
  \LeftLabel{\scriptsize PolyVar}
  \UnaryInfC{$\Gt{\Gamma};\Gt{\Delta \setminus \Delta_1'} \proves
  				\widetilde y : \widetilde M$}
  \LeftLabel{\scriptsize PolyRcv}
  \BinaryInfC{\begin{tabular}{c}
  				$\Gt{\Gamma_1};
                 \Theta'
     	        \proves$ \\
     	        $\propinp{k}{\widetilde y}
  		        \bbout{u_i}{\wtd z}
                \propout{k+1}{\wtd y'} \inact
                \hastype \Proc$
                \end{tabular}}
  \DisplayProof
  \end{align}
%    \noindent where $\Delta_3 = \Delta \setminus \Delta_2$. 
  Using \eqref{eq:output-ih-1} and \eqref{pt:stvalue}, the following tree proves this case:
  \begin{align}
    \label{pt:output1}
    \AxiomC{\eqref{pt:stvalue}}
    \AxiomC{\eqref{eq:output-ih-1}}
    % \LeftLabel{\scriptsize (\lemref{lem:subst}) with $\subst{\tilde n}{\tilde u}$}
    % \UnaryInfC{$\Gt{\Gamma'_1};\Gt{\Delta'_1} \cat \Theta_1
    %             \proves \B{k+1}{\tilde y'}{P'\sigma} \hastype \Proc$}
    % \LeftLabel{\scriptsize (\lemref{lem:strength}) with $\tilde z$}
    \UnaryInfC{$\Gt{\Gamma_1};\Gt{\Delta'_1} \cat
    			\Theta_1 \proves
                \B{k+1}{\tilde y'\sigma}{P'\incrname{u}{i}} \hastype \Proc$}
     \LeftLabel{\scriptsize Par}
    \BinaryInfC{$\Gt{\Gamma_1}; \Gt{\Delta'_1} \cat \Theta \proves
                  \B{k}{\tilde y}{\bout{u_i}{z}P'} \hastype \Proc$}
    \DisplayProof
  \end{align}
  
    	Note that we have used the following for the right assumption of \eqref{pt:input}:
  	\begin{align*}
  		% \Gt{\Delta'_1 \cat u_i:S}\subst{\tilde n}{\tilde u} &=
  		% \Gt{\Delta'_1 \cat u_{i+1}:S} \\
  		\B{k+1}{\tilde y'}{P'} &\equiv_{\alpha}
  		\B{k+1}{\tilde y'\sigma}{P'\incrname{u}{i}}
  	\end{align*}

%  In this case $u_i \notin \wtd x$ we would have to 
%%  apply substitution $\subst{u_{i+1}}{u_{i}}$ to $\Gamma_1$
%apply \lemref{lem:subst} with 
%$\subst{u_{i+1}}{u_{i}}$

  %   \noindent where $\widetilde n =
%   (u_{i+1},\ldots,u_{i+\len{\Gt{S}}})$ and $\widetilde u =
%   (u_i,\ldots,u_{i+\len{\Gt{S}}-1})$.

  We now consider sub-case \rom{2}. For this sub-case Rule~\textsc{Req}
		can be applied:

   \begin{align}
   	\label{pt:outputitr-2}
   	\AxiomC{$\Gamma;\es \proves u \hastype \chtype{C}$}
   	\AxiomC{$\Gamma;\Delta_1 \hastype P' \hastype \Proc$}
  	\AxiomC{$\Gamma;\Delta_z \proves z \hastype C$}
  	\LeftLabel{\scriptsize Req}
   	\TrinaryInfC{$\Gamma;\Delta_1 \cat \Delta_z \proves \bout{u_i}{z}P' \hastype \Proc$}
   	\DisplayProof
   \end{align}

   Let $\widetilde x' \subseteq \fn{P'}$ and 
   $\wtd y$ such that $\indexed{\wtd y'}{\wtd x'}{\Gamma, \Delta_1}$
   . Further, let $\Gamma'_1 =
   \Gamma \setminus \widetilde x'$ and
   $\Delta'_1 = \Delta_1 \setminus \wtd x'$.
    Also, let $\Theta_1$ be
     environment defined as in sub-case \rom{1}.
%TODO dfdfdok

  By IH on the second assumption of \eqref{pt:outputitr-2} we have:
  \begin{align}
  	\label{eq:output-ih-1-2}
    \Gt{\Gamma_1'};\Gt{\Delta'_1} \cat \Theta_1 \proves
    \B{k+1}{\tilde y'}{P'} \hastype \Proc
  \end{align}

	By \lemref{lem:varbreak} and the first and third
   	assumptions of \eqref{pt:outputitr-2} we have:
   	\begin{align}
   		\label{eq:output-ih-2-1}
   		\Gt{\Gamma};\es \proves u_i \hastype \Gt{\chtype{C}}
\\
   		\label{eq:output-ih-2}
   		\Gt{\Gamma};\Gt{\Delta_z} \proves \widetilde z \hastype \Gt{C}
   	\end{align}

%  % need to construct \Theta
%  Let $\widetilde x = \fv{P}$ and $\Gamma_1 = \Gamma \setminus \widetilde x$.
%  We define $\Theta = \Theta_1 \cat \Theta_2 \cat \Theta'$, where:
%  \begin{align*}
%    \Theta' = \prop_{k}: \btinp{\widetilde M} \tinact \cat
%    \dual{\prop_{k+r+1}}:\btout{\widetilde M_2} \tinact
%  \end{align*}
%    \noindent with
%  $\widetilde M = (\Gt{\Gamma}\cat \Gt{\Lambda})(\widetilde x)$.
%  By \defref{def:sizeproc}, we know $\len{P} =
%  \len{V} + \len{P'} + 1$, so
%  $$\dom{\Theta}=(\prop_k,\ldots,\prop_{k+\len{P}-1}) \cup
%  (\dual{\prop_{k+1}},\ldots,\dual{\prop_{k+\len{P}-1}})$$
%  By construction $\Theta$ is balanced since $\Theta(\prop_{k+\degree+1}) \dualof \Theta(\dual{\prop_{k+\degree+1}})$ and
%  	 $\Theta_1$ and $\Theta_2$ are balanced.

We define $\wtd x = \wtd x' \cup z \cup u$ and 
$\wtd y = \wtd y' \cup \wtd z \cup u_i$ where $\len{\wtd z} = \len{\Gt{C}}$. 
    Notice that $\indexed{\wtd y}{\wtd x}{\Gamma,\Delta}$.
    Let $\Gamma_1 = \Gamma \setminus \wtd x = \Gamma'_1 \setminus u$
    and $\Delta \setminus \wtd x = \Delta'_1$.
% We define $\widetilde x$, $\wtd y$, and $\Theta$ as in sub-case
% \rom{1}. 

  By \tabref{t:bdowncorec}, we have:
\begin{align*}
  \B{k}{\tilde y}{\bout{u_i}{z}P'} =
  \propinp{k}{\widetilde y}
  \bbout{u_i}{\wtd z} \propout{k+1}{\widetilde y'} \inact \Par
  \B{k+1}{\tilde y'}{P'}
\end{align*}

  We shall prove the following judgment: 
  $$\Gt{\Gamma_1};\Gt{\Delta'_1} \cat \Theta
                  \proves \B{k}{\tilde y}{\bout{u_i}{z}P'}$$
  We use some auxiliary derivations:
  \begin{align}
  	\label{pt:zsend-2}
  	\AxiomC{}
  	\LeftLabel{\scriptsize Nil}
  	\UnaryInfC{$\Gt{\Gamma};\es;\es \proves \inact \hastype \Proc$}
  	\LeftLabel{\scriptsize End}
  	\UnaryInfC{$\Gt{\Gamma};\es;\dual{\prop_{k+1}}:\tinact \proves \inact \hastype \Proc$}
  	\AxiomC{}
  	\LeftLabel{\scriptsize PolyVar}
  	\UnaryInfC{$\Gt{\Gamma}; \Gt{\Delta_1\setminus \Delta'_1}
  				\proves \widetilde y' : \wtd M_1$}
  	\LeftLabel{\scriptsize PolySend}
  	\BinaryInfC{$\Gt{\Gamma}; \Gt{\Delta_1 \setminus \Delta'_1} \cat
  				\dual{\prop_{k+1}}:\btout{\widetilde M_1} \tinact
  				\proves \bout{\dual {\prop_{k+1}}}{\widetilde y'} \inact \hastype \Proc$}
  	\DisplayProof
  \end{align}

    % \begin{align}
    %     \AxiomC{} 
    %     \UnaryInfC{}
    % \end{align}

  \begin{align}
  	\label{pt:uisend-2}
  	\AxiomC{\eqref{eq:output-ih-2-1}} 
  	\AxiomC{\eqref{pt:zsend-2}}
%  	\AxiomC{$\Gamma;\wtd z:\Gt{C} \proves \wtd z \hastype \Gt{C}$}
\AxiomC{\eqref{eq:output-ih-2}} 
  	\LeftLabel{\scriptsize PolyReq}
  	\TrinaryInfC{$\Gt{\Gamma};
  	\Gt{\Delta_1 \setminus \Delta'_1}
  			\cat 
  			\dual{\prop_{k+1}}:\btout{\widetilde M_1} \tinact
  			\cat \wtd z : \Gt{C}
  			\proves \bbout{u_i}{\wtd z}
  			\propout{k+1}{\widetilde y'} \inact \hastype \Proc$}
  	\DisplayProof
  \end{align}

  \begin{align}
  \label{pt:stvalue-2}
  \AxiomC{\eqref{pt:uisend-2}}
  \AxiomC{}
  \LeftLabel{\scriptsize PolyVar}
  \UnaryInfC{$\Gt{\Gamma};
  \Delta_1 \setminus \Delta_1' \cat \wtd z:\Gt{C}
            \proves
  			\widetilde y \hastype \widetilde M$}
  \LeftLabel{\scriptsize PolyRcv}
  \BinaryInfC{$\Gt{\Gamma_1};
  		\Theta'
     	\proves \propinp{k}{\widetilde y}
  		\bbout{u_i}{\wtd z} \propout{k+1}{\widetilde y'} \inact \hastype \Proc$}
  \DisplayProof
  \end{align}

  The following tree proves this case:
  \begin{align}
    \label{pt:output1-2}
    \AxiomC{\eqref{pt:stvalue-2}}
    \AxiomC{\eqref{eq:output-ih-1-2}}
    \LeftLabel{\scriptsize}
    \UnaryInfC{$\Gt{\Gamma_1};\Gt{\Delta'_1} \cat \Theta_1 \proves
    \B{k+1}{\tilde y'}{P'} \hastype \Proc$}
     \LeftLabel{\scriptsize Par}
    \BinaryInfC{$\Gt{\Gamma_1};\Gt{\Delta'_1} \cat \Theta
                  \proves \B{k}{\tilde y}{\bout{u_i}{z}P'} \hastype \Proc$}
    \DisplayProof
  \end{align}
  We remark that if $u_i \notin \fn{P'}$ we need to apply 
\lemref{lem:strength}  with $u_i$ to the 
right assumption of \eqref{pt:output1-2} before applying \eqref{eq:output-ih-1-2}. 
 This concludes the analysis for the output case $P = \bout{u_i}{z}P'$.

\item Case $P = \news{s:C}P'$. We distinguish two sub-cases:
\rom{1} $C = S$ and \rom{2} $C = \chtype{C}$. 
First, we $\alpha$-convert $P$ as follows:
\begin{align*}
	P \equiv_{\alpha} \news{s_1:C}P'\subst{s_1 \dual{s_1}}{s \dual{s}}
\end{align*}

We consider sub-case \rom{1} first. For this case Rule~\textsc{ResS} can be applied:
\begin{align}
	\label{pt:restritr}
	\AxiomC{$\Gamma;\Delta \cat s_1:S \cat \dual {s_1}:\dual S
				\proves P'\subst{s_1 \dual{s_1}}{s \dual{s}} \hastype \Proc$}
	\LeftLabel{\scriptsize ResS}
	\UnaryInfC{$\Gamma;\Delta \proves
              \news{s_1:S}P'\subst{s_1 \dual{s_1}}{s \dual{s}} \hastype \Proc$}
	\DisplayProof
\end{align}

By IH on the assumption of \eqref{pt:restritr} we have:
\begin{align}
	\label{eq:restr-ih}
	\Gt{\Gamma \setminus \wtd x};\Gt{\Delta \setminus \wtd x \cat s_1:S \cat \dual {s_1}:\dual S}
				\cat \Theta_1 \proves
				\B{k}{\tilde y}{P'\subst{s_1 \dual{s_1}}{s \dual{s}}} \hastype \Proc
\end{align}
\noindent where 
$\widetilde x \subseteq \fn{P'}$
such that $s_1,\dual{s_1} \notin \wtd x$ and 
$\wtd y$ such that $\indexed{\wtd y}{\wtd x}{\Gamma,\Delta}$.
%where $\Delta' = \Delta \cat s_1:S \cat \dual {s_1}:\dual S$.
Also, $\balan{\Theta_1}$ with
$$
\dom{\Theta_1}=\{\prop_k,\ldots,\prop_{k+\lenHOopt{P'}-1}\}
\cup \{\dual{\prop_{k+1}},\ldots,\dual{\prop_{k+\lenHOopt{P'}-1}}\}
$$
and $\Theta_1(\prop_k) =
\btinp{\widetilde M} \tinact$ with $\widetilde M =
(\Gt{\Gamma}\cat\Gt{\Delta})(\widetilde y)$.

Note that we take $\Theta = \Theta_1$ since $\lenHOopt{P}=\lenHOopt{P'}$. By \defref{def:typesdecomp} and \defref{def:typesdecompenv} and~\eqref{eq:restr-ih}, we know that:
\begin{align}
	\label{eq:restr-ih1}
	\Gt{\Gamma \setminus \wtd x};\Gt{\Delta \setminus \wtd x} \cat \widetilde s:\Gt{S} \cat	\dual{\widetilde s}:
  \Gt{\dual S} \proves \B{k}{\tilde y}{P'\subst{s_1 \dual{s_1}}{s \dual{s}}}
	\hastype \Proc
\end{align}
\noindent where $\widetilde s = (s_1,\ldots,s_{\len{\Gt{S}}})$ and
$\dual{\widetilde s} = (\dual{s_1},\ldots,\dual{s_{\len{\Gt{S}}}})$.
By \tabref{t:bdowncorec}, we have:
\begin{align*}
	\B{k}{\tilde y}{\news{s}P'} = \news{\widetilde s : \Gt{S}}
								\B{k}{\tilde y}{P'\subst{s_1 \dual{s_1}}{s \dual{s}}}
\end{align*}

The following tree proves this sub-case:
\begin{align}
	\label{pt:restr1}
	\AxiomC{\eqref{eq:restr-ih1}}
	\LeftLabel{\scriptsize PolyResS}
	\UnaryInfC{$\Gt{\Gamma \setminus \wtd x};\Gt{\Delta \setminus \wtd x} \proves
				\news{\widetilde s : \Gt{S}}
				\B{k}{\tilde y}{P'\subst{s_1 \dual{s_1}}{s \dual{s}}} \hastype \Proc$}
	\DisplayProof
\end{align}

We now consider sub-case \rom{2}. Similarly to sub-case \rom{1} we first $\alpha$-convert $P$ as
follows:
\begin{align*}
	P \equiv_\alpha \news{s_1}{P'\subst{s_1}{s}}
\end{align*}

For this sub-case Rule~\textsc{Res} can be applied:
\begin{align}
	\label{eq:restritr2}
	\AxiomC{$\Gamma \cat s_1:\chtype{C};\Delta \proves
            P'\subst{s_1}{s} \hastype \Proc$}
	\LeftLabel{\scriptsize Res}
	\UnaryInfC{$\Gamma;\Delta \proves \news{s_1}P'\subst{s_1}{s}
					\hastype \Proc$}
	\DisplayProof
\end{align}

By IH on the
first assumption of \eqref{eq:restritr2} we have:
\begin{align}
	\label{eq:restr-ih2}
	\Gt{\Gamma \setminus \wtd x \cat s_1:\chtype{C}};\Gt{\Delta \setminus \wtd x}
		\cat \Theta_1
		\proves \B{k}{\tilde y}{P'\subst{s_1}{s}} \hastype \Proc
\end{align}

\noindent where 
$\widetilde x \subseteq \fn{P'}$
such that $s_1 \notin \wtd x$ and 
$\wtd y$ such that $\indexed{\wtd y}{\wtd x}{\Gamma,\Delta}$.
Also, $\balan{\Theta_1}$ with
$$
\dom{\Theta_1}=\{\prop_k,\ldots,\prop_{k+\lenHOopt{P'}-1}\}
\cup \{\dual{\prop_{k+1}},\ldots,\dual{\prop_{k+\lenHOopt{P'}-1}}\}
$$
and $\Theta_1(\prop_k) =
\btinp{\widetilde M} \tinact$ with $\widetilde M =
(\Gt{\Gamma}\cat\Gt{\Delta})(\widetilde y)$.

Here we also take $\Theta = \Theta_1$ since  $\lenHOopt{P}=\lenHOopt{P'}$.
We notice that by \defref{def:typesdecomp} and \defref{def:typesdecompenv} and
\eqref{eq:restr-ih2}:
\begin{align}
	\label{eq:restr-ih3}
	\Gt{\Gamma \setminus \wtd x} \cat s_1:\Gt{\chtype{C}};\Gt{\Delta \setminus \wtd x}
		\cat \Theta_1
		\proves \B{k}{\tilde y}{P'\subst{s_1}{s}} \hastype \Proc
\end{align}

By \tabref{t:bdowncorec}, we have:
\begin{align*}
	\B{k}{\tilde y}{\news{s}P'} = \news{s_1 : \Gt{\chtype{C}}}
								\B{k}{\tilde y}{P'\subst{s_1}{s}}
\end{align*}
%\noindent where $\widetilde s = s_1$ since $\len{\Gt{\chtype{U}}}=1$.
The following tree proves this sub-case:
\begin{align}
	\AxiomC{\eqref{eq:restr-ih3}}
	\LeftLabel{\scriptsize PolyRes}
	\UnaryInfC{$\Gt{\Gamma \setminus \wtd x};\Gt{\Delta \setminus \wtd x}\cat \Theta
					\proves \news{s_1 : \Gt{\chtype{C}}}
								\B{k}{\tilde y}{P'\subst{s_1}{s}} \hastype \Proc$}
	\DisplayProof
\end{align}

\item Case $P = Q \Par R$. For this case only Rule~\textsc{Par} can be applied:
\begin{align}
	\label{pt:compitr}
	\AxiomC{$\Gamma;\Delta_1 \proves Q \hastype \Proc$}
	\AxiomC{$\Gamma;\Delta_2 \proves R \hastype \Proc$}
	\LeftLabel{\scriptsize Par}
	\BinaryInfC{$\Gamma;\Delta_1 \cat \Delta_2
					     \proves Q \Par R \hastype \Proc$}
	\DisplayProof
\end{align}

By IH on the first assumption of \eqref{pt:compitr} we have:
\begin{align}
	\label{eq:comp-ih-1}
	\Gt{\Gamma'_1};\Gt{\Delta'_1} \cat \Theta_1 \proves
  \B{k+1}{\tilde y_1}{Q} \hastype \Proc
\end{align}

\noindent where 
$\widetilde x_1 \subseteq \fn{Q}$ and 
$\widetilde y_1$ such that $\indexed{\widetilde y_1}{\wtd x_1}{\Gamma,\Delta_1}$. 
Also, $\Gamma'_1 = \Gamma \setminus \wtd x_1$, 
$\Delta'_1 = \Delta_1 \setminus \wtd x_1$, 
and $\balan{\Theta_1}$ with
$$\dom{\Theta_1}=\{\prop_{k+1},\ldots,\prop_{k+\lenHOopt{Q}}\}
\cup \{\dual{\prop_{k+2}},\ldots,\dual{\prop_{k+\lenHOopt{Q}}}\}
$$
and
$\Theta_1(\prop_{k+1}) = \btinp{\widetilde M_1} \tinact$ with $\widetilde M_1 =
(\Gt{\Gamma}\cat\Gt{\Delta_1})(\widetilde y_1)$.

By IH on the second assumption of \eqref{pt:compitr} we have:
\begin{align}
	\label{eq:comp-ih-2}
	\Gt{\Gamma'_2};\Gt{\Delta_2'} \cat \Theta_2 \proves
  \B{k+\degree+1}{\tilde y_2}{R} \hastype \Proc
\end{align}

\noindent where 
$\widetilde x_2 \subseteq \fn{R}$ and 
$\widetilde y_2$ such that $\indexed{\widetilde y_2}{\wtd x_2}{\Gamma,\Delta_2}$
and  
$\degree = |Q|$. Also, 
$\Gamma'_2 = \Gamma \setminus \wtd x_2$, 
$\Delta'_2 = \Delta_2 \setminus \wtd x_2$
and $\balan{\Theta_2}$ with
$$\dom{\Theta_2}=\{\prop_{k+\degree+1},\ldots,\prop_{k+\degree+\lenHOopt{R}}\}
\cup \{\dual{\prop_{k+\degree+2}},\ldots,\dual{\prop_{k+\degree+\lenHOopt{R}}}\}$$ and
$\Theta_2(\prop_{k+\degree+1}) = \btinp{\widetilde M_2} \tinact$ with $\widetilde M_2 =
(\Gt{\Gamma}\cat\Gt{\Delta_2})(\widetilde y_2)$.

We define $\wtd x = \wtd x_1 \cup \wtd x_2$. 
We may notice that $\wtd x \subseteq \fn{P}$ since 
$\fn{P} = \fn{Q} \cup \fn{R}$. 
Accordingly, we define $\wtd y = \wtd y_1, \wtd y_2$. 
By definition, $\indexed{\wtd y}{\wtd x}{\Gamma, \Delta_1 \cat \Delta_2}$ holds. 
Further, let $\widetilde M = (\Gt{\Gamma},\Gt{\Delta_1\cat\Delta_2})(\widetilde y)$. 
%$\wtd x_1 \subseteq \fn{Q}$ and $\wtd x_2 \subseteq \fn{R}$. 
%
%Let $\widetilde x = \fv{P}$ and $\widetilde M = (\Gt{\Gamma},\Gt{\Lambda_1\cat\Lambda_2})(\widetilde x)$.
%We may notice that $\widetilde M_i \subseteq \widetilde M$ for $i \in \{1,2\}$.
We define $\Theta = \Theta_1 \cat \Theta_2 \cat \Theta'$ where:
 \begin{align*}
	\Theta' = \prop_k:\btinp{\widetilde M} \tinact \cat
				\dual{\prop_{k+1}}:\btout{\widetilde M_1} \tinact
				\cat
				\dual{\prop_{k+\degree+1}}:\btout{\widetilde M_2} \tinact
\end{align*}

 By construction $\Theta$ is balanced since $\Theta(\prop_{k+1}) \dualof \Theta(\dual{\prop_{k+1}})$, $\Theta(\prop_{k+\degree+1}) \dualof \Theta(\dual{\prop_{k+\degree+1}})$, and
  	 $\Theta_1$ and $\Theta_2$ are balanced.

By \tabref{t:bdowncorec} we have:
\begin{align*}
  	\B{k}{\tilde y}{Q \Par R} =\propinp{k}{\widetilde y} \propout{k+1}{\widetilde y_1}
    \propout{k+\degree+1}{\widetilde y_2} \inact \Par
    \B{k+1}{\tilde y_1}{Q} \Par \B{k+\degree+1}{\tilde y_2}{R}
\end{align*}

We may notice that $\wtd y_1 = \fnb{Q}{\widetilde y}$
and $\wtd y_2 = \fnb{R}{\widetilde y}$ hold
by the construction of $\wtd y$. 
Let $\Gamma_1 = \Gamma \setminus \widetilde x$. We shall prove the following judgment:
\begin{align*}
\Gt{\Gamma_1};\Gt{\Delta'_1 \cat \Delta'_2}
                \cat \Theta \proves
                \propinp{k}{\widetilde y} \bout{\dual {\prop_{k+1}}}{\widetilde y_1}
   						  \bout{\dual {\prop_{k+\degree+1}}}{\widetilde y_2} \inact \Par
    					  \B{k+1}{\tilde y_1}{Q} \Par \B{k+\degree+1}{\tilde y_2}{R} \hastype \Proc
\end{align*}

To type  $\propinp{k}{\widetilde y} \propout{k+1}{\widetilde y_1}
    \propout{k+\degree+1}{\widetilde y_2} \inact$, we use some auxiliary derivations:
\begin{align}
	\label{pt:compsend2}
	\AxiomC{}
\LeftLabel{\scriptsize Nil}
	\UnaryInfC{$\Gt{\Gamma};\es \proves \inact$}
	\LeftLabel{\scriptsize End}
	\UnaryInfC{$\Gt{\Gamma};\dual{\prop_{k+\degree+1}}:\tinact \proves \inact$}
	\AxiomC{}
	\LeftLabel{\scriptsize PolyVar}
	\UnaryInfC{$\Gt{\Gamma};\Gt{\Delta_2} \cat 
				\proves \widetilde z \hastype \widetilde M_2$}
	\LeftLabel{\scriptsize PolySend}
	\BinaryInfC{$\Gt{\Gamma};\Gt{\Delta'_2} \cat 
				\dual{\prop_{k+\degree+1}}:\btout{\widetilde M_2}\tinact
				\proves \propout{k+\degree+1}{\widetilde z} \inact \hastype \Proc$}
	\LeftLabel{\scriptsize End}
	\UnaryInfC{$\Gt{\Gamma};\Gt{\Delta'_2} \cat 
				\dual{\prop_{k+\degree+1}}:\btout{\widetilde M_2}\tinact
				\cat \dual{\prop_{k+1}}:\tinact
				\proves \propout{k+\degree+1}{\widetilde z} \inact \hastype \Proc$}
	\DisplayProof
\end{align}

\begin{align}
	\label{pt:compsend1}
	\AxiomC{\eqref{pt:compsend2}}
	\AxiomC{}
	\LeftLabel{\scriptsize PolyVar}
	\UnaryInfC{$\Gt{\Gamma};\Gt{\Delta_1}
				\proves \widetilde y_1 \hastype \widetilde M_1$}
	\LeftLabel{\scriptsize PolySend}
	\BinaryInfC{\begin{tabular}{c}
	$\Gt{\Gamma};\Gt{\Delta'_1\cat\Delta'_2} \cat             \dual{\prop_{k+1}}:\btout{\widetilde M_1}\tinact \cat
				 \dual{\prop_{k+\degree+1}}:\btout{\widetilde M_2}\tinact
			     \proves$ \\
			     $\propout{k+1}{\widetilde y_1}
   			    \propout{k+\degree+1}{\widetilde y_2} \inact \hastype \Proc$
   			    \end{tabular}}
   	\LeftLabel{\scriptsize End}
   \UnaryInfC{\begin{tabular}{c}
	$\Gt{\Gamma};\Gt{\Delta'_1\cat\Delta'_2} \cat
                \dual{\prop_{k+1}}:\btout{\widetilde M_1}\tinact \cat
				 \dual{\prop_{k+\degree+1}}:\btout{\widetilde M_2}\tinact
				 \cat \prop_k:\tinact
			     \proves$ \\
			     $\propout{k+1}{\widetilde y_1}
   			    \propout{k+\degree+1}{\widetilde y_2} \inact \hastype \Proc$
   			    \end{tabular}}
	\DisplayProof
\end{align}

\begin{align}
	\label{pt:compinput1}
	\AxiomC{\eqref{pt:compsend1}}
	\AxiomC{}
	\LeftLabel{\scriptsize PolyVar}
	\UnaryInfC{$\Gt{\Gamma};\Gt{\Delta'_1\cat\Delta'_2}
				      \proves \widetilde x \hastype \widetilde M$}
	\LeftLabel{\scriptsize PolyRcv}
	\BinaryInfC{$\Gt{\Gamma_1};\Theta' \proves
					     \propinp{k}{\widetilde y}
					     \propout{k+1}{\widetilde y_1}
   						 \propout{k+\degree+1}{\widetilde y_2} \inact \hastype \Proc$}
	\DisplayProof
\end{align}

\begin{align}
	\label{pt:comp-par-1}
	\AxiomC{\eqref{eq:comp-ih-1}}
	\LeftLabel{\scriptsize (\lemref{lem:weaken}) with $\Gamma_1' \setminus \Gamma_1$}
	\UnaryInfC{$\Gt{\Gamma_1};\Gt{\Delta_1} \cat \Theta_1 \proves
  					\B{k+1}{\tilde y_1}{Q} \hastype \Proc$}
  	\DisplayProof
\end{align}

\begin{align}
	\label{pt:comp-par-2}
	\AxiomC{\eqref{eq:comp-ih-2}}
	\LeftLabel{\scriptsize (\lemref{lem:weaken}) with $\Gamma_2' \setminus \Gamma_1$}
	\UnaryInfC{$\Gt{\Gamma_1};\Gt{\Delta'_2} \cat \Theta_2 \proves
  					\B{k+\degree+1}{\tilde y_2}{R} \hastype \Proc$}
  	\DisplayProof
\end{align}

\begin{align}
	\label{pt:par}
	\AxiomC{\eqref{pt:comp-par-1}}
	\AxiomC{\eqref{pt:comp-par-2}}
	\LeftLabel{\scriptsize Par}
	\BinaryInfC{$\Gt{\Gamma_1};\Gt{\Delta'_1 \cat \Delta'_2} \cat
                \Theta_1 \cat \Theta_2 \proves
                \B{k+1}{\tilde y}{Q} \Par \B{k+\degree+1}{\tilde z}{R} \hastype \Proc$}
     \DisplayProof
\end{align}

The following tree proves this case:

\begin{align*}
	\AxiomC{\eqref{pt:compinput1}}
	\AxiomC{\eqref{pt:par}}
	\LeftLabel{\scriptsize Par}
	\BinaryInfC{
	\begin{tabular}{c}
	$\Gt{\Gamma_1};\Gt{\Delta'_1 \cat \Delta'_2}
                \cat \Theta \proves$ \\
                $\propinp{k}{\widetilde y}
                \bout{\dual {\prop_{k+1}}}{\widetilde y_1}
   						  \bout{\dual {\prop_{k+\degree+1}}}{\widetilde y_2} \inact \Par
    					  \B{k+1}{\tilde y_1}{Q} \Par \B{k+\degree+1}{\tilde y_2}{R} \hastype \Proc$
    					  \end{tabular}
    					  }
	\DisplayProof
\end{align*}

  \item Case $P = \recp{X}P'$. The only rule that can be 
  applied here is \textsc{Rec}:
  \begin{align}
  \label{pt:recInv}
    \AxiomC{$\Gamma \cat X : \Delta;\Delta \proves P' \hastype \Proc$} 
    \UnaryInfC{$\Gamma;\Delta \proves \recp{X}P'$} 
    \DisplayProof
  \end{align}
  
We remark that by \eqref{pt:recInv} we know 
$x:S \in \Delta \implies \mathsf{tr}(S)$.
Then, by applying \lemref{lem:brec} on the assumption of \eqref{pt:recInv} we have: 
\begin{align}
\label{pt:recIH}
\Gt{\Gamma \setminus \wtd x};\Theta 
 \proves \Brec{k+1}{\tilde y'}{P'}_g \hastype \Proc	
\end{align}

% \noindent where $g = \{X \mapsto \wtd m\}$
% with $\wtd n = \fn{P'}$ and $\wtd m = \bname{\wtd n : \wtd S}$.w
We take  $\wtd x' = \fn{P'}$, so we have 
  $\Delta \setminus x' = \emptyset$. Further, 
  $\wtd y'$ is such that 
  $\indexed{\wtd y'}{\wtd x'}{\Gamma,\Delta}$. 
Let  $\Theta' = \thetaR' \cat \thetax(g)$ with 
$\thetax(g) =  {\prop^r_{X}} : \chtype{\wtd M'}$ 
with $\wtd M' = (\Gt{\Gamma},\Gt{\Delta})(\wtd y')$.
Further,  $\wtd x' \subseteq P'$ and $\wtd y'$ such that 
  $\Delta \setminus x' = \emptyset$ and 
  $\indexed{\wtd y'}{\wtd x'}{\Gamma,\Delta}$. 
  Also, $\balan{\thetaR'}$ with 
$$\dom{\thetaR'} = \{\prop^r_{k+1},\ldots,\prop^r_{k+\lenHOopt{P'}} \} \cup 
 \{\dual{\prop^r_{k+1}},\ldots,\dual{\prop^r_{k+\lenHOopt{P'}}} \}$$ where
 $\thetaR' (\prop_{k+1})=\prop_k:\btinp{\wtd M'}\tinact$. 

Let $l = \lenHOopt{P'}$ and $\wtd z$ 
such that $\len{\wtd y'} = \len{\wtd z}$.
% We take $\wtd x = \wtd x'$ since $\fn{P} = \fn{P'}$.
% As $\Delta \setminus \wtd x = \emptyset$ we 
% have that $\wtd x' \supseteq \fn{P} \setminus \fs{P}$. 
% so we have $\wtd y'$ is properly defined. 
Further, let $\wtd x \subseteq \fn{P}$  
and $\wtd y = \bname{\wtd x : \wtd S}$. 
By definition we have $\wtd x \subseteq \wtd x'$. 
% We remark that by $\wtd x' = \fn{P}$ that 
% $\wtd y'$ is properly defined for this case. 
By \tabref{t:bdowncorec}, we have: 
\begin{align*}
  \B{k}{\tilde y}{P} &=
        \news{\prop^r_X}
        (\propinp{k}{\wtd y}
        \proproutk{r}{k+1}{\wtd y'}
        \recp{X}
        \proprinpk{r}{X}{\wtd z}
        \proproutk{r}{k+1}{\wtd z}X
      \Par 
       \Brec{k+1}{\tilde y'}{P'}_g)
\end{align*}
Let $\thetaR = \thetaR' \cdot \thetaR''$ where: 
$$\thetaR'' =  \dual{\prop^r_{k}} : \trec{t}\btinp{\wtd M}\tvar{t}
\cdot \dual{\prop^r_{k+1}} : \trec{t}\btout{\wtd M'}\tvar{t}$$

% Let $\Theta = \Theta' \cdot \thetaR''$ where: 
% $$\thetaR'' = 
% \prop^r_{k} \cdot
% \prop^r_{X} : \trec{t}\btinp{\wtd M}\tvar{t} 
% $$ 
% \noindent where $\wtd M = (\Gt{\Gamma}\cat\Gt{\Delta})(\widetilde y)$. 
%  By construction $\balan{\thetaR}$. 

% We know $\wtd x \subseteq \fn{P}$ since $\fn{P} = \fn{P'}$.
% We take $\wtd x = \wtd x'$ since $\fn{P} = \fn{P'}$.
% As $\Delta \setminus \wtd x = \emptyset$ we 
% have that $\wtd x \supseteq \fn{P} \setminus \fs{P}$. 
We shall prove the following judgment: 
\begin{align} 
  \Gt{\Gamma \setminus \wtd x}; \Gt{\Delta \setminus \wtd x}
  \cdot \envR \proves 	\B{k}{\tilde y}{P}
  \hastype \Proc
\end{align}

Let $\thetax' = \prop^r_{X} : \trec{t}\btinp{\wtd M'}\tvar{t}
\cdot \dual{\prop^r_{X}} : \trec{t}\btout{\wtd M'}\tvar{t}$. 
We use some auxiliary sub-trees: 

%	\begin{align}
%		\AxiomC{} 
%		\UnaryInfC{}
%		\DisplayProof	
%	\end{align}
%	
%	\begin{align}
%	\label{pt:rec4}
%		\AxiomC{} 
%		\LeftLabel{\scriptsize RVar}
%		\UnaryInfC{$\Gt{\Gamma \setminus \wtd x} \cat X : \Theta''; 
%		\Theta''
%		\proves 
%        	X
%		$}
%		\DisplayProof	
%	\end{align}

\begin{align}
\label{pt:rec4}
  \AxiomC{} 
  \LeftLabel{\scriptsize RVar}
  \UnaryInfC{$\Gt{\Gamma \setminus \wtd x} \cat X : \Theta''; 
  \Theta''
  \proves 
        X
        \hastype \Proc
  $}
  \AxiomC{} 
  \LeftLabel{\scriptsize PolyVar}
  \UnaryInfC{$\Gt{\Gamma \setminus \wtd x} \cat X : \Theta'';
  \Gt{\Delta} \proves 
  \wtd z \hastype \wtd M$} 
  \LeftLabel{\scriptsize Send}
  \BinaryInfC{$\Gt{\Gamma \setminus \wtd x} \cat X : \Theta'';
  \Gt{\Delta} \cat 
  \Theta''
  \proves 
  \proproutk{r}{k+1}{\wtd z}X
        \hastype \Proc
  $}	
  \DisplayProof
\end{align}

\begin{align}
  \label{pt:rec3}
\AxiomC{\eqref{pt:rec4}}
\AxiomC{} 
\LeftLabel{\scriptsize PolyVar}
\UnaryInfC{$\Gt{\Gamma \setminus \wtd x}; \Gt{\Delta} 
\proves \wtd z \hastype \wtd M$}
\LeftLabel{\scriptsize PolyRcv}
  \BinaryInfC{$\Gt{\Gamma \setminus \wtd x} \cat X : \Theta'';
  \Theta'' \proves 
  \binp{\prop^r_{X}}{\wtd z}
  \proproutk{r}{k+1}{\wtd z}X
        \hastype \Proc
  $} 
  \LeftLabel{\scriptsize Rec}
  \UnaryInfC{\begin{tabular}{c}
  $
  \Gt{\Gamma \setminus \wtd x}; 
  \Theta''
  \proves$ 
  % \\ 
  $
        \recp{X}\binp{\prop^r_{X}}{\wtd z}
        \proproutk{r}{k+1}{\wtd z}X
        \hastype \Proc$
        \end{tabular}}
  \DisplayProof	
\end{align}
\noindent where $\Theta'' = \dual{\prop^r_{k+1}} : \trec{t}\btout{\wtd M}\tvar{t}
\cat \prop^r_{X} : \trec{t}\btinp{\wtd M}\tvar{t}$.

\begin{align}
\label{pt:rec2}
  \AxiomC{\eqref{pt:rec3}} 
  \AxiomC{} 
  \LeftLabel{\scriptsize PolyVar}
  \UnaryInfC{$\Gt{\Gamma \setminus \wtd x}; 
  \Gt{\Delta} \proves 
  \wtd y' \hastype \wtd M'$} 
  \LeftLabel{\scriptsize PolySend}
  \BinaryInfC{
  \begin{tabular}{c}
  $
  \Gt{\Gamma \setminus \wtd x}; 
  \Gt{\Delta} \cat 
  \dual{\prop^r_{k+1}} : \trec{t}\btout{\wtd M}\tvar{t}
\cat \prop^r_{X} : \trec{t}\btinp{\wtd M}\tvar{t} 
  \proves$ 
  % \\ 
  $
        \bout{\prop^r_{k+1}}{\wtd y}
        \recp{X}\binp{\prop^r_{X}}{\wtd z}
        \proproutk{r}{k+1}{\wtd z}X
        \hastype \Proc$
        \end{tabular}}
  \DisplayProof
\end{align}

\begin{align}
\label{pt:rec1}
  \AxiomC{\eqref{pt:rec2}} 
  \AxiomC{} 
  \LeftLabel{\scriptsize PolyVar}
  \UnaryInfC{$\Gt{\Gamma \setminus \wtd x};
  \wtd y : \wtd M 
  \proves \wtd y \hastype \wtd M$} 
  \LeftLabel{\scriptsize PolyRcv}
  \BinaryInfC{$\Gt{\Gamma \setminus \wtd x}; 
  \Gt{\Delta \setminus \wtd x} \cdot 
  \thetaR'' \cdot \prop^r_{X} : \trec{t}\btinp{\wtd M}\tvar{t}
  \proves
  \propinp{k}{\wtd y}
  \proproutk{r}{k+1}{\wtd y'}
  \recp{X}
  \proprinpk{r}{X}{\wtd z}
  \proproutk{r}{k+1}{\wtd z}X
        \hastype \Proc$} 
  \DisplayProof
\end{align}

The following tree proves this case: 
\begin{align}
  \AxiomC{\eqref{pt:rec1}} 
%		\AxiomC{$\Gt{\Gamma \setminus \wtd x};  
%		\thetaR 
%		\proves
%		\Brec{k+1}{\tilde y'}{P'}$} 
\AxiomC{\eqref{pt:recIH}} 
  \LeftLabel{\scriptsize Par}
  \BinaryInfC{$
  \Gt{\Gamma \setminus \wtd x}; 
  \Gt{\Delta \setminus \wtd x} \cdot \thetaR \cdot \thetax'
  \proves \propinp{k}{\wtd y}
        \proproutk{r}{k+1}{\wtd y'}X
        \recp{X}\binp{\prop^r_{X}}{\wtd z}
        \proproutk{r}{k+1}{\wtd z}X
      \Par 
      \Brec{k+1}{\tilde y}{P'}
  \hastype \Proc$} 
  \LeftLabel{\scriptsize ResS}
\UnaryInfC{$
\Gt{\Gamma \setminus \wtd x}; 
\Gt{\Delta \setminus \wtd x} \cdot \thetaR
\proves \news{\prop^r_X}(\propinp{k}{\wtd y}
\proproutk{r}{k+1}{\wtd y'}X
      \recp{X}\binp{\prop^r_{X}}{\wtd z}
      \proproutk{r}{k+1}{\wtd z}X
    \Par 
    \Brec{k+1}{\tilde y'}{P'})
\hastype \Proc$}
  \DisplayProof	
\end{align}

\item Case $P = \bout{r}{z}P'$ when $\tr(r)$. 
For this case Rule~\textsc{Send} can be applied:
\begin{align}
  \label{pt:rec-outputitr}
  \AxiomC{$\Gamma;\Delta \cat  r:S' \proves P' \hastype \Proc$}
  \AxiomC{$\Gamma;\Delta_z \proves z \hastype C$}
  \AxiomC{}
  \LeftLabel{\scriptsize Send}
  \TrinaryInfC{$\Gamma;\Delta \cat 
  r : S \cat 
  \Delta_z
                \proves \bout{r}{z}P' \hastype \Proc$}
  \DisplayProof
\end{align}
  \noindent where $S = \btout{C}S'$.

  Then, by IH on the first assumption of \eqref{pt:rec-outputitr} we have:
  \begin{align}
    \label{eq:rec-output-ih-1}
    \Gt{\Gamma'_1};\Gt{\Delta'_1 } \cat \Theta_1 \proves
    \B{k+1}{\tilde y'}{P'} \hastype \Proc
  \end{align}
  \noindent where $\widetilde x' \subseteq \fn{P'}$ 
such that $r \in \wtd x'$ 
and $\widetilde y'$ such that 
$\indexed{\widetilde y'}{\widetilde x'}{\Gamma,\Delta \cat r:S}$. 
By this follows that $(r_1,\ldots,r_{\len{\Gt{S}}}) \subseteq \wtd y'$. 
 Also, $\Gamma'_1 =
\Gamma \setminus \widetilde x'$, 
$\Delta'_1 = \Delta \setminus \widetilde y'$, and $\balan{\Theta_1}$
with
$$
\dom{\Theta_1}=\{\prop_{k+1},\ldots,\prop_{k+\lenHOopt{P'}}\}\cup
\{\dual{\prop_{k+2}},\ldots,\dual{\prop_{k+\lenHOopt{P'}}}\}
$$
and $\Theta_1(\prop_{k+1})=\btinp{\widetilde M_1}\tinact$ where
$\widetilde M_1 =
(\Gt{\Gamma},\Gt{\Delta, r:S})(\wtd y')$.

  By applying \lemref{lem:varbreak} on the
   assumption of \eqref{pt:outputitr} we have:
   \begin{align}
     \label{eq:rec-outputih2}
     \Gt{\Gamma};\Gt{\Delta_z} \proves \widetilde z \hastype \Gt{C}
   \end{align}

We assume $\wtd x = \wtd x', z$. Since 
$\wtd x' \subseteq \fn{P'}$ follows that  
 $\widetilde x \subseteq \fn{P}$.
 Let $\wtd y = \wtd y', \wtd z$ where 
 $\len{\wtd z} = \len{\Gt{C}}$. 
 By \defref{def:indexed} follows that  
 $\indexed{\wtd y}{\wtd x}{\Gamma, \Delta \cat r : S \cat \Delta_z}$. 
  We define $\Theta = \Theta_1 \cat \Theta'$, where:
  \begin{align*}
    \Theta' = \prop_{k}: \btinp{\widetilde M} \tinact \cat
    \dual{\prop_{k+1}}:\btout{\widetilde M_1} \tinact
  \end{align*}

\noindent with $\widetilde M = (\Gt{\Gamma}\cat \Gt{\Delta \cat r:S \cat \Delta_z})(\widetilde y)$. By \defref{def:sizeproc}, we know $\lenHOopt{P} =\lenHOopt{P'} + 1$, so
$$
\dom{\Theta}=\{\prop_k,\ldots,\prop_{k+\lenHOopt{P}-1}\} \cup
\{\dual{\prop_{k+1}},\ldots,\dual{\prop_{k+\lenHOopt{P}-1}}\}
$$
and $\Theta$ is balanced since $\Theta(\prop_{k+1}) 
\dualof \Theta(\dual{\prop_{k+1}})$ and $\Theta_1$ is 
balanced. 

By \tabref{t:bdowncorec}, we have:
\begin{align*}
  \B{k}{\tilde y}{\bout{r}{z}P'} =
  \propinp{k}{\widetilde y}
  \bbout{r_{f(S)}}{\wtd z} \propout{k+1}{\widetilde y'}
  \inact \Par
  \B{k+1}{\tilde y'}{P'}
\end{align*}
% \noindent where $\len{\wtd z}=\len{\Gt{C}}$. 
Let $\Gamma_1 = \Gamma \setminus \widetilde x = \Gamma'_1$ 
and $\Delta \setminus \wtd x = \Delta'_1$.

We shall prove the following judgment:
\begin{align}
  \AxiomC{$\Gt{\Gamma_1}; \Gt{\Delta'_1} \cat \Theta \proves
  \B{k}{\tilde y}{\bout{r}{z}P'} \hastype \Proc$}
  \DisplayProof
\end{align}
%   \noindent where we may notice that following holds: 

%   $$\Delta'_1 = \Delta \setminus \wtd y' = (\Delta_1 \cat u_i:\btout{C}S \cat \Delta_z) \setminus \widetilde y $$

Let $\Delta_1 =\Delta \cat r : S \cat \Delta_z$.
To type the left-hand side component of
$\B{k}{\tilde y}{\bout{r}{z}P'}$
we use some auxiliary derivations:
\begin{align}
  \label{pt:rec-output3}
  \AxiomC{}
  \LeftLabel{\scriptsize Nil}
  \UnaryInfC{$\Gt{\Gamma};\es \proves \inact \hastype \Proc$}
  \LeftLabel{\scriptsize End}
  \UnaryInfC{$\Gt{\Gamma};\dual{\prop_{k+1}} : \tinact \proves \inact \hastype \Proc$}
  \AxiomC{}
  \LeftLabel{\scriptsize PolyVar}
  \UnaryInfC{$\Gt{\Gamma};\Gt{\Delta \cat r:S \setminus \Delta'_1}
        \proves \widetilde y' \hastype \widetilde M_1$}
  \LeftLabel{\scriptsize PolySend}
  \BinaryInfC{$\Gt{\Gamma};
        \dual{\prop_{k+1}}:\btout{\widetilde M_1} \tinact
          \cat \Gt{\Delta \cat r:S \setminus \Delta'_1}
        \proves \bout{\dual {\prop_{k+1}}}{\widetilde y'} 
        \hastype \Proc$}
  \DisplayProof
\end{align}

\begin{align}
  \label{pt:rec-output2}
  \AxiomC{\eqref{pt:rec-output3}}
  \AxiomC{\eqref{eq:rec-outputih2}}
%  	\LeftLabel{\scriptsize \lemref{lem:subst} with 
%  	$\subst{\tilde z_1}{\tilde z}$}
%  	\UnaryInfC{$\Gt{\Gamma};\Gt{\Delta_z \subst{\tilde z}{\tilde z_1}} \proves \widetilde z\hastype \Gt{C}$}
  \LeftLabel{\scriptsize PolySend}
  \BinaryInfC{\begin{tabular}{c}
        $\Gt{\Gamma};
        \Gt{\Delta_1 \setminus \Delta_1'}
              \cat
               \dual{\prop_{k+1}}:\btout{\widetilde M_1}\tinact
               \proves$ 
               $\bbout{r_{f(S)}}{\widetilde z}
                 \propout{k+1}{\widetilde y'} \inact \hastype \Proc$
                 \end{tabular}}
    \LeftLabel{\scriptsize End}
  \UnaryInfC{\begin{tabular}{c}
        $\Gt{\Gamma};
        \Gt{\Delta_1 \setminus \Delta'_1}
               \cat 
               \dual{\prop_{k+1}}:\btout{\widetilde M_1}\tinact \cat \prop_k:\tinact 
               \proves$ 
               $\bbout{r_{f(S)}}{\wtd z}
                 \propout{k+1}{\wtd y'} \inact \hastype \Proc$
                 \end{tabular}}
  \DisplayProof
\end{align}
% TODO continue updating proof here 
\begin{align}
\label{pt:rec-output1}
\AxiomC{\eqref{pt:rec-output2}}
\AxiomC{}
\LeftLabel{\scriptsize PolyVar}
\UnaryInfC{$\Gt{\Gamma};\Gt{\Delta_1 \setminus \Delta_1'} \proves
        \widetilde y \hastype \widetilde M$}
\LeftLabel{\scriptsize PolyRcv}
\BinaryInfC{\begin{tabular}{c}
        $\Gt{\Gamma_1}; 
               \Theta'
             \proves$ 
             $\propinp{k}{\widetilde y}
            \bbout{r_{f(S)}}{\wtd z}
              \propout{k+1}{\wtd y'} \inact
              \hastype \Proc$
              \end{tabular}}
\DisplayProof
\end{align}

We may notice that 
by \defref{def:typesdecompenv} and \defref{f:tdec} we have 
     $\Gt{\Delta_1 \setminus \Delta_1'}=\Gt{\Delta} \cat \wtd r : \Rtsopt{}{}{S} \cat 
     \Gt{\Delta_z} \setminus \Gt{\Delta_1'}$. Further, by \lemref{lem:indexcor}
     we know $\Gt{\Delta_1}(r_{f(S)}) = \trec{t}\btout{\Gt{C}}\vart{t}$.

The following tree proves this case:
\begin{align}
  \label{pt:output1}
  \AxiomC{\eqref{pt:rec-output1}}
  \AxiomC{\eqref{eq:rec-output-ih-1}}
  \UnaryInfC{$\Gt{\Gamma_1};\Gt{\Delta'_1} \cat
        \Theta_1 \proves
              \B{k+1}{\tilde y'}{P'} \hastype \Proc$}
   \LeftLabel{\scriptsize Par}
  \BinaryInfC{$\Gt{\Gamma_1}; \Gt{\Delta'_1} \cat \Theta \proves
                \B{k}{\tilde y}{\bout{r}{z}P'} \hastype \Proc$}
  \DisplayProof
\end{align}

\item Case $P = \binp{r}{z}P'$ when $\tr(r)$.
For this case Rule \textsc{Rcv} can be applied:
  \begin{align}
    \label{pt:rec-inputInv}
    \AxiomC{$\Gamma; \Delta \cat r : S'  \cat \Delta_z \proves P' \hastype \Proc$}
    \AxiomC{$\Gamma; \Delta_z \proves z \hastype C$}
    \LeftLabel{\scriptsize Rcv}
    \BinaryInfC{$\Gamma \setminus z;
            \Delta \cat r:
                  S \proves \binp{r}{z}P' \hastype \Proc$}
    \DisplayProof
  \end{align}
\noindent where $S = \btinp{C}S'$. 

Then, by IH on the first assumption of \eqref{pt:inputInv} we know:
\begin{align}
  \label{eq:rec-input-ih}
  \Gt{\Gamma'_1};\Gt{\Delta'_1} \cat \Theta_1 \proves
  \B{k+1}{\tilde y'}{P'} \hastype \Proc
\end{align}

\noindent where 
$\widetilde x' \subseteq \fn{P'}$ 
such that $r \in \wtd x'$ 
and $\widetilde y'$ such that 
$\indexed{\widetilde y'}{\widetilde x'}{\Gamma,\Delta \cat r:S}$. 
By this follows that $(r_1,\ldots,r_{\len{\Gt{S}}}) \subseteq \wtd y'$. 

Also,
 $\Gamma_1'=\Gamma \setminus \widetilde x'$, 
 $\Delta_1' = \Delta \setminus \widetilde x'$, and $\balan{\Theta_1}$ with
 $$
 \dom{\Theta_1}=\{\prop_{k+1},\ldots,\prop_{k+\lenHOopt{P'}}\}
 \cup \{\dual{\prop_{k+2}},\ldots,\dual{\prop_{k+\lenHOopt{P'}}}\}
 $$
 and ${\Theta_1(\prop_{k+1})}=\btinp{\widetilde M'}\tinact$
 where $\widetilde M' = (\Gt{\Gamma},\Gt{\Delta,r:S,\Delta_z})(\widetilde y')$.

By applying \lemref{lem:varbreak} to the second
assumption of \eqref{pt:inputInv} we have:
\begin{align}
  \label{eq:rec-input-ih2}
  \Gt{\Gamma};\Gt{\Delta_z} \proves z \hastype \Gt{C}
\end{align}

Let $\wtd x = \wtd x' \setminus z$ 
and $\wtd y = \wtd y' \setminus \wtd z$ such that 
$\len{\wtd z}=\Gt{C}$ where. We may notice that 
by \defref{def:indexed} 
 $\indexed{\wtd y}{\wtd x}{\Gamma,\Delta \cat r:S}$ holds. 
We define $\Theta = \Theta_1 \cat \Theta'$, where
\begin{align*}
\Theta' = \prop_k:\btinp{\widetilde M} \tinact \cat \dual {\prop_{k+1}}:\btout{\widetilde M'} \tinact
\end{align*}
with $\widetilde M = (\Gt{\Gamma},\Gt{\Delta \cat \cat u_i:
                  \btinp{C}S})(\widetilde y)$.
By \defref{def:sizeproc},
$\lenHOopt{P} = \lenHOopt{P'} + 1$ so
$$\dom{\Theta} = \{\prop_k,\ldots,\prop_{k+\lenHOopt{P}-1}\}
  \cup \{\dual{\prop_{k+1}},\ldots,\dual{\prop_{k+\lenHOopt{P}-1}}\}$$
  and $\Theta$ is balanced since $\Theta(\prop_{k+1}) \dualof \Theta(\dual{\prop_{k+1}})$ and
   $\Theta_1$ is balanced.
By \tabref{t:bdowncorec}:
\begin{align*}
 \B{k}{\tilde y}{\binp{r}{z}P'} = \propinp{k}{\wtd y}
 \binp{r_{f(S)}}{\wtd z}
 \propout{k+1}
 {\wtd y'} \inact \Par \B{k+1}{\tilde y'}{P'}
\end{align*}

Also, let $\Gamma_1 = \Gamma \setminus \widetilde x$ and 
$\Delta_1 = \Delta \setminus \widetilde x$. We may notice that 
$\Delta_1 = \Delta'_1$.
We shall prove the following judgment:
\begin{align*}
\Gt{\Gamma_1 \setminus z};\Gt{\Delta_1}
  \cat \Theta
  \proves
    \B{k}{\tilde y}{\binp{r}{z}P'}
\end{align*}

%\noindent where $\Gamma_1 = \Gamma \setminus \widetilde x$.
Let $\Delta_1 = \Delta \cat r:S$.
The left-hand side component of $\B{k}{\tilde y}{\binp{r}{z}P'}$ is typed using
 some auxiliary derivations:
\begin{align}
  %\gamma
  \label{pt:rec-input3}
  \AxiomC{}
  \LeftLabel{\scriptsize Nil}
  \UnaryInfC{$\Gt{\Gamma};\es \proves \inact \hastype \Proc$}
  \LeftLabel{\scriptsize End}
  \UnaryInfC{$\Gt{\Gamma};\dual{\prop_{k+1}}:\tinact \proves \inact \hastype \Proc$}
  \AxiomC{}
  \LeftLabel{\scriptsize PolyVar}
  \UnaryInfC{$\Gt{\Gamma};
  \Gt{\Delta \setminus \Delta_1}
              \proves \widetilde y' \hastype \widetilde M'$}
  \LeftLabel{\scriptsize PolySend}
  \BinaryInfC{$\Gt{\Gamma};
                \dual {\prop_{k+1}}:\btout{\widetilde M'} \tinact
                \cat 
                \Gt{\Delta \setminus \Delta_1}
                \proves \propout{k+1}{\widetilde y'} \inact \hastype \Proc$}
  \DisplayProof
\end{align}
\begin{align}
  %beta
  \label{pt:rec-input2}
  \AxiomC{\eqref{pt:rec-input3}}
  \AxiomC{\eqref{eq:rec-input-ih2}}
  \LeftLabel{\scriptsize Rcv}
  \BinaryInfC{
  \begin{tabular}{c}
      $\Gt{\Gamma \setminus z}; 
              \dual {\prop_{k+1}}:\btout{\widetilde M'} \tinact \cat 
      \Gt{\Delta_2}
              \proves$ 
              $\binp{r_{f(S)}}{\widetilde z}\propout{k+1}{\widetilde y'} \inact \hastype \Proc$
  \end{tabular}
}
   \LeftLabel{\scriptsize End}
  \UnaryInfC{ 
  \begin{tabular}{c}
  $\Gt{\Gamma \setminus z}; 
              \dual {\prop_{k+1}}:\btout{\widetilde M'} \tinact
              \cat \prop_k: \tinact \cat
              \Gt{\Delta_2}
              \proves$ 
              $\binp{r_{f(S)}}{\wtd z}\propout{k+1}{\widetilde y'} \inact \hastype \Proc$
   \end{tabular}}
  \DisplayProof
\end{align}

\begin{align}
  \label{pt:rec-input1}
  \AxiomC{\eqref{pt:rec-input2}}
  \AxiomC{}
  \LeftLabel{\scriptsize PolyVar}
  \UnaryInfC{$\Gt{\Gamma \setminus z};
  \Gt{\Delta_2}
  \proves \widetilde y \hastype \widetilde M$}
  \LeftLabel{\scriptsize PolyRcv}
  \BinaryInfC{$\Gt{\Gamma_1 \setminus z};
   \Theta' \proves \propinp{k}{\widetilde
  y}\binp{r_{f(S)}}{z}\propout{k+1}{\widetilde y'} \inact \hastype \Proc$}
\DisplayProof
\end{align}
\noindent 
where $\Delta_2 = \Delta \cat r:S \setminus \Delta_1$. 
We may notice that 
by \defref{def:typesdecompenv} and \defref{f:tdec} we have 
     $\Gt{\Delta_2}=\Gt{\Delta} \cat \wtd r : \Rtsopt{}{}{S} \setminus  
     \Gt{\Delta_1}$. Further, by \lemref{lem:indexcor}
     we know $\Gt{\Delta_2}(r_{f(S)}) = \trec{t}\btinp{\Gt{C}}\vart{t}$.

The following tree
proves this case:
\begin{align}
  \label{pt:rec-input}
  \AxiomC{\eqref{pt:rec-input1}}
  \AxiomC{\eqref{eq:rec-input-ih}}
   \LeftLabel{\scriptsize}
  \UnaryInfC{
  \begin{tabular}{c}
  $\Gt{\Gamma'_1 \setminus z}; \Gt{\Delta_1} \cat \Theta_1 \proves$ 
  $\B{k+1}{\tilde y'}{P'} \hastype \Proc$
  \end{tabular}}
  \LeftLabel{\scriptsize Par}
  \BinaryInfC{\begin{tabular}{c}
        $\Gt{\Gamma_1 \backslash z};\Gt{\Delta_1}
                \cat \Theta \proves$ 
                $\propinp{k}{\widetilde y}
                \binp{r_{f(S)}}{\widetilde z}\propout{k+1}{\widetilde y'} \inact \Par \B{k+1}
                {\tilde y'}{P'} \hastype \Proc$
                \end{tabular}}
  \DisplayProof
\end{align}
  \noindent

\item Case $P = \news{s:\trec{t}{S}}{P'}$. For this case 
Rule~\textsc{ResS} can be applied: 
\begin{align}
\label{pt:resrecInv}
\AxiomC{$\Gamma;\Delta \cat s:\trec{t}S \cat 
\dual{s}:\dual{\trec{t}S} \proves P'$} 
\LeftLabel{\scriptsize ResS}
\UnaryInfC{$\Gamma;\Delta \proves 
\news{s:\trec{t}{S}}P'$}
\DisplayProof
\end{align}

By IH on the assumption of \eqref{pt:resrecInv} we have: 
\begin{align}
\label{eq:recresIh}
\Gt{\Gamma \setminus \wtd x'};\Gt{\Delta \setminus \wtd x'}
\cat \Theta_1 \proves \B{k+1}{\tilde y'}{P'}	
\end{align}

where we take $\wtd y'$ such that $\wtd s, \wtd {\dual s} \subseteq \wtd y'$ with $\wtd s = (s_1,\ldots,s_{\len{\Rtopt{S}}})$
and $\wtd {\dual s} = (\dual s_1,\ldots,\dual s_{\len{\Rtopt{S}}})$.
. Accordingly, $\wtd x'$ is such that
$s,\dual s \subseteq \wtd x'$. Since $\mathtt{lin}(s)$ and 
$\mathtt{lin}(\dual s)$ we know $\wtd x' \subseteq \fn{P'}$.  
Also, $\indexed{\wtd y'}{\wtd x'}{\Gamma,\Delta_1}$ 
where $\Delta_1 = \Delta \cat s:\trec{t}S \cat 
\dual{s}:\dual{\trec{t}S} $. 
Also, $\balan{\Theta_1}$ with 
 $$
 \dom{\Theta_1}=\{\prop_{k+1},\ldots,\prop_{k+\lenHOopt{P'}}\}
 \cup \{\dual{\prop_{k+2}},\ldots,\dual{\prop_{k+\lenHOopt{P'}}}\}
 $$
 \noindent and $\Theta_1(\prop_{k+1}) = \btinp{\wtd M'}\tinact$
 where $\wtd M = (\Gt{\Gamma}, \Gt{\Delta})(\wtd y')$. 
 
 Let $\wtd y = \wtd y' \setminus (\wtd s, \wtd {\dual s})$ 
 and $\wtd x = \wtd x' \setminus (s,\dual s)$. 
 Since $s,\dual s \notin \fn{P}$ we know $\wtd x \subseteq \fn{P}$
 and $\indexed{\wtd y}{\wtd x}{\Gamma,\Delta}$.
 
 We define $\Theta = \Theta_1\cat \Theta'$ where 
 $$\Theta' = \prop_k:\btinp{\wtd M}\tinact \cat 
 \dual{\prop_{k+1}} : \btout{\wtd M'}\tinact$$
 
 By \tabref{t:bdowncorec}, we have: 
 \begin{align*}
   \B{k}{\tilde y}{P} = \news{\widetilde{s}:\Rtopt{S}}
   (\propinp{k}{\wtd y}\propout{k+1}{\wtd y'}\inact \Par \B{k}{\tilde y'}{P'})
 \end{align*}
 
 We should prove the following judgment: 
 \begin{align*}
   \Gt{\Gamma \setminus \wtd x};\Gt{\Delta \setminus \wtd x} \cat \Theta \proves \B{k}{\tilde y}{P} \hastype \Proc
 \end{align*}

We use some auxiliary sub-tree: 

\begin{align}
  \label{pt:resrec1}
  \AxiomC{} 
  \LeftLabel{\scriptsize Nil}
  \UnaryInfC{$\Gt{\Gamma};\es \proves \inact 
  \hastype \Proc$} 
  \AxiomC{} 
  \LeftLabel{\scriptsize PolyVar}
  \UnaryInfC{$\Gt{\Gamma};\Gt{\Delta_1 \cap \wtd x'} \proves 
  \wtd y' \hastype \wtd M'$} 
  \LeftLabel{\scriptsize PolySend}
  \BinaryInfC{$\Gt{\Gamma};\Gt{\Delta \cap \wtd x}
\cat 
\wtd s : \Rtopt{S} \cat \wtd {\dual s}: \Rtopt{\dual S}
\proves \propout{k+1}{\wtd y'}\inact
\hastype \Proc$}
  \DisplayProof
\end{align}
\noindent here we may notice that 
$$\Gt{\Delta \cap \wtd x}
\cat 
\wtd s : \Rtopt{S} \cat \wtd {\dual s}: \Rtopt{\dual S} = 
\Gt{\Delta_1 \cap \wtd x'}$$

The following tree proves this case: 
\begin{align}
\AxiomC{\eqref{pt:resrec1}} 
\AxiomC{} 
\LeftLabel{\scriptsize PolyVar}
\UnaryInfC{$\Gt{\Gamma};\Gt{\Delta \cap \wtd x} \proves \wtd y \hastype \wtd M$} 
\LeftLabel{\scriptsize PolyRcv}
\BinaryInfC{$\Gt{\Gamma \setminus \wtd x};
\Theta' \cat 
  \wtd s : \Rtopt{S} \cat \wtd {\dual s}: \Rtopt{\dual S}
  \proves 
  \propinp{k}{\wtd y}\propout{k+1}{\wtd y'}\inact
  \hastype \Proc$} 
\AxiomC{\eqref{eq:recresIh}} 
\LeftLabel{\scriptsize Par}
  \BinaryInfC{$\Gt{\Gamma \setminus \wtd x};\Gt{\Delta \setminus \wtd x} \cat \Theta \cat 
  \wtd s : \Rtopt{S} \cat \wtd {\dual s}: \Rtopt{\dual S}
  \proves 
   \propinp{k}{\wtd y}\propout{k+1}{\wtd y'}\inact \Par \B{k}{\tilde y'}{P'} \hastype \Proc$} 
  \LeftLabel{\scriptsize PolyResS}
  \UnaryInfC{$	\Gt{\Gamma \setminus \wtd x};\Gt{\Delta \setminus \wtd x} \cat \Theta \proves 
  \news{\widetilde{s}:\Rtopt{S}}
   (\propinp{k}{\wtd y}\propout{k+1}{\wtd y'}\inact \Par \B{k}{\tilde y'}{P'})
  \hastype \Proc$}
  \DisplayProof
\end{align}
 
\end{enumerate}

\qed

\end{proof}

\subsection{Proof of \thmref{t:decompcore} (Minimality Result, Optimized)}
\label{app:decompcore}
\thmdecompcore*

\begin{proof} 

  By assumption, $\Gamma;\Delta \proves P \hastype \Proc$. 
  Then by applying \lemref{lem:subst} we have: 
  \begin{align}
  \label{eq:rec-typedec-subst}
    \Gamma\sigma;\Delta\sigma \proves P\sigma \hastype \Proc	
  \end{align}
  
  By \defref{def:decomp}, we
    shall prove the following judgment:
    \begin{align} 
    \Gt{\Gamma\sigma};\Gt{\Delta\sigma} \proves 	
    \news{\wtd \prop}(
    \propout{k}{\wtd r} \inact \Par \B{k}{\tilde r}{P\sigma})
    \hastype \Proc 
    \end{align}
  \noindent where $\widetilde \prop = (\prop_k,\ldots,\prop_{k+\lenHOopt{P}-1})$;
     $k > 0$; and 
    $\wtd r = \bigcup_{v \in \tilde v}\{v_1,\ldots, v_{\len{\Gt{S}}} \}$ with $v:S$.
    Since $\wtd v \subseteq \fn{P}$ 
    we know $\indexed{\wtd r}{\wtd v}{\Gamma\sigma, \Delta\sigma}$.
    Since $P\sigma$ is an initialized process, 
  we apply \thmref{t:typerecur} to \eqref{eq:rec-typedec-subst} to get:
    \begin{align}
      \label{eq:rec-typedec-bdown}
      \Gt{\Gamma\sigma};\Gt{\Delta \sigma \setminus \wtd v}\cat\Theta
      \proves \B{k}{\tilde r}{P\sigma} \hastype \Proc
    \end{align}
  \noindent where	$\Theta$ is balanced with
    $\dom{\Theta} = \{\prop_k,\prop_{k+1},\ldots,\prop_{k+\lenHOopt{P}-1} \}
    \cup \{\dual{\prop_{k+1}},\ldots,\dual{\prop_{k+\lenHOopt{P}-1}} \}$ and
    $\Theta(\prop_k)=\btinp{\wtd M}\tinact$ 
    with $\wtd M =\Gt{\Delta}(\wtd r)$.
    
    The following tree proves this case: 
    \begin{align*}
    \AxiomC{} 
    \LeftLabel{\scriptsize Nil}
    \UnaryInfC{$\Gt{\Gamma\sigma};\emptyset \proves \inact
    \hastype \Proc$} 
    \LeftLabel{\scriptsize End}
    \UnaryInfC{$\Gt{\Gamma\sigma};\prop_k:\tinact \proves \inact
    \hastype \Proc$} 
    \AxiomC{}
    \LeftLabel{\scriptsize PolyVar} 
    \UnaryInfC{$\Gt{\Gamma\sigma}; 
    \wtd r:\wtd M \proves \wtd r \hastype \wtd M$} 
    \LeftLabel{\scriptsize Send}
    \BinaryInfC{$\Gt{\Gamma\sigma};
      \dual{\prop_k}:\btout{\wtd M}\tinact 
      \cat \wtd r : \wtd M
      \proves 	
    \propout{k}{\wtd r} \inact   \hastype \Proc$} 
    \AxiomC{\eqref{eq:rec-typedec-bdown}} 
    \LeftLabel{\scriptsize Par}
      \BinaryInfC{$\Gt{\Gamma\sigma};\Gt{\Delta\sigma} 
      \cat \dual{\prop_k}:\btout{\wtd M}\tinact \cat \Theta
      \proves 	
    \propout{k}{\wtd r} \inact \Par \B{k}{\tilde r}{P\sigma}
    \hastype \Proc$}
      \LeftLabel{\scriptsize ResS}
      \UnaryInfC{$\Gt{\Gamma\sigma};
      \Gt{\Delta\sigma} \proves 	
    \news{\wtd \prop}(
    \propout{k}{\wtd r} \inact \Par \B{k}{\tilde r}{P\sigma})
    \hastype \Proc$}
    \DisplayProof
    \end{align*}
  \end{proof}

\subsection{MST Bisimilarity}
 \label{app:ss:mst}

% \begin{definition}[Indexed name]
%   \label{def:indexedname}
%   Given a name $n$, we write $\iname{n}$ to either denote 
%   $n$ or any indexed name $n_i$, with $i > 0$.
% \end{definition}

% \begin{definition}[Relating names]
%   \label{def:namesrelate}
%   We define $\valuesrelate$ as the relation on names defined as
%   $$
%   \frac{}
%   {\epsilon \valuesrelate \epsilon} 
%   \quad 
%   \frac{\Gamma;\Delta \proves n_i \hastype C}
%   {n_i \valuesrelate (n_i,\ldots,n_{i+\len{\Gt{C}}-1})} 
%   \quad 
%    \frac{\tilde n \valuesrelate \tilde m_1 \ 
%   \quad  n_i \valuesrelate \tilde m_2}
%   {\tilde n,n_i \valuesrelate \tilde m_1, \tilde m_2} 
%   $$
%   \noindent where $\epsilon$ denotes the empty list. 
% \end{definition}

%
%\begin{definition}[Indexed names substitutions]
%  \label{d:indexedsubstitution}
%  Let 
%  $$\widetilde u = (a,b,s, \dual s, \dual{s}', s',r, r', \ldots)$$ 
%  be a finite tuple of names.
%  We write $\indices{\wtd u}$ to denote 
%  $$\indices{\wtd u} = 
%  \{\subst{a_{1}, b_{1}, s_{i}, \dual s_{i},  
%  s'_{j}, \dual s'_{j}, r_{1}, r'_{1}, \ldots}{a,b,s,s',r,r',\ldots} : 
%  i,j,\ldots > 0 \}$$
%\end{definition}

\noindent Now, we are ready to relate processes, modulo indexed names
(Def.~\ref{def:indexedname}), using the relation $\processrelate$ defined as follows: 
\begin{definition}[$\processrelate$ Indexed process relation]
We define the relation $\processrelate$ as
  \label{def:valuesprelation}
  \begin{mathpar}
    \inferrule[\eltsrule{IPSnd}]
    {P\sigma \processrelate P' \and v\sigma \valuesrelate \wtd v \and \sigma = \nextn{n_i}}
    {\bout{n_i}{v}P \processrelate \bout{n_i}{\wtd v}P'}
    \qquad 
    \inferrule[\eltsrule{IPInact}] {
    }{\inact \processrelate \inact} 
    \\
    \inferrule[\eltsrule{IPRcv}] {
      P\sigma \processrelate P' \and v\sigma \valuesrelate \wtd v \and \sigma = \nextn{n_i}
    }{\binp{n_i}{y}P \processrelate \binp{n_i}{\wtd y}P'}  
   \quad 
    \inferrule[\eltsrule{IPNews}] 
    { P \processrelate P' \and \tilde m_1 \valuesrelate \tilde m_2 
    }{\news{\tilde m_1}P \processrelate \news{\tilde m_2}P' } 
  \end{mathpar}
\end{definition}

\begin{definition}[Minimal characteristic processes]
  \label{d:mcp}
    \begin{align*}
      \mapcharm{\btinp{C} S}{u}_i
      &\defeq
      \binp{u_i}{x} (\bout{t}{u_{i+1}, \ldots,u_{i+\len{\Gt{S}}}} \inact \Par \mapcharm{C}{x}_i)
      \\
      \mapcharm{\btout{C} S}{u}_i
      &\defeq
      \bout{u_i}{\omapcharm{C}} \bout{t}{u_{i+1}, \ldots,u_{i+\len{\Gt{S}}}} \inact \\
      \mapcharm{\tinact}{u}_i & \defeq \inact \\
      \mapcharm{\chtype{C}}{u}_i
      &\defeq \bout{u_1}{\omapcharm{C}} \bout{t}{u_1} \inact \\
      \mapcharm{ \trec{t}{S} }{u}_i &\defeq \mapcharm{S \subst{\tinact}{\vart{t}} }{u}_i \\
      \omapcharm{S}  & \defeq   \wtd s ~~ (\len{\wtd s} = \len{\Gt{S}}, \wtd s \textrm{ fresh}) \\
      \omapcharm{\chtype{C}} &\defeq a_1 ~~ (a_1 \textrm{ fresh})
    \end{align*}
\end{definition}

% \begin{definition}[Characteristic trigger process]
%   \begin{align*}
%     \ftrigger{t}{v}{C}	& \defeq 	\fotrigger{t}{x}{s}{C}{v}
%   \end{align*}
% \end{definition}

% \begin{definition}[Minimal characteristic trigger process]
%   \begin{align*}
%     \ftriggerm{t}{v_i}{C}	& \defeq 	\fotriggerm{t_1}{x}{s_1}{C}{v_i}{i}
%   \end{align*}
% \end{definition}

\begin{definition}[Trigger Collections]
  \label{d:triggerscollection}
  We let $H, H'$ to range over \emph{trigger collections}: processes of the form
  $P_1 \Par \cdots \Par P_n$ (with $n \geq 1$), where each $P_i$ is a trigger
  process or a process that originates from a trigger process. 
 \end{definition}
 
 \begin{example}
  Let $H_1 =  \ftrigger{t}{v}{C} \Par \mapchar{C}{u_1} \Par 
  \bout{t_2}{u_2}\inact$  
  where $v, t_1,t_2,u_1,u_2$ are channel names, 
  $C$ a channel type. We could see that, 
  $\mapchar{C}{u_1}$ and  $\bout{t_2}{u_2}\inact$ 
  originates from a trigger process. Thus, $H_1$ is a trigger collection.
 \end{example}

\begin{definition}[Process in parallel with a trigger or a characteristic process]
  \label{def:parallel}
We write 
  $P \parallel Q$ to stand for $P \Par Q$ 
  where either $P$ or $Q$ is a trigger collection. \end{definition}

  \begin{definition}[Propagators of $P$]
   \label{d:fpn}
    We define $\fpn{P}$ to denote the set of free propagator names in $P$. 
  \end{definition}

  \begin{definition}[Depth of recursive variable]
    Let $P$ be a recursive process. 
    We define \rvardepth{P} to count sequential prefixes in $P$ 
    preceding recursive variable $X$ or a subprocess of shape $\recp{X}Q$. 
    Function \rvardepth{P} and \rvardepthaux{P} are mutually defined as follows: 
    \begin{align*}
      \rvardepth{P} &= 
      \begin{cases}
        \rvardepthaux{P} & \text{ if } \recpx{P} \\
          0 & \text{ otherwise } \\
      \end{cases}
      \\ 
      \rvardepthaux{P} &= 
      \begin{cases}
        \rvardepth{Q} + 1 & \text{ if } P = \alpha.Q \\
        \rvardepth{Q} + \rvardepth{R}  & \text{ if } P = Q \Par R \\
        0 & \text{ if } P = \recp{X}Q \text{ or } P = \rvar{X} 
        \\
        \rvardepth{Q} & \text{ if } P = \news{s}Q
      \end{cases}
      % \rvardepthaux{\alpha.Q} &= \rvardepth{Q} + 1\\ 
      % \rvardepthaux{(Q \Par R)} &= \rvardepth{Q} + \rvardepth{R} \\
      % \rvardepthaux{\recp{X}Q} &= 0 \\ 
      % \rvardepthaux{\rvar{X}} &= 0 \\
      % \rvardepthaux{\news{s}Q} & = \rvardepth{Q}
    \end{align*}
  \end{definition}

\begin{definition}[Name breakdown]
  \label{d:name-breakdown}
  Let $u_i:C$ be an indexed name with its session type. 
  We write $\bname{u_i:C}$ to denote 
  $$\bname{u_i:C}=(u_i,\ldots,u_{i + \len{\Gt{C}} - 1})$$
\end{definition}

\noindent Function $\bname{\cdot}$ is extended to work on a list 
element-wise, as follows: 
$$\bname{(u^1_i, \ldots, u^n_j) : (C_1, \ldots, C_n)} =
\bname{u^1_i:C_1} \cdot \ldots \cdot \bname{u^n_j:C_n}$$

% \begin{figure*}
% \begin{table}[H]
%   \begin{tabular}{ |l|l|l|}
%     \rowcolor{gray!25}
%     f & f & f
%   \end{tabular} 
% \end{table} 
% \end{figure*}

% \begin{figure*}
% \begin{table}[H]
%   \begin{tabular}{ |l|l|l|}
%     \rowcolor{gray!25}
%   \hline
%   $P$ &
%   \multicolumn{2}{l|}{
%   \begin{tabular}{l}
%   \noalign{\smallskip}
%   $\Cbpi{\tilde u}{\tilde x}{P}$
%   \smallskip
%   \end{tabular} 
%   } \\
%   f & f & f 
% \end{tabular}  
% \end{table} 
% \end{figure*}

\begin{figure*}

  \begin{table}[H]
    \begin{tabular}{ |l|l|l|}
      \rowcolor{gray!25}
  \hline
  $P$ &
    \multicolumn{2}{l|}{
  \begin{tabular}{l}
    \noalign{\smallskip}
    $\Cbpi{\tilde u}{\tilde x}{P}$
    \smallskip
  \end{tabular} 
  } 
  \\
  \hline
$Q_1 \parallel Q_2$ 
&
  \begin{tabular}{l}
  \noalign{\smallskip}
     $\{ R_1 \parallel R_2: 
     R_1 \in \Cbpi{\tilde u_1}{\tilde y}{Q_1}, 
     R_2 \in \Cbpi{\tilde u_2}{\tilde z}{Q_2}
     \}$
     \smallskip 
  \end{tabular}
  &
  %side-conditions
  \begin{tabular}{l}
    \noalign{\smallskip}
    $\wtd y = \fnb{Q_1}{\tilde x}$, $\wtd z = \fnb{Q_2}{\tilde x}$ \\
    $\subst{\tilde u}{\tilde x} = \subst{\tilde u_1}{\tilde y} \cdot \subst{\tilde u_2}{\tilde z}$ 
    \smallskip
  \end{tabular}
     \\
     \hline
     $\news{s:C}{Q}$ &
     \begin{tabular}{l}
       \noalign{\smallskip}
        $\{\news{\widetilde{s}:\Gt{C}}{\,R} : \Cbpi{\tilde u}{\tilde x}{Q\sigma} \}$
       \smallskip
     \end{tabular}
     &
     %side-conditions
     \begin{tabular}{l}
       \noalign{\smallskip}
       $\widetilde{s} = (s_1,\ldots,s_{\len{\Gt{C}}})$ \\
       $\sigma =  \subst{s_1 \dual{s_1}}{s \dual{s}}$
      %  $\sigma = \begin{cases}
      %              \subst{s_1 \dual{s_1}}{s \dual{s}} & \text{if} \ C = S \\
      %              \subst{s_1}{s} & \text{if} \ C = \chtype{U}
  %  \end{cases}
  %  $
       \smallskip
     \end{tabular}
     \\
     \hline
  $Q$
  &
  \begin{tabular}{l}
  \noalign{\smallskip}
     $\{  \news{\wtd \prop} R \,:\,  
  R = \apropout{k}{\wtd u} \Par \B{k}{\tilde x}{Q} \}$ 
   \\
  $\cup~ \{ \news{\wtd \prop}R \,:\, R \in \Dbpi{\tilde u}{\tilde x}{Q}\}$
  \smallskip 
  \end{tabular}
  &
  %side-conditions
  \begin{tabular}{l}
    \noalign{\smallskip}
    $\wtd \prop = \fpn{R}$
    \smallskip
  \end{tabular} 
  \\
  \hline 
    $\inact$ &
  \begin{tabular}{l}
    \noalign{\smallskip}
    $\{\inact\}$
   \smallskip
  \end{tabular}
  &
  \begin{tabular}{l}
      \noalign{\smallskip}
  %$\widetilde x = \es$ 
  \smallskip
  \end{tabular}
%   \\
%   \hline 
%   $\Cbrecpi{\tilde u}{\tilde x}{Q}$
% &
%   \begin{tabular}{l}
%   \noalign{\smallskip}
%   $\{  \news{\wtd \prop} (\propoutrec{k+1}{\wtd z\rho}
%   \recp{X}\binp{\prop^r_{X}}{\wtd y}
% \propoutrec{k+1}{\wtd y}X \Par R) \,:\,  
%   R = \Brec{k}{\tilde x}{Q}_g \}$ 
%   \\
%   $\cup~ \{  \news{\wtd \prop} (
%   \recp{X}\binp{\prop^r_{X}}{\wtd y}
% \propoutrec{k+1}{\wtd y}X \Par R 
% \Par 
% \proproutk{r}{\rvar{X}}{\wtd x\rho}
% \recp{X}\proprinpk{r}{k}{\wtd x}\proproutk{r}{\rvar{X}}{\wtd x}\rvar{X}
% )  \,:\, R = \Brec{k}{\tilde x}{Q\subst{\specx}{X}}_g \}$ \\ 
%   $\cup \ \{\news{\wtd \prop} R : R \in \Dbrecpi{\tilde u}{\tilde x}{Q} \}$
%      \smallskip 
%   \end{tabular}
%   &
%   %side-conditions
%   \begin{tabular}{l}
%     \noalign{\smallskip}
%     \smallskip
%   \end{tabular}
  \\ 
      \rowcolor{gray!25}
      \hline
      $P$ &
        \multicolumn{2}{l|}{
      \begin{tabular}{l}
        \noalign{\smallskip}
        $\Dbpi{\tilde u}{\tilde x}{P}$
        \smallskip
      \end{tabular}
    }  \\
      \hline
    $\binp{n_i}{y}Q$
    &
    
      \begin{tabular}{l}
          \noalign{\smallskip}
          $\{\binp{n_{\mstindex} \rho}{\wtd y} 
          \apropout{k+1}{\wtd z \rho}
         \Par \B{k+1}{\tilde z}{Q\sigma}\}$ \\
          \smallskip
      \end{tabular}
      &
      %side-conditions
      \begin{tabular}{l}
        \noalign{\smallskip}
        $y:S$ $\wedge$ $\wtd y = (y_1,\ldots,y_{\len{S}})$ \\
        $\wtd w = \linecondit{\lin{n_i}}{\{n_i\}}{\epsilon}$ \\
    %     $\wtd w = \begin{cases}
    %  \{ n_i \} & \text{if} \ \lin{n_i} \\
    %  \epsilon & \text{otherwise} 	
    %  \end{cases}
    % $ \\ 
        $\wtd z = \fnb{Q}{\wtd x \wtd y \setminus \wtd w}$\\
        $\rho = \subst{\tilde u}{\tilde x}$ \\
        % $\rho= \rho
        % \cdot \subst{\tilde u_z}{\tilde z}$ \\
        $\sigma = \nextn{n_i}\cdot \subst{y_1}{y}$  \\
        $\mstindex = \linecondit{\tr(S)}{f(S)}{i}$
        \smallskip
      \end{tabular}
        \\
      \hline
      
      $\bout{n_i}{y_j}{Q}$ &
        \begin{tabular}{l}
          \noalign{\smallskip}
                $\{\bbout{n_{\mstindex} \rho}
                {\wtd y \rho}         
                \apropout{k+1}{\wtd z \rho}  \Par$ 
          $\B{k+1}{\tilde z}{Q\sigma} \}$
         \smallskip
      \end{tabular}
      &
      %side-conditions
      \begin{tabular}{l}
        \noalign{\smallskip}
        $y : S \wedge \wtd y = (y_j, \ldots,y_{j+\len{\Gt{S}}-1})$ \\
        $\wtd w = \linecondit{\lin{n_i}}{\{n_i\}}{\epsilon}$ \\
    % $\wtd w = \begin{cases}
    %  \{ n_i \} & \text{if} \ \lin{n_i} \\
    %  \epsilon & \text{otherwise} 	
    %  \end{cases}
    % $ \\ 
         $\wtd z = \fnb{Q}{\wtd x \setminus \wtd w}$\\
         $\rho = \subst{\tilde u}{\tilde x}$ \\
          % $\rho= \rho
          % \cdot \subst{\tilde u_z}{\tilde z}$ \\
         $\sigma = \nextn{n_i}$ \\
         ${\mstindex} = \linecondit{\tr(S)}{f(S)}{i}$
        \smallskip
      \end{tabular}
      \\
    
    \hline

      $Q_1 \Par Q_2$ &
      \begin{tabular}{l}
        \noalign{\smallskip}
        $\{ \propout{k}{\wtd y \rho}
        \apropout{k+\degree}{\wtd z \rho}   \Par$ 
        $\B{k}{\tilde y}{Q_1} \Par \B{k+\degree}{\tilde z}{Q_2}\}$ \\
        $\cup$
        \\
        $\{(R_1 \Par R_2) :
        \Cbpi{\tilde u_1}{\tilde y}{Q_1}, R_2 \in 
        \Cbpi{\tilde u_2}{\tilde z}{Q_2}\}$
        \smallskip
      \end{tabular}
      &
      %side-conditions
      \begin{tabular}{l}
        \noalign{\smallskip}
        $\wtd y  = \fnb{Q_1}{\wtd x}$ \\
        $\wtd z = \fnb{Q_2}{\wtd x}$ \\
        $\rho = \subst{\tilde u}{\tilde x}$ \\
      %  $\subst{\tilde u}{\tilde x} = \subst{\tilde u_1}{\tilde y}
      %  \cdot \subst{\tilde u_2}{\tilde z}$ \\
        $\degree = \lenHOopt{Q_1}$
        \smallskip
      \end{tabular}
          \\
      \hline
      $\recp{X}P$ &
    \begin{tabular}{l}
      \noalign{\smallskip}
      $\{ \propoutrec{k+1}{\wtd z\rho}
              \recp{X}\binp{\prop^r_{X}}{\wtd y}
        \propoutrec{k+1}{\wtd y}X
            \Par$  \\
            $\Brec{k+1}{\tilde x}{P}_{g}\}$
     \smallskip
    \end{tabular}
    &
    \begin{tabular}{l}
        \noalign{\smallskip}
        $\wtd n = \fn{P}$ \\
        $\wtd n : \wtd C$ $\wedge$ $\wtd m = \bname{\wtd n : \wtd C}$ \\
        $\wtd z = \wtd x \cup \wtd m$, $\len{\wtd z} = \len{\wtd y}$ \\
        $g = \{X \mapsto \wtd m\}$
    \smallskip
    \end{tabular}
    \\
    \hline 
      $\inact$ &
    \begin{tabular}{l}
      \noalign{\smallskip}
      $\{\inact\}$
     \smallskip
    \end{tabular}
    &
    \begin{tabular}{l}
        \noalign{\smallskip}
    %$\widetilde x = \es$ 
    \smallskip
    \end{tabular}
      \\
      \hline 
    \end{tabular}
    \caption{The definition of $\Cbpi{\tilde u}{\tilde x}{P}$ 
    and $\Dbpi{\tilde u}{\tilde x}{P}$
    (core fragment). \label{t:tablecd}}
    \vspace{-2mm}
    \end{table}
\end{figure*}

\begin{figure*}

  \begin{table}[H]
    \begin{tabular}{ |l|l|l|}
      \rowcolor{gray!25}
  \hline
  $P$ &
    \multicolumn{2}{l|}{
  \begin{tabular}{l}
    \noalign{\smallskip}
    $\Cbpi{\tilde u}{\tilde x}{P}$
    \smallskip
  \end{tabular} 
  } 
\\
     \hline
  $Q$
  &
  \begin{tabular}{l}
  \noalign{\smallskip}
  % $f$ \\
  $\Cbrecpi{\tilde u}{\tilde x}{\recp{X}Q^*}^d$
  $\text{ if } Q \equiv \alpha_d.\alpha_{d-1}. \ldots .\alpha_{d-p}.(P_X \Par R)$
  and $\recp{X}Q^*$ is a subprocess of $P_X$
  \smallskip 
  \\
  \hdashline 
  \noalign{\smallskip}
    % $\{  \news{\wtd \prop} R \,:\,  
    % R = \apropout{k}{\wtd u} \Par \B{k}{\tilde x}{Q} \}$ 
    $\{  \news{\wtd \prop} R \,:\,  
    R \in \{\apropout{k}{\wtd u} \Par \B{k}{\tilde x}{Q}, 
    \apropoutrecsh{k}{\wtd u}{} \Par \Brec{k}{\tilde x}{Q} \} \}$
    \\
    $\cup~ \{ \news{\wtd \prop}R \,:\, R \in 
    \Dbpi{\tilde u}{\tilde x}{Q} \cup \Dbrecpi{k}{\tilde x, \rho}{Q}^d_\es\}$ 
    $\text{ otherwise }$
  \smallskip
  \end{tabular}
  &
  %side-conditions
  \begin{tabular}{l}
    \noalign{\smallskip}
    $\wtd \prop = \fpn{R}$ \\
    $\rho = \subst{\tilde u}{\tilde x}$
    \smallskip
  \end{tabular} 
  \\
  \hline 
  $\Cbrecpi{\tilde u}{\tilde x}{Q}^d$
  % $\recp{X}Q$
&
  \begin{tabular}{l}
  \noalign{\smallskip}
  $ \{\news{\wtd \prop} (
    \recp{X}\binp{\prop^r_{X}}{\wtd y}
  \propoutrec{k+1}{\wtd y}X \Par R 
  \Par  
  \proprinpk{r}{k}{\wtd x}\propoutrecsh{\rvar{X}}{\wtd x}\rvar{X}:
   R \in \Dbrecpi{k}{\tilde x}{Q}^d_g \}$ $\cup N$ \\
   where: \\
   $M = 
   \begin{cases}
    \{  \news{\wtd \prop} (
    \recp{X}\binp{\prop^r_{X}}{\wtd y}
  \propoutrec{k+1}{\wtd y}X \Par R  \Par \\
  \propoutrecsh{\rvar{X}}{\wtd x\rho}
  \recp{X}\proprinpk{r}{k}{\wtd x}\propoutrecsh{\rvar{X}}{\wtd x}\rvar{X}
  )  \,:\, R \in \Dbrecpi{k}{\tilde x}{Q}^0_g \} & \text{ if } g \not= \es \\
  \{  \news{\wtd \prop} (
    \recp{X}\binp{\prop^r_{X}}{}
  \propoutrec{k+1}{}X \Par R  \Par  \\
  \apropoutrecsh{\rvar{X}}{} \Par 
  \recp{X}\proprinpk{r}{k}{}(\apropoutrecsh{\rvar{X}}{} \Par \rvar{X})
  )  \,:\, R \in \Dbrecpi{k}{\tilde x}{Q}^0_g \} & \text{ otherwise }
   \end{cases}$ 
   \\
  % $M_2 = \{  \news{\wtd \prop} (
  %   \recp{X}\binp{\prop^r_{X}}{\wtd y}
  % \propoutrec{k+1}{\wtd y}X \Par R$  \\
  % $\qquad \Par 
  % \proproutk{r}{\rvar{X}}{\wtd x\rho}
  % \recp{X}\proprinpk{r}{k}{\wtd x}\propoutrecsh{\rvar{X}}{\wtd x}\rvar{X}
  % )  \,:\, R \in \Dbrecpi{k}{\tilde x}{Q}^0_g \}$ \\
 $N =
  \begin{cases}
     \{  \news{\wtd \prop} (\propoutrec{k}{\wtd z\rho}
  \recp{X}\binp{\prop^r_{X}}{\wtd y}
\propoutrec{k}{\wtd y}X \Par \Brec{k}{\tilde x}{Q}_g ) \}
  % \\
  \cup~ M & \text{ if } \recdep = 0 \\ 
\emptyset & \text{otherwise}
  \end{cases}
  $
     \smallskip 
  \end{tabular}
  &
  %side-conditions
  \begin{tabular}{l}
    \noalign{\smallskip}
    % $\recdep = \rvardepth{Q}$
    $\wtd \prop = \fpn{R}$ \\
    $Q \equiv \recp{X} Q^*$ \\
    $\wtd x = \fs{Q^*}$ \\
    $g = \{ X \mapsto \wtd x\}$ \\
    $\rho = \subst{\tilde u}{\tilde x}$
    \smallskip
  \end{tabular}
  \\ 
      \rowcolor{gray!25}
      \hline
      $P$ &
        \multicolumn{2}{l|}{
      \begin{tabular}{l}
        \noalign{\smallskip}
        $\Dbrecpi{k}{\tilde x, \rho}{P}^d_g$ $\text{ when } 
        g  \not= \es$
        \smallskip
      \end{tabular}
    } 
     \\
      \hline
             %%%%%%
    %% =======================
    %% =======================
    %%%%%%
    % $\Dbrecpi{k}{\tilde x, \rho}{\bout{u_i}{y_j}{Q}}^d_g$ & 
    $\bout{n_i}{y_j}{Q}$ &
    \begin{tabular}{l}
    \noalign{\smallskip}
    $\{\bout{n_l}{\wtd y\rho} \propoutrec{k+1}{\wtd z\rho}
    \recp{X}\binp{\prop^r_k}{\wtd x}
    \bout{n_l}{\wtd y} 
    \propoutrec{k+1}{\wtd z}\rvar{X}
  \Par$ 
  %  \\
  $\Brec{k+1}{\tilde z}{Q\sigma}_g \}$ $\text{ if } \rvardepth{Q} = \recdep$
  \\
  \hdashline 
  \noalign{\smallskip}
  $N \cup \{\recp{X}\binp{\prop^r_k}{\wtd x}
    \bout{n_l}{\wtd y} 
    \propoutrec{k+1}{\wtd z}\rvar{X}
  \Par$ 
  %  \\
  $R : R \in \Dbrecpi{k+1}{\tilde z, \rho}{Q\sigma}^d_g\}$ $\text{ otherwise }$
  \\
  % \hdashline 
  % \noalign{\smallskip}
  where: \\
  $ N = 
\begin{cases}
  \{\propoutrec{k+1}{\wtd z\rho}
  \recp{X}\binp{\prop^r_k}{\wtd x}
  \bout{n_l}{\wtd y} 
  \propoutrec{k+1}{\wtd z}\rvar{X}
 \Par \Brec{k+1}{\tilde z}{Q\sigma}_g \} & \text{if } \rvardepth{Q} = \recdep + 1 \\ 
  \es & \text{otherwise}
\end{cases} 
$
%   \\
%   $ \qquad N = \{\propoutrec{k+1}{\wtd z\rho}
%   \recp{X}\binp{\prop^r_k}{\wtd x}
%   \bout{n_l}{\wtd y} 
%   \propoutrec{k+1}{\wtd z}\rvar{X}
%  \Par$ 
% $\Brec{k+1}{\tilde z}{Q\sigma}_g \}$ $\text{ if } \rvardepth{Q} = \recdep + 1$  \\
%   $\qquad N = \es$ $\texttt{ otherwise }$
  \smallskip
\end{tabular} & 
\begin{tabular}{l}
       \noalign{\smallskip}
       $y : T$ $\wedge (y_j,\ldots,y_{j+\len{\Gt{T}}-1})$ \\ 
    % $r:S \wedge \mathsf{tr}(S)$ \\
    $\wtd w = \linecondit{\lin{u_i}}{\{ u_i \}}{\epsilon}$ \\
    $\wtd z = g(X) \cup \fnb{Q}{\wtd x \setminus \wtd w}$  \\
    $l = \linecondit{\mathtt{tr}(u_i)}{f(S)}{i}$ \\
    $\sigma = \nextn{u_i}$
    \smallskip
\end{tabular} 
\\
\hline 
% $\Dbrecpi{k}{\tilde x}{\binp{u_i}{y}{Q}}^d_g$
$\binp{n_i}{y}{Q}$
&
\begin{tabular}{l}
    \noalign{\smallskip}
     $\{\binp{n_l}{\wtd y} 
    \propoutrec{k+1}{\wtd z\rho}
    \recp{X}\binp{\prop^r_k}{\wtd x}
      \binp{n_l}{\wtd y} 
      \propoutrec{k+1}{\wtd z}
      \rvar{X}
     \Par$ 
    %  \\
    $\Brec{k+1}{\tilde z}{Q\sigma}_g \}$ $\text{ if } \rvardepth{Q} = \recdep$
    \\
    \hdashline 
    \noalign{\smallskip}
    $N \cup \{\recp{X}\binp{\prop^r_k}{\widetilde x}
      \binp{n_l}{\widetilde y} 
      \propoutrec{k+1}{\wtd z}
      \rvar{X}
     \Par$ 
    %  \\
    $R : R \in \Dbrecpi{k+1}{\tilde z, \rho}{Q\sigma}^d_g\}$
    \\
    % \hdashline 
    % \noalign{\smallskip}
    $N = 
    \begin{cases} 
      \{\propoutrec{k+1}{\wtd z\rho}
    \recp{X}\binp{\prop^r_k}{\wtd x}
      \binp{n_l}{\wtd y} 
      \propoutrec{k+1}{\wtd z}
      \rvar{X}
     \Par
    \Brec{k+1}{\tilde z}{Q\sigma}_g \} & \text{ if } \rvardepth{Q} = \recdep + 1 \\
    \es & \text{ otherwise }
    \end{cases}
    $
    \smallskip 
\end{tabular} & 
\begin{tabular}{l}
       \noalign{\smallskip}
    % $r:S \wedge \mathsf{tr}(S)$ \\
    $\wtd w = \linecondit{\lin{u_i}}{\{ u_i \}}{\epsilon}$ \\
    $\wtd z = g(X) \cup \fnb{Q}{\wtd x \wtd y \setminus \wtd w}$  \\
    $l = \linecondit{\mathtt{tr}(u_i)}{f(S)}{i}$ \\
    $\sigma = \nextn{u_i} \cdot \subst{y_1}{y}$
    % $\wtd z = \fnb{Q}{\wtd x \wtd y}$  
    \smallskip
\end{tabular} 
\\
\hline
% $\Dbrecpi{k}{\tilde x,\rho}{Q_1 \Par Q_2}^d_g$
$Q_1 \Par Q_2$
& 
\begin{tabular}{l}
    \noalign{\smallskip}
    $ N \cup \{\recp{X}\proprinpk{r}{k}{\wtd x}
    (\proproutk{r}{k+1}{\wtd y_1}\rvar{X}
    \Par \apropoutrecsh{k+\degree+1}{\wtd y_2}) 
     \Par$ 
    %  \\
    $R_1 \Par R_2 :$  \\
    $R_1 \in \Dbrecpi{k+1}{\tilde y_1, \rho}{Q_1}^d_{g_1}, 
    R_2 \in \Dbrecpi{k+\degree+1}{\tilde y_2, \rho}{Q_2}^d_{g_2}\}$ 
    % $\cup$ $N$
    \\
    \hdashline 
    \noalign{\smallskip}
    $ N = 
    \begin{cases} 
   \{\proproutk{r}{k+1}{\wtd y_1\rho}
    \recp{X}\proprinpk{r}{k}{\wtd x} (\proproutk{r}{k+1}{\wtd y_1}\rvar{X}
    \Par 
    \apropoutrecsh{k+\degree+1}{\wtd y_2})
     \Par
    %  \\
    \\ \Brec{k+1}{\tilde y_1}{Q_1}_{g_1} \Par 
    \Brec{k+\degree+1}{\tilde y_2}{Q_2}_{g_2}\} & \text{ if } \rvardepth{Q_1} = \recdep \\
    \es & \text{ otherwise }
    \end{cases}
    $
    \smallskip 
  \smallskip
\end{tabular} & 
\begin{tabular}{l}
         \noalign{\smallskip}
         $\recpx{Q_1}$ \\
         $\wtd y_1  = g(X) \cup \fnb{Q_1}{\wtd x}$ \\
         $\wtd y_2  =  \fnb{Q_2}{\wtd x}$ \\
        %  $i \in \{1,2\}.$ \\
        %  $\quad \wtd y_i' = \linecondit{\recpx{Q_i}}{g(X)}{\epsilon}$ \\
        %  $\quad g_i = \linecondit{\recpx{Q_i}}{g_i}{\epsilon}$ \\
        %  $\quad \wtd y_i  = \wtd y_i' \cup \fnb{Q_i}{\wtd x}$ \\
         $\degree = \lenHOopt{Q_1}$
    \smallskip
\end{tabular} 
\\
\hline
% $\Dbrecpi{k}{\tilde x, \rho}{\news{s:C}{Q}}^d_g$ & 
$\news{s:C}{Q}$ &
\begin{tabular}{l}
    \noalign{\smallskip}
    $N \cup \{\recp{X}\news{\widetilde{s}:\Gt{C}}\propinp{k}{\wtd x}\propout{k+1}{\wtd z}X$
    $\Par$
    $R : R \in \Dbrecpi{k+1}{\tilde z, \rho}{Q \sigma }^d_g \}$
    \\
    \hdashline 
    \noalign{\smallskip}
    $R = \propout{k+1}{\wtd z\rho}
    \recp{X}\news{\wtd{s}:\Gt{C}}\propinp{k}{\wtd x}\propout{k+1}{\wtd z}X$ \\
    $ N = 
    \begin{cases}
    \{\news{\wtd{s}:\Gt{C}}R
    \Par
    \Brec{k+1}{\tilde z}{Q\sigma}_g\} &  \text{ if } \rvardepth{Q_1} = \recdep \\
    \es & \text{ otherwise }
    \end{cases}
    $
  \smallskip
\end{tabular} & 
\begin{tabular}{l}
    \noalign{\smallskip}
      %  $\mathsf{tr}(\trec{t}{S})$ \\
       $\widetilde{s} = (s_1,\ldots,s_{\len{\Gt{S}}})$ \\
       $\widetilde {\dual{s}} =  (\dual{s_1},\ldots,\dual{s_{\len{\Gt{S}}}})$ \\
       $\wtd n =
        \linecondit{\lin{s}}{\wtd n}{\epsilon}$ \\
%        $\widetilde {\dual{s}} = \begin{cases}
%         (\dual{s_1},\ldots,\dual{s_{\len{\Gt{S}}}}) & \text{if} \ C = S \\
%         \epsilon & \text{if} \ C = \chtype{U}
% \end{cases}
% $\\
      %  $\widetilde {\dual{s}} = (\dual{s_1},\ldots,\dual{s_{\len{\Rtopt{S}}}})$ \\
       $\wtd z = \wtd x, \wtd s, \wtd n$ \\
       $\sigma = \subst{s_1 \dual{s_1}}{s \dual{s}} $
    \smallskip
\end{tabular} 
\\
\hline
% $\Brec{k}{\tilde x}{X}_g$ 
$X$
&  
\begin{tabular}{l}
\noalign{\smallskip}
$\inact$
\smallskip
\end{tabular}
& 
\begin{tabular}{l}
       \noalign{\smallskip}
      %  $\wtd x = g(X)$
    \smallskip
\end{tabular} 

\\ 
      \rowcolor{gray!25}
      \hline
      $P$ &
        \multicolumn{2}{l|}{
      \begin{tabular}{l}
        \noalign{\smallskip}
        $\Dbrecpi{k}{\tilde x, \rho}{P}^d_g$ $\text{ when } g = \es$
        \smallskip
      \end{tabular}
    } 
     \\
      \hline
             %%%%%%
    %% =======================
    %% =======================
    %%%%%%
    $\bout{n_i}{y_j}{Q}$
    &  
    \begin{tabular}{l}
    \noalign{\smallskip}
    $ \{
    \bout{n_{\mstindex}}{\wtd y\rho} \apropoutrecsh{k+1}{\wtd z\rho} \Par  
    \recp{X}\propinprecsh{k}{\wtd x}
    (\bout{n_{\mstindex}}{\wtd y} \apropoutrecsh{k+1}{\wtd z}
    \Par \rvar{X}) 
   \Par$
  $\Brec{k+1}{\tilde z}{Q\sigma}_g \}$
    \smallskip
    \end{tabular}
    & 
    \begin{tabular}{l}
           \noalign{\smallskip}
          %  $\wtd x = g(X)$
        \smallskip
    \end{tabular} 
\\ \hline     
$\binp{n_i}{y}{Q}$
&  
\begin{tabular}{l}
\noalign{\smallskip}
$
\{\binp{n_{\mstindex}}{\wtd y} \apropoutrecsh{k+1}{\wtd z\rho}  \Par 
\recp{X}\propinprecsh{k}{\wtd x}
(\binp{n_{\mstindex}}{\wtd y} 
\apropoutrecsh{k+1}{\wtd z} \Par \rvar{X}) 
\Par$ 
%  \\
$\Brec{k+1}{\tilde z}{Q\sigma}_g\}$ 
\smallskip
\end{tabular}
& 
\begin{tabular}{l}
       \noalign{\smallskip}
      %  $\wtd x = g(X)$
    \smallskip
\end{tabular} 
\\ \hline    
$Q_1 \Par Q_2$
&  
\begin{tabular}{l}
\noalign{\smallskip}
$
\{\apropoutrecsh{k+1}{\wtd y_1\rho}
\Par \apropoutrecsh{k+\degree+1}{\wtd y_2\rho} \Par 
\recp{X}\proprinpk{r}{k}{\wtd x}(\apropoutrecsh{k+1}{\wtd y_1}
\Par \apropoutrecsh{k+\degree+1}{\wtd y_2} \Par \rvar{X})
 \Par$ 
 \\
$\Brec{k+1}{\tilde y_1}{Q_1}_{g_1} \Par 
\Brec{k+\degree+1}{\tilde y_2}{Q_2}_{g_2}\}$ 
\smallskip
\end{tabular}
& 
\begin{tabular}{l}
       \noalign{\smallskip}
      %  $\wtd x = g(X)$
    \smallskip
\end{tabular} 
\\ \hline    
$\news{s:C}{Q}$ 
&  
\begin{tabular}{l}
\noalign{\smallskip}
$
\{\apropoutrecsh{k+1}{\wtd z\rho} \Par 
\recp{X}\news{\wtd{s}:\Gt{C}}
\propinp{k}{\wtd x}(\apropoutrecsh{k+1}{\wtd z} \Par X)$
$\Par$
$\Brec{k+1}{\tilde z}{Q}_g\}$
\smallskip
\end{tabular}
& 
\begin{tabular}{l}
       \noalign{\smallskip}
      %  $\wtd x = g(X)$
    \smallskip
\end{tabular} 
\\ \hline    
    \end{tabular}
    \caption{The extension of $\Cbpi{\tilde u}{\tilde x}{P}$ 
    and definition of $\Dbrecpi{k}{\tilde x, \rho}{P}^d_g$
    (recursion extension). Side conditions for 
    last four rows ($g = \es$) are the same as for corresponding 
    cases when $g \not = \es$. \label{t:tablecd-rec}}
    \vspace{-2mm}
    \end{table}
\end{figure*}

 \begin{definition}[Indexed names substitutions]
   \label{d:indexedsubstitution}
   Let 
   $$\widetilde u = (a,b,s, \dual s, \dual{s}', s',r, r', \ldots)$$ 
   be a finite tuple of names.
   We write $\indices{\wtd u}$ to denote 
   $$\indices{\wtd u} = 
   \{\subst{a_{1}, b_{1}, s_{i}, \dual s_{i},  
   s'_{j}, \dual s'_{j}, r_{1}, r'_{1}, \ldots}{a,b,s,s',r,r',\ldots} : 
   i,j,\ldots > 0 \}$$
 \end{definition}

\begin{definition}[Relation \relS]
  \label{d:relation-s}
  Let $P\subst{\tilde u}{\tilde x}$ be a well-typed process 
and let the $\mathcal{C}$-set be as in \tabref{t:tablecd}.
  We define the relation $\relS$ as follows: 
  \begin{align*}
    \relS &= \big\{(P\subst{\tilde u}{\tilde x}, R) :
        R \in \Cbpi{\bns{u}}{\bns{x}}{P\sigma} \\
        & \quad \quad \text{ with } 
    \wtd n = \fn{P} \cup \wtd u \cup \wtd x, \sigma \in \indices{\wtd n}, \\
    & \quad \quad \qquad \wbns{u} = \bn{\wtd u \sigma : \wtd C}, 
    \wbns x = \bn{\wtd x \sigma : \wtd C} 
    \big\}
  \end{align*}
  \noindent where $\wtd u : \wtd C$. 
\end{definition}

For the convenience, we define function $\Cbs{-}{-}{\cdot}$ 
relying on $\Cbpi{-}{-}{\cdot}$ as follows: 

\begin{definition}[Function  $\Cbs{-}{-}{\cdot}$ ]
  \label{d:cbs}
  Let $P$ be a process, $\rho$ be a name substitution, and $\sigma$ be an indexed 
  name substitution. We define $\Cbs{\rho}{\sigma}{P}$ as follows: 
  \begin{align*}
    \Cbs{\rho}{\sigma}{P_1}  &= \Cbpi{\bns{u}}{\bns{x}}{P\sigma} \\
        & \quad \text{ with } 
        \rho = \subst{\tilde u}{\tilde x}, 
    % \wtd n = \fn{P} \cup \wtd u \cup \wtd x, \sigma \in \indices{\wtd n}, \\
      \wbns{u} = \bn{\wtd u \sigma : \wtd C}, 
    \wbns x = \bn{\wtd x \sigma : \wtd C} 
  \end{align*}
  \noindent where $\wtd u : \wtd C$. 
\end{definition}

\subsection{Operational correspondence}
\label{app:ss:oc}

\begin{lemma}
  \label{l:c-prop-closed}
  Given an indexed process $P_1\subst{\tilde u}{\tilde x}$, 
  the set $\Cbpi{\tilde u}{\tilde x}{P_1}$ is closed under $\tau$ transitions on
  non-essential prefixes. That is, 
   if $R_1 \in \Cbpi{\tilde u}{\tilde x}{P_1}$ 
  and $R_1 \by{\tau} R_2$ is inferred from the actions on non-essential prefixes, 
  then $R_2 \in \Cbpi{\tilde u}{\tilde x}{P_1}$.
\end{lemma}
\begin{proof}[Sketch]
  By the induction on the structure of $P_1$ and 
  the inspection of definition of $\Cbpi{-}{-}{\cdot}$ 
  and $\Dbpi{-}{-}{\cdot}$
  in \tabref{t:tablecd} and \tabref{t:tablecd-rec}. 
\end{proof}

\begin{lemma}
  \label{l:processrelate-mst}
  Relation $\processrelate$ is a MST bisimulation. 
\end{lemma}
\begin{proof}[Sketch]
  Straightforward by the transition induction and \defref{def:valuesprelation}. 
\end{proof}

\lemms* 

\begin{proof} 
  \label{app:lemms}
 By transition induction. 
%  Then, we analyze inductive cases. 
  Let $\rho_1 = \subst{\tilde u}{\tilde x}$. 
  By inversion of $P_1 \relS Q_1$ 
  we know there is $\sigma_1 \in \indices{\fn{P_1} \cup \wtd u \cup \wtd x}$, 
  % $\wbns{u}=\bn{\wtd u \sigma_1}$, $\wbns{x}=\bn{\wtd x \sigma_1}$, 
  % such that $Q_1 \in \Cbpi{\bns u}{\bns x}{P_1\sigma_1}$.
  such that $Q_1 \in \Cbs{\rho_1}{\sigma_1}{P_1}$. 
  We need the following assertion on the index substitution. 
  If $P_1\rho_1 \by{\ell} P_2\rho_2$ and $\subj{\ell}=n$ then there exists $Q_2$
  such that $Q_1 \by{\iname \ell} Q_2$ 
  with $\subj{\iname \ell} = n_i$ and $Q_2 \in \Cbs{\rho_2}{\sigma_2}{P_2}$
  such that $\sigma_2 \in \indices{P_2\rho_2}$
  with $\nextn{n_i} \in \sigma_2$. 
%  and 
%  $Q_2 \in \Cbs{\rho_2}{\sigma_2}{P_2}$
%  % $Q_2 \in \Cbpi{\bns u'}{\bns x'}{P_2\sigma_2}$ 
%  for some $\rho_2$, and for some $\sigma_2'$ we have 
%  % $\sigma_2 = \sigma_1 \cdot \incrname{n}{i}$
%  $\sigma_2 = \sigma_2' \cdot \sigma_1 \cdot \incrname{n}{i}$
%  with $n_i = \subj{\iname \ell}$.  

  First, we consider two base cases: Rules~\texttt{Snd} and 
  \texttt{Rv}. Then, we consider inductive cases: 
  Rules~$\texttt{Par}_{\texttt{L}}$ and $\texttt{Tau}$. 
  We omit inductive cases $\texttt{New}$ and $\texttt{Res}$
  as they follow directly by the inductive hypothesis and the 
  definition of the restriction case in $\Cbpi{-}{-}{\cdot}$
  (\tabref{t:tablecd}). 
  Finally, we separately treat cases when a process is recursive.
  We show two cases (\texttt{Rv} and $\texttt{Par}_{\texttt{L}}$) 
  emphasizing specifics of the recursion breakdown. 
%  Let $\rho = \subst{\tilde u}{\tilde x}$ 
%  in every case. 
 \begin{enumerate}
   \item Case \texttt{Snd}. 
   We distinguish two sub-cases: \rom{1} 
   $P_1 = \bout{n}{v}P_2$
   and \rom{2} $P_1 = \bout{n}{y}P_2$ with 
   $\subst{v}{y} \in \rho_1$. 
   In both sub-cases we know there is 
    $\rho_2 = \subst{\tilde u_2}{\tilde x_2}$ such that
   $$P_1\rho_1 = \bout{n\rho_1}{v}P_2\rho_2$$ 

   We have the following transition: 
   \begin{align*} 
    \AxiomC{} 
    \LeftLabel{\scriptsize $\rulename{Snd}{}$}
    \UnaryInfC{$P_1\rho_1
    \by{\bactout{n\rho_1}{v}} 
    P_2 \rho_2
    $}
    \DisplayProof
  \end{align*}
  
  Let $\sigma_1 \in \indices{\wtd p}$ where 
  $\wtd p = \indices{\fn{P_1} \cup \wtd u \cup \wtd x}$ such that 
  $\subst{n_i}{n} \in \sigma_1$. 
   Also, let $\sigma_2 = \sigma_1 \cdot \nextn{n_i}$. 
%  
%  Let $\sigma_1 = \sigma' \cdot \initname{n}{i}$  where 
%  $\sigma' \in \indices{\fn{P_1} \cup \wtd u \cup \wtd x}$ 
%  and $\sigma_2 = \sigma_1 \cdot \sigma$ where $\sigma = \nextn{n_i}$. 
  Here we take $\sigmav = \sigma_2$. 
  Further, let $\wbns{u} =\bname{\wtd u \sigma_1 : \wtd C}$
  and $\wbns{x} =\bname{\wtd x \sigma_1 : \wtd C}$ with $\wtd u : \wtd C$. 
  Also, let $\wtd z = \fnb{P_2}{\wbns{x} \setminus \wtd w}$ 
  where $\wtd w = \{n_i\}$ if $\lin{n_i}$ otherwise $\wtd w = \epsilon$. 
  Then, in both sub-cases, there are two possibilities for the shape of $Q_1$, namely: 
  \begin{align*}
    Q^1_1 &= \news{\wtd \prop_k}(\apropout{k}{\wbns u} \Par
    \B{k}{\bns x}{P_1  \sigma_1}) \\
    Q^2_1 &= \news{\wtd \prop_{k+1}} \bout{n_i \rho_*}{\wtd v} 
    \apropout{k+1}{\wtd z \rho_*}
   \Par \B{k+1}{\tilde z}{P_2\sigma_2}
  \end{align*}

  \noindent 
  % where $v_j \valuesrelate \wtd v$.   
  where $v\sigmav \valuesrelate \wtd v$ 
  and $\rho_* = \subst{\wtd u_*}{\wtd x_*}$
  By \lemref{l:c-prop-closed} we know that $Q^1_1 \by{\tau} Q^2_1$. 
  Thus, we only consider how $Q^2_1$ evolves. 
  We can infer the following: 
  $$Q^2_1 \by{\bactout{n_i\rho_*}{\tilde v}} Q_2$$
  \noindent where $Q_2 =\news{\wtd \prop_{k+1}}\apropout{k+1}{\wtd z \rho_*}
  \Par \B{k+1}{\tilde z}{P_2\sigma_2}$. Then, we should show the following: 
  \begin{align}
    \label{eq:snd-goal1}
  {(P_2 \parallel \ftrigger{t}{v}{C_1})\rho_2 }
    \ \relS \ 
  {Q_2 \parallel \ftriggerm{t}{v\sigmav}{C_1}}
  \end{align}

  % First, we can see that if $

  By \tabref{t:tablecd} we can see that 
  \begin{align} 
    \label{eq:snd-c-r1}
    Q_2 \in \Cbpi{\tilde z \rho_*}{\tilde z}{P_2\sigma_2}
  \end{align} 
  
  Here we remark that our assertion holds by the construction as we have
  $\sigma_2=\sigma_1\cdot \nextn{n_i}$. 

  By \defref{d:fnb} and \defref{d:name-breakdown} we know that 
  % there are $\wtd u_2$ and $\wtd x_2$ such that 
  % \begin{align*}
  %   P_2\subst{\tilde u}{\tilde x} = P_2\subst{\tilde u_2}{\tilde x_2}
  % \end{align*}
  % and 
  % \begin{align*}
  %   \wtd z = \fnb{P_2}{\bname{\wtd x : \wtd C} \setminus \wtd w} = 
  %   \bname{\wtd x_2 \sigma_1 \cdot \sigma : \wtd C_2}
  % \end{align*}
  \begin{align*}
    \wtd z = \fnb{P_2}{\bname{\wtd x : \wtd C} \setminus \wtd w} = 
    \bname{\wtd x_2 \sigma_2 : \wtd C_2}
  \end{align*}
  \noindent with $\wtd x_2 : \wtd C_2$. 
   Similarly, we have 
  $$\wtd z\rho_* = \bname{\wtd x_2 \rho_2 \sigma_2: \wtd C_2}$$ 
  % $$\wtd z\rho_* = \bname{\wtd x_2 \rho_2 \sigma_1 \cdot \sigma : \wtd C_2}$$ 

  Now, by the assumption $\dual n \not\in \wtd v$ 
  we know $\subst{\dual n_i}{\dual n} \not\in \sigma_2$.  
  Thus, by $\sigma_2 = \sigma_1 \cdot \nextn{n_i}$
  and \defref{d:indexedsubstitution}, we have 
  $$\sigma_2 \in \indices{\wtd p}$$ 

  Further, we know there is 
  $$\sigma_2' \in \indices{\fn{P_2\rho_2}}$$ 
%  $$\sigma_2' \in \indices{\fn{P_2} \cup \wtd u_2 \cup \wtd x_2}$$ 
%      $$\sigma_2' \in \indices{\fn{P_2} \cup \wtd u_2 \cup \wtd x_2}$$ 

  such that 
  $P_2\rho_2 \sigma_2 = P_2\rho_2\sigma_2'$. 
  Thus, by this and \eqref{eq:snd-c-r1} we have that $P_2\rho_2 \relS Q_2$. 
  Next, by the definition we have 
  $\ftrigger{t}{v}{C_1} \relS \ftriggerm{t}{v\rho\sigma}{C_1}$. 
  Thus,  the goal \eqref{eq:snd-goal1} follows. 
  This concludes \texttt{Snd} case. 

  \item Case \texttt{Rv}. Here we know $P_1 = \binp{n}{y}P_2$. 
 We know there is $\rho_2 = \subst{\tilde u_2}{\tilde x_2}$
 such that 
 $$P_1\rho_1 = \binp{n\rho_1}{y}P_2\rho_2$$

  The transition is as follows: 
  \begin{align*}
    \AxiomC{} 
    \LeftLabel{\scriptsize $\rulename{Rv}{}$}
    \UnaryInfC{$\binp{n\rho_1}{y}P_2\rho_2 \by{\abinp{n}{v}} 
    P_2 \rho_2 \cdot \subst{v}{y}$}
    \DisplayProof  	
  \end{align*}
  Let $\sigma_1 = \sigma' \cdot \initname{n}{i}$  where 
  $\sigma' \in \indices{\fn{P_1} \cup \wtd u \cup \wtd x}$ 
  and $\sigma_2 = \sigma_1 \cdot \sigma$ where 
  $\sigma = \nextn{n_i} \cdot \initname{y}{1}$.
  Further, let $\wbns u =\bname{\wtd u \sigma_1 : \wtd C}$
  and $\wbns x =\bname{\wtd x \sigma_1 : \wtd C}$ with $\wtd u : \wtd C$. 
  Also, let 
  $\wtd y = (y_1,\ldots,y_{\len{\Gt{S}}})$ and 
  $\wtd z = \fnb{P_2}{\wbns x \wtd y \setminus \wtd w}$ 
  where $\wtd w = \{n_i\}$ if $\lin{n_i}$ otherwise $\wtd w = \epsilon$. 
  Then, there are two possibilities for the shape of $Q_1$, namely: 
  \begin{align*}
    Q^1_1 &= \news{\wtd \prop_k}(\apropout{k}{\wbns u} \Par
    \B{k}{\bns x}{P_1  \sigma_1}) \\
    Q^2_1 &= \news{\wtd \prop_{k+1}} \binp{n_i \rho}{\wtd y} 
    \apropout{k+1}{\wtd z \rho}
   \Par \B{k+1}{\tilde z}{P_2\sigma_2}
  \end{align*}

  By \lemref{l:c-prop-closed} we know that $Q^1_1 \by{\tau} Q^2_1$. 
  Thus, we only consider how $Q^2_1$ evolves. 
  We can infer the following: 
  \begin{align*}
    Q^2_1 \by{\bactinp{n_i\rho}{\wtd v}} Q_2 
  \end{align*}
  \noindent where 
  $Q_2 = \news{\wtd \prop_{k+1}}\apropout{k+1}{\wtd z \rho \cdot \subst{\tilde v}{\tilde y}}
  \Par \B{k+1}{\tilde z}{P_2\sigma_2}$ 
  and $v\sigmav \valuesrelate \wtd v$ for some $\sigmav \in \indices{v}$.
  Now, we should show the following: 
  \begin{align}
    \label{eq:fo-rv-goal1}
    P_2\rho_2 \cdot \subst{v}{y} \relS Q_2 
  \end{align}

  By \tabref{t:tablecd} we can see that 
  \begin{align} 
    \label{eq:rv-c-r1}
    Q_2 \in 
    \Cbpi{\tilde z \rho_2 \cdot \subst{\tilde v}{\tilde y}}{\tilde z}{P_2\sigma_2 \cdot \sigmav}
  \end{align} 

  Here we remark that 
  $\sigma_2 \cdot \sigmav= \sigmav \cdot \sigma_1 \cdot \incrname{n}{i}$. 
  Further, we may notice that 
  $$\sigma_2 \cdot \sigmav \in \indices{\fn{P_2} \cup \wtd u_2 \cup \wtd x_2}$$

  By \defref{d:fnb} and \defref{d:name-breakdown} we have that 
  \begin{align*}
    \wtd z &= \fnb{P_2}{\bname{\wtd x : \wtd C}\cdot \wtd y \setminus \wtd w} \\
     &= 
    \bname{\wtd x y (\sigma_1 \cdot \sigma ): \wtd C S} 
  \end{align*}
  \noindent with $y : S$. Similarly, we have 
  \begin{align*}
    \wtd z \rho_2 \cdot \subst{\tilde v}{\tilde y} =  
     \bname{\wtd x y \rho_2 \cdot \subst{v}{y}(\sigma_2 \cdot \sigmav ): \wtd C S} 
  \end{align*}

  % Further, we may notice that 
  % $$\sigma_2 \cdot \sigmav \in \indices $$

  Thus, by this and \eqref{eq:rv-c-r1} the goal 
  \eqref{eq:fo-rv-goal1} follows. 
  This concludes \texttt{Rv} case (and the base cases).
  We remark that base cases concerning triggers collection processes 
  follow by  \lemref{l:processrelate-mst}. 
  Next, we consider inductive cases. 

  \item Case $\texttt{Par}_{\texttt{L}}$. 
  Here we know  $P_1 = P'_1 \Par P''_1$.
  % We distinguish two sub-cases: 
  % \rom{1} $P_1 = P'_1 \Par P''_1$ and \rom{2} $P_1 = H_1 \parallel P''_1$ 
  % where $H_1$ is a triggers collection. 
  % We only consider sub-case \rom{1} as sub-case \rom{2} is similar using 
  % \lemref{l:processrelate-mst}. 
  The final rule in the inference tree is 
  as follows: 
  \begin{align*} 
  \AxiomC{$P_1' \subst{\tilde u'_1}{\tilde y_1} \by{\ell} 
  P_2' \subst{\tilde u'_2}{\tilde y_2} $} 
  \AxiomC{$\bn{\ell} \cap \fn{P_1''} = \emptyset$} 
  \LeftLabel{\scriptsize $\rulename{Par}{_L}$}
  \BinaryInfC{$P_1' \subst{\tilde u'_1}{\tilde y_1} \Par 
  P_1'' \subst{\tilde u''_1}{\tilde z_1}
  \by{\ell} P_2' \subst{\tilde u'_2}{\tilde y_2} \Par P_1''\subst{\tilde u''_1}{\tilde z_2}$} 	
  \DisplayProof 
  \end{align*}

  Let $\sigma_1 \in \indices{\fn{P_1}\cup \wtd u \cup \wtd x}$. 
  Further, let $\wtd y = \fnb{P_1'}{\wbns x}$, 
  $\wtd z = \fnb{P_1''}{\wbns x}$, $\wbns{u} =\bname{\wtd u \sigma_1 : \wtd C}$,
   $\wbns{x} =\bname{\wtd x \sigma_1 : \wtd C}$ with $\wtd u : \wtd C$, and 
   $\rhom=\subst{\bns u}{\bns x}$. 
  In sub-case \rom{1}, by the definition of $\relS$
  (\tabref{t:tablecd}), there are following possibilities for $Q_1$: 
    \begin{align*}
      Q^1_1 &= \news{\wtd \prop_k}(\apropout{k}{\wbns u} \Par
      \B{k}{\bns x}{P_1  \sigma_1}) \\
      Q^2_1 &= \propout{k}{\wtd y \rhom}
      \apropout{k+\degree}{\wtd z \rhom}   \Par
      \B{k}{\tilde y}{P'_1\sigma_1} \Par \B{k+\degree}{\tilde z}{P''_1\sigma_1} \\
      N^3_1 &= \{(R'_1 \Par R''_1) :
      \Cbpi{\tilde y\rhom}{\tilde y}{P'_1\sigma_1}, R''_1 \in 
      \Cbpi{\tilde z\rhom}{\tilde z}{P''_1 \sigma_1}\}
    \end{align*}
    By \lemref{l:c-prop-closed} there exist 
    \begin{align}
      Q'_1 &\in \Cbpi{\tilde y\rhom}{\tilde y}{P_1'\sigma_1}
    \\
      Q''_1 &\in \Cbpi{\tilde z\rhom}{\tilde z}{P_1''\sigma_1}
      \label{eq:fo-parl-q''_1}
    \end{align}
    such that 
  \begin{align*}
    Q^1_1 \By{\tau} Q^2_1 \By{\tau} Q'_1 \Par Q''_1
  \end{align*}

  Thus, in both cases we consider how $Q'_1 \Par Q''_1$
evolves. 
By the definition of $\relS$ we have 
\begin{align} 
  &P_1' \rho_1' \relS Q'_1 
  \label{fo-parl-q'1}
  \\
  &P_1'' \rho_1'' \relS Q''_1
  \label{fo-parl-q''1}
\end{align}

% By unfolding \defref{d:relation-s} we know 
% % there are $\sigma_1' \in \indices{\fn{P_1'} \cup \rho_1'}$ and 
% % $\sigma_1'' \in \indices{\fn{P_1''} \cup \rho_1''}$
% % such that  
% \begin{align}
%   Q_1' &\in \Cbs{\rho_1'}{\sigma_1}{P_1'} 
%   \label{fo-parl-q'1-2}
%   \\
%   Q_1'' &\in \Cbs{\rho_1''}{\sigma_1}{P_1''}
%   \label{fo-parl-q''1-2}
% \end{align}

To apply IH we do the case analysis on the action $\ell$: 
\begin{itemize}
  \item Sub-case $\ell \equiv \bactinp{n}{v}$. 
  If $v \in \wtd u$ then we take 
  $\sigmav = \sigma_1$, otherwise 
  $\sigmav = \initname{v}{j}$ for  $j > 0$. 
  Then,  by applying IH to \eqref{fo-parl-q'1} we know there is 
  $Q'_2$ such that $Q'_1 \By{\bactinp{n}{\tilde v}} Q'_2$ and 
  \begin{align}
    \label{eq:fo-parl-ih2-inp}
    P_2' \subst{\tilde u'_2}{\tilde y_2} \ \relS \ Q_2' 	
    \end{align}
    \noindent where $v \sigmav \valuesrelate \wtd v$ 
    and $\wtd u'_2 =\wtd u'_1 \cdot \wtd v$. 
    We should show that 
    \begin{align}
      \label{eq:fo-parl-inp-goal}
      P_2' \rho_2' \Par 
      P_1'' \rho_1'' \relS Q_2' \Par Q_1'' 
    \end{align}
    \noindent where $\rho_2' = \subst{\tilde u'_2}{\tilde y_1}$ 
    and $\rho_1'' = \subst{\tilde u''_1}{\tilde z_1}$. 
    Let $\sigma_2 = \sigma_1 \cdot \nextn{n_i}$ 
    such that $\initname{n}{i} \in \sigma_1$. Then, by
     \eqref{eq:fo-parl-ih2-inp} we know 
    \begin{align}
      \label{eq:fo-parl-ih2-inp-2}
      Q_2' \in \Cbs{\rho'_2}{\sigma_2 \cdot \sigmav}{P_2'}
    \end{align}
    By the definition of $\sigmav$ and $\sigma_2$ we may see that 
    $$\Cbs{\rho_1''}{\sigma_2 \cdot \sigmav}{P_1''} = \Cbs{\rho_1''}{\sigma_1}{P_1''}$$
    So, by \eqref{eq:fo-parl-ih2-inp-2} and \eqref{eq:fo-parl-q''_1} we have 
    \begin{align} 
      \label{eq:fo-parl-inp-3}
     Q_2' \Par Q_1'' \in \Cbs{\rho'_2 \cdot \rho'_1}{\sigma_2 \cdot \sigmav}{P_2' \Par P_1''}
    \end{align} 
    Further, we may notice that  
    $\sigma_2 \cdot \sigma_v \in \indices{\fn{P_2' \Par P''_1} \cup \rho'_2 \cup \rho''_1}$. 
    So, by this and \eqref{eq:fo-parl-inp-3} the goal 
      \eqref{eq:fo-parl-inp-goal} follows. 
  
  \item Sub-case $\ell = \tau$. 
  By applying IH to \eqref{fo-parl-q'1} we know there is 
  $Q'_2$ such that $Q'_1 \By{\ell} Q'_2$ and 
  \begin{align}
    \label{eq:fo-parl-tau-ih2}
    P_2' \rho'_2 \ \relS \ Q_2' 	
    \end{align} 
    \noindent where $\rho'_2 = \subst{\tilde u'_2}{\tilde y_2}$. 
    We should show that 
    \begin{align}
      \label{eq:fo-parl-tau-goal}
      P_2' \rho_2' \Par 
      P_1'' \rho_1'' \relS Q_2' \Par Q_1'' 
    \end{align}
    By \eqref{eq:fo-parl-tau-ih2}, we know there is 
    $\sigma_2 \in \indices{\fn{P_2} \cup \rho'_2}$ such that  
    \begin{align*}
      Q_2' \in \Cbs{\rho'_2}{\sigma_2}{P_2'}
    \end{align*}
    Further, by remark we know that either 
  $\sigma_2' = \sigma_1 \cdot \incrname{n}{i} \cdot \incrname{\dual n}{i}$
  for some $n_i, \dual n_i \in \fn{P'_2 \rho'_2}$ and 
  $n_i, \dual n_i \not\in \fn{P''_1 \rho''_1}$ or 
  $\sigma_2' = \sigma_1$
  such that 
  $$\Cbs{\rho'_2}{\sigma_2}{P_2'} = \Cbs{\rho'_2}{\sigma_2'}{P_2'}$$ 
  
  By this  we have that 
  $$\Cbs{\rho'_1}{\sigma_2'}{P_1'} = \Cbs{\rho'_1}{\sigma_1}{P_1'}$$
  So, we know that 
  $$Q_2' \Par Q''_1 \in \Cbs{\rho'_2 \cdot \rho''_1}{\sigma_2'}{P'_2 \Par P''_1}$$
  By \eqref{eq:fo-parl-tau-ih2} and  \eqref{eq:fo-parl-q''_1} and the definition of $\sigma_2'$
  the goal \eqref{eq:fo-parl-tau-goal} follows. 

  \item Sub-case  $\ell \equiv \news{\wtd m_1}\about{n}{v:C_1}$. 
  Here we omit details on substitutions as they are similar 
  to the first sub-case. 
  By applying IH to 
  \eqref{fo-parl-q'1} we know there is 
  $Q'_2$ such that $Q'_1 \By{\ell} Q'_2$ and 
  \begin{align}
    \label{eq:fo-parl-out-ih1}
    &{\newsp{\wtd{m_1}}{P'_2 \parallel \ftrigger{t}{v}{C_1}}}
    \ \relS \\
    &{\newsp{\widetilde{m_2}}{Q'_2 \parallel \ftriggerm{t}{v\sigma_1}{C_1}}}
  \end{align}

  We should show that 
  \begin{align}
    \label{eq:fo-parl-out-goal}
    &{\newsp{\wtd{m_1}}{P'_2 \Par P''_1 \parallel \ftrigger{t}{v}{C_1}}}
    \ \relS \\
    &{\newsp{\widetilde{m_2}}{Q'_2 \Par P''_1 \parallel \ftriggerm{t}{v\sigma_1}{C_1}}}
  \end{align}

  By \defref{d:relation-s} and \tabref{t:tablecd} from 
  \eqref{eq:fo-parl-out-ih1} we can infer the following: 
  \begin{align}
    \label{eq:fo-parl-out-ih2}
    P_2' \subst{\tilde u'_1}{\tilde y'} \ \relS \ Q_2' 	
    \end{align}
    So, by \eqref{fo-parl-q''1} and \eqref{eq:fo-parl-out-ih2} 
  the goal   \eqref{eq:fo-parl-out-goal} follows. 
\end{itemize}
This concludes $\texttt{Par}_{\texttt{L}}$ case. 

\item Case \texttt{Tau}. 
Here we know $P_1 = P'_1 \Par P''_1$. 
Without the loss of generality, we assume
 $\ell_1 = \news{\wtd m_1}\about{\dual n_i}{v_1}$
and $\ell_2 = \abinp{n_i}{v_1}$. 
Let  $\rho_1' = \subst{\tilde u'_1}{\tilde y}$ and 
$\rho_1'' = \subst{\tilde u''_1}{\tilde z}$ 
such that 
$$P_1\rho_1 = P_1'\rho_1' \Par P''_1 \rho''_1$$ 

Then, the final rule in the inference tree is as follows: 
\begin{align*}
  \AxiomC{$P_1'\rho_1' \by{\ell_1} P_2' \rho_2'$} 
  \AxiomC{$P_1'' \rho_1'' 
  \by{\ell_2} P_2'' \rho_2'$} 
  \AxiomC{$\ell_1 \asymp \ell_2$} 
  \LeftLabel{\scriptsize $\rulename{Tau}{}$}
  \TrinaryInfC{$P_1' \rho_1' \Par P_1'' \rho_1''
  \by{\tau} 
  \news{\wtd m_1}(P_2'  \rho_2' 
  \Par P_2'' \rho''_2)$}	
  \DisplayProof
  \end{align*}

  Let $\sigma_1$, $\wtd y$, $\wtd z$, $\wbns u$, 
  $\wbns x$, and $\rhom$ be defined as in the previous case. 
  Further, $Q_1$ can have shapes: 
  $Q^1_1$, $Q^2_1$, and $N^3_1$ as in the previous case. 
  As in the previous case, we know that there are
    %% the below is already defined in the previous case, we can reuse it 
  % Let $\sigma_1 \in \indices{\fn{P_1}\cup \wtd u \cup \wtd x}$. 
  % Further, let $\wtd y = \fnb{P_1'}{\wbns x}$, 
  % $\wtd z = \fnb{P_1''}{\wbns x}$, $\wbns{u} =\bname{\wtd u \sigma_1 : \wtd C}$,
  %  $\wbns{x} =\bname{\wtd x \sigma_1 : \wtd C}$ with $\wtd u : \wtd C$, and 
  %  $\rhom=\subst{\bns u}{\bns x}$. 
  % Then, by the definition of $\relS$
  % (\tabref{t:tablecd}), there are following possibilities for $Q_1$: 
  %   \begin{align*}
  %     Q^1_1 &= \news{\wtd \prop_k}(\apropout{k}{\wbns u} \Par
  %     \B{k}{\bns x}{P_1  \sigma_1}) \\
  %     Q^2_1 &= \propout{k}{\wtd y \rhom}
  %     \apropout{k+\degree}{\wtd z \rhom}   \Par
  %     \B{k}{\tilde y}{P'_1\sigma_1} \Par \B{k+\degree}{\tilde z}{P''_1\sigma_1} \\
  %     N^3_1 &= \{(R'_1 \Par R''_1) :
  %     \Cbpi{\tilde y\rhom}{\tilde y}{P'_1\sigma_1}, R''_1 \in 
  %     \Cbpi{\tilde z\rhom}{\tilde z}{P''_1 \sigma_1}\}
  %   \end{align*}
    \begin{align}
      Q'_1 &\in \Cbpi{\tilde y\rhom}{\tilde y}{P_1'\sigma_1}
      \label{eq:fo-tau-q'_1} \\
      Q''_1 &\in \Cbpi{\tilde z\rhom}{\tilde z}{P_1''\sigma_1}
      \label{eq:fo-tau-q''_1}
    \end{align}
    such that 
  \begin{align*}
    Q^1_1 \By{\tau} Q^2_1 \By{\tau} Q'_1 \Par Q''_1
  \end{align*}

  Thus, in both cases we consider how $Q'_1 \Par Q''_1$
evolves. By the definition of $\relS$ we have 
\begin{align} 
  &P_1' \rho_1' \relS Q'_1 
  \label{fo-tau-q'1}
  \\
  &P_1'' \rho_1'' \relS Q''_1
  \label{fo-tau-q''1}
\end{align}
We apply IH component-wise: 
\begin{itemize}
  \item By applying IH to \eqref{fo-tau-q'1} we know there is 
  $Q'_2$ such that $Q'_1 \By{\news{\wtd m_2}\about{\dual n_i}{\tilde v}} Q'_2$
  and 
  \begin{align}
    \label{eq:fo-tau-out-ih1}
    &{\newsp{\wtd{m_1}}{P'_2 \parallel \ftrigger{t}{v}{C_1}}\rho'_2}
    \ \relS \\
    &{\newsp{\widetilde{m_2}}{Q'_2 \parallel \ftriggerm{t}{v\sigma_1}{C_1}}}
  \end{align}
  \noindent where $v\sigma_1 \valuesrelate \wtd v$. 
  \item By applying IH to \eqref{fo-tau-q''1}  we know there is
  $Q_2''$ such that $Q''_1 \By{\bactinp{n_i}{\tilde v}} Q''_2$ and 
  \begin{align}
    \label{eq:fo-tau-ih2}
    P_2'' \rho''_2 \ \relS \ Q_2'' 	
    \end{align}
\end{itemize}
Now, by \eqref{eq:fo-tau-out-ih1} we can infer: 
\begin{align*}
  P_2'\rho'_2 \relS Q_2'
\end{align*}

By this we know there is $\sigma_2' \in \indices{\fn{P_2'} \cup \rho'_2}$
such that 
\begin{align*}
  Q_2' \in \Cbs{\rho'_2}{\sigma_2'}{P_2'}
\end{align*}

Moreover, we know that it must be 
$\sigma_2' \subseteq \sigma_1 \cdot \nextn{\dual n_i}$. 
So, we have 
\begin{align*}
  Q_2' \in \Cbs{\rho'_2}{\sigma_1 \cdot \nextn{\dual n_i}}{P_2'}
\end{align*}

Similarly, there is $\sigma_2'' \in \indices{\fn{P_2''} \cup \rho''_2}$
and $\sigma_2'' \subseteq \sigma_1 \cdot \nextn{\dual n_i}$, so 
we have the following  
\begin{align*}
  Q_2'' \in \Cbs{\rho''_2}{\sigma_1 \cdot \nextn{n_i}}{P_2''}
\end{align*}

% Further, by this we know that 
% \begin{align*}
%   Q_2' \in \Cbpi{\bns u'_2}{\bns y}{P_2'\sigma_1 \cdot \nextn{n_i}} 
% \end{align*} 
% \noindent where $\bns u'_2 = \bname{\tilde u_2'\sigma_1 \cdot \nextn{n_i}}$. 
% Similarly,  by \eqref{fo-tau-q''1} we know that 
% \begin{align*}
%   Q_2'' \in \Cbpi{\bns u''_2}{\bns z}{P_2''\sigma_1 \cdot \nextn{n_i}} 
% \end{align*} 
% \noindent where $\bns u''_2 = \bname{\tilde u_2''\sigma_1 \cdot \nextn{n_i}}$.
% \todo[inline]{This should be part of IH? Should we reprhase the 
% statement then?}
So, we have 
\begin{align*}
  Q_2' \Par Q_2'' \in \Cbs{\rho'_2 \cdot \rho_2''}{\sigma_1 \cdot \nextn{n_i} 
  \cdot \nextn{\dual n_i}}
  {P_2' \Par P_2''}
\end{align*}
% \begin{align*}
%   Q_2' \Par Q_2'' \in \Cbpi{\bns u'_2 \cdot \bns u''_2}{\bns y' \cdot \bns z'}
%   {(P_2' \Par P_2'')\sigma_1 \cdot \nextn{n_i}}
% \end{align*}
By definition of \defref{d:indexedsubstitution}, there is 
$\sigma_2 \in \indices{\fn{P_2' \Par P_2''} \cup  \rho'_2 \cup \rho''_2}$ such that 
$\sigma_2 \subseteq \sigma_1 \cdot \nextn{n_i} \cdot \nextn{\dual n_i}$. 
That is, we know 
\begin{align*}
  \Cbs{\rho'_2 \cdot \rho_2''}{\sigma_2}
  {P_2' \Par P_2''} = \Cbs{\rho'_2 \cdot \rho_2''}{\sigma_1 \cdot \nextn{n_i} 
  \cdot \nextn{\dual n_i}}
  {P_2' \Par P_2''}
\end{align*}
% we have that $\sigma_1 \cdot \nextn{n_i} 
% \cdot \nextn{\dual n_i} \in \indices{\fn{P_2' \Par P_2''} \cup \cup \wtd u \cup \wtd x}$. 
Thus, we can conclude 
\begin{align*}
  &{\newsp{\wtd{m_1}}{P'_2 \Par P''_2}\rho_2' \cdot \rho''_2}
  \ \relS 
  {\newsp{\widetilde{m_2}}{Q'_2 \Par Q''_2}}
\end{align*}
This concludes \texttt{Tau} case. 

% \item Case \texttt{News}. 
   
 \end{enumerate}

 \textbf{Recursion cases}
 Now, we consider cases where $P'_1 \equiv \recp{X}P^*_1$ 
 is a parallel component of $P_1$. 
 We focus on cases that highlight specifics of 
 the breakdown of recursive processes 
 and omit details that are similar to the corresponding 
 non-recursive cases. 
 \begin{enumerate}
   \item Case \texttt{Rv}. 
  Here we know $P_1 = \binp{n}{y}P_2$
  such that $P_1\equiv\recp{X}P^*_1$. 
  Let 
  \begin{align*}
  	P^1_1 = \alpha_d.\alpha_{d-1}. \ldots .\alpha_{d-p}.(P_X \Par R)
  \end{align*}
  \noindent where $R$ and $P_X$ are some processes, $P_X$ contains $X$ 
  and $\alpha_d = \abinp{n}{y}$.
   As $P_1$ is a recursive process, 
    we know that there is $\recp{X}P^*$ such that $P^1_1$ is its sub-processes and
    \begin{align*}
    	P_1 \equiv P^1_1\subst{\recp{X}P^*}{X}
    \end{align*} 
%
%    where $\recp{X}P^*$ is subprocess of $P_X$, $\alpha_d = \abinp{n}{y}$, and 
%    $\alpha_d.\alpha_{d-1}. \ldots .\alpha_{d-p}$  and  . 
    Here we can distinguish two sub-cases: \rom{1} $p > 0$ and \rom{2} $p = 0$ and 
    $R \equiv \inact$. 
   We know there is $\rho_2 = \subst{\tilde u_2}{\tilde x_2}$
   such that 
   $$P_1\rho_1 = \binp{n\rho_1}{y}P_2\rho_2$$
  
    The transition is as follows: 
    \begin{align*}
      \AxiomC{} 
      \LeftLabel{\scriptsize $\rulename{Rv}{}$}
      \UnaryInfC{$
      	 P^1_1\subst{\recp{X}P^*}{X}
      	\by{\abinp{n}{v}} 
      	P_2 \rho_2 \cdot \subst{v}{y}
      $}
      \DisplayProof  	
    \end{align*}

	Let $\sigma_1 = \sigma' \cdot \initname{n}{i}$  where 
  $\sigma' \in \indices{\fn{P_1} \cup \wtd u \cup \wtd x}$ 
  and $\sigma_2 = \sigma_1 \cdot \sigma$ where 
  $\sigma = \nextn{n_i} \cdot \initname{y}{1}$.
  Further, let $\wbns u =\bname{\wtd u \sigma_1 : \wtd C}$
  and $\wbns x =\bname{\wtd x \sigma_1 : \wtd C}$ with $\wtd u : \wtd C$. 
  Also, let 
  $\wtd y = (y_1,\ldots,y_{\len{\Gt{S}}})$ and 
  $\wtd z = \fnb{P_2}{\wbns x \wtd y \setminus \wtd w}$ 
  where $\wtd w = \{n_i\}$ if $\lin{n_i}$ otherwise $\wtd w = \epsilon$. 
%    As  $P_1\equiv\recp{X}P^*$ 
%    we know that $P_1 \equiv \alpha_d,\alpha_{d-1},\ldots,\alpha_1.\recp{X}P^*_1 \Par R$ 
%    where $R$ is some process and $\alpha_d,\alpha_{d-1},\ldots,\alpha_1$ is a subprocess 
%    of $P^*_1$ with $\alpha_d = \abinp{n}{y}$.
%    Here we can distinguish two sub-cases: \rom{1} $d > 1$ and \rom{2} $d = 1$. 
%    We consider sub-case \rom{1} first. 
    
     We could see that 
    $d = \rvardepth{\alpha_d,\alpha_{d-1},\ldots,\alpha_1.\recp{X}P^*_1}$. 
    So, by  \tabref{t:tablecd-rec}
    there are following possibilities for the shape of $Q_1$, namely elements in $N$
    defined as: 
    \begin{align*}
    	N = \{\news{\wtd \prop}R : R \in \Cbrecpi{\bns u}{\bns x, \rho}{\recp{X}P^*}^d \}
    \end{align*}
    
    Let 
    \begin{align*}
    	Q^1_1 = \news{\wtd \prop}
    		B_1
    		\Par 
    	 	\binp{n_l}{\wtd y} 
    		\propoutrec{k+1}{\wtd z\rho}
    		\recp{X}\binp{\prop^r_k}{\wtd x}
      		\binp{n_l}{\wtd y} 
      		\propoutrec{k+1}{\wtd z}
      		\rvar{X}
    		 \Par
%      		\\
    	\Brec{k+1}{\tilde z}{\alpha_d,\alpha_{d-1}.P^2_1\sigma}_g
    \end{align*}
    \noindent where $B_1$ is, intuitively, trios mimicking  
    prefixes before $\alpha_d$ and $P^2_1$ is such that 
    $P^1_1 = \alpha_d.\alpha_{d-1}.P^2_1$. 
    By unfolding definition of $\Cbrecpi{\bns u}{\bns x, \rho}{\recp{X}P^*}^d$ 
   	we have that $Q^1_1 \in N$. Further, 
   	if $R \in \Cbrecpi{\bns u}{\bns x, \rho}{\recp{X}P^*}^d$
   	then $R \By{\tau} Q^1_1$. So, we only analyze 
   	how $Q^1_1$ evolves. 
    We can infer the following: 
    \begin{align*}
      Q^1_1 \by{\bactinp{n_i\rho}{\wtd v}} Q_2 
    \end{align*}

    where 
     \begin{align*}
     	Q_2=
    		B_1 
    		\Par
    		\propoutrec{k+1}{\wtd z \rho \cdot \subst{\tilde v}{\tilde y}}
    		\recp{X}\binp{\prop^r_k}{\wtd x}
     		\binp{n_l}{\wtd y} 
     		\propoutrec{k+1}{\wtd z}
     		\rvar{X} \Par \Brec{k+1}{\tilde z}{\alpha_{d-1}.P^2_1\sigma}_g
     \end{align*}
   \noindent  with $v\sigmav \valuesrelate \wtd v$ for some $\sigmav \in \indices{v}$.
    Now, we should show that 
    \begin{align}
      \label{eq:fo-rv-rec-goal1}
      P_2\rho_2 \cdot \subst{v}{y} \relS Q_2 
    \end{align}

	Let $\wtd u_z =\tilde z \rho_2 \cdot \subst{\tilde v}{\tilde y}$. 
	In sub-case \rom{1} we should show that 
	$Q_2 \in \Cbpi{\tilde u_z}{\tilde z}{\alpha_{d-1}.P^2_1}$.
    So, we should show that 
    \begin{align*}
      Q_2 \in  \Cbrecpi{\tilde u_z}
      {\tilde z, \rho_2\cdot \subst{\tilde v}{\tilde y}}{P^*}^{d-1}_g
    \end{align*}
    
    This follows by the inspection of definition 
    $\Dbrecpi{k}{\tilde z, \rho_2 \cdot \subst{\tilde v}{\tilde y}}{P^*}^{d-1}_g$. 
    That is, we can notice that 
    $$Q^1_2 = B_1 \Par B_2$$
    where 
    $B_2 \in \Dbrecpi{k}{\tilde z, \rho_2 \cdot \subst{\tilde v}{\tilde y}}
    {\alpha_{d-1}.P^2_1\sigma}^{d-1}_g$ 
    as $(d-1) + 1= \rvardepth{\alpha_d.\alpha_{d-1}.P^2_1\sigma}$. 
    So, \eqref{eq:fo-rv-rec-goal1} follows. 
    This concludes sub-case \rom{1}. 
    
    In sub-case \rom{2} we know $P_2 \equiv \alpha_{d-1}.P^2_1 \Par R$.  
    Now, by \tabref{t:tablecd-rec} we have $Q_2 \by{\tau} Q^2_2$ where 
    \begin{align*} 
    Q^2_2=& \news{\wtd \prop} 
       V_1 \Par 
   			 \apropoutrecsh{k+\degree+1}{\wtd u_{z_2}}
     		\Par 
         V_2
    \end{align*}

    \noindent where 
    \begin{align*}
      V_1 = & B_1 
      \Par
      \recp{X}\binp{\prop^r_k}{\wtd x}
       \binp{n_l}{\wtd y} 
       \propoutrec{k+1}{\wtd z}
       \rvar{X} \Par 
       \proproutk{r}{k+1}{\wtd u_{z_1}}
      \recp{X}\proprinpk{r}{k}{\wtd x} (\proproutk{r}{k+1}{\wtd z_1}\rvar{X} \Par 
      \apropoutrecsh{k+\degree+1}{\wtd z_2}) \\
      V_2 = & \Brec{k+1}{\tilde z_1}{P_X}_{g_1} \Par 
      \Brec{k+\degree+1}{\tilde z_2}{R}_{\es}
    \end{align*}

    Now, we should show that 
   $Q^2_2 \in \Cbpi{\tilde u_z}{\tilde z}
   {\alpha_{d-1}.P^2_1 \Par R}$.
     By \tabref{t:tablecd-rec} we have that 
    \begin{align}
     \{R_1 \Par R_2 : R_1 \in \Cbrecpi{\tilde u_{z_1}}{\tilde z_1}
     {\alpha_{d-1}.P^2_1},~ R_2 \in \Cbpi{\tilde u_{z_2}}{\tilde z_2}{R}\}
     \subseteq	\Cbpi{\tilde u_{z}}{\tilde z}
    {\alpha_{d-1}.P^2_1 \Par R} 
    \label{eq:fo-rv-rec-r1r2}
    \end{align}
    
    Further, we know that 
     \begin{align}
		  \news{\wtd \prop_{k+l+1}} \apropoutrecsh{k+l+1}{\wtd u_z} 
      \Par \Brec{k+l+1}{\tilde z_2}{R}_\es
		  \in \Cbpi{\tilde u_{z_2}}{\tilde z_2}{R}
      \label{eq:fo-rv-rec-v1}
    \end{align}
    \noindent and 
    \begin{align}
      & V_1 \Par V_2 \in 
        \Cbrecpi{\tilde u_{z_1}}{\tilde z_1}{\alpha_{d-1}.P^2_1}
        \label{eq:fo-rv-rec-v2}
    \end{align}

    Thus, by \eqref{eq:fo-rv-rec-r1r2}, \eqref{eq:fo-rv-rec-v1}, 
    and \eqref{eq:fo-rv-rec-v2} 
    we have the following: 
    \begin{align*}
      V_1 \Par V_2 \Par 
      \news{\wtd \prop_{k+l+1}} \apropoutrecsh{k+l+1}{\wtd u_z} 
      \Par \Brec{k+l+1}{\tilde z_2}{R}_\es
      \in \Cbpi{\tilde u_{z}}{\tilde z}{\alpha_{d-1}.P^2_1 \Par R}
    \end{align*}

    Now, we can notice that 
    $\wtd \prop_{k+l+1} \cap \fpn{V_1} = \es$ and  
    $\wtd \prop_{k+l+1} \cap \fpn{\Brec{k+1}{\tilde z_1}{P_X}_{g_1}} = \es$. 
    Further, we have 
    $$\news{\wtd \prop_{k+l+1}} \Brec{k+\degree+1}{\tilde z_2}{R}_{\es} 
    \fwb \inact$$
    \noindent (where $\fwb$ is defined in Definition 18~\cite{KouzapasPY17}) 
    as first shared trigger $\prop_{k+l+1}$ in the 
    breakdown of $R$ is restricted so it could not get activated. 

    % $$\news{\wtd \prop} 
    % V_1 \Par 
    %    \apropoutrecsh{k+\degree+1}{\wtd u_{z_2}}
    %   \Par 
    %   V_2$$

    Thus, we have  
    $$Q^2_2 \equiv V_1 \Par V_2 \Par 
    \news{\wtd \prop_{k+l+1}} \apropoutrecsh{k+l+1}{\wtd u_z} 
    \Par \Brec{k+l+1}{\tilde z_2}{R}_\es$$
    
    This concludes \texttt{Rv} case. Now, we consider the inductive case. 
 \item Case $\mathtt{Par}_{\mathtt{L}}$. 
      Here we know $P_1 = P'_1 \Par P''_1$. 
      Similarly to the previous case, let 
      \begin{align*}
        P^1_1 = \alpha_d.\alpha_{d-1}. \ldots .\alpha_{d-p}.(P_X \Par R)
      \end{align*}
      We assume $P'_1$ is a recursive process. So, we know 
      there is $\recp{X}P^*$ such that $P^1_1$ is its subprocess 
      and 
      $$P'_1 \equiv P^1_1\subst{\recp{X}P^*}{X}$$

      % Here, we can distinguish sub-cases depending 
      % on if $P''_1 \equiv R$ and $p > 0$ or $p = 0$. 

      Here, we can distinguish two sub-cases: \rom{1} 
      $P''_1 \equiv R$ and \rom{2} $P''_1 \not\equiv R$. 
      Here, we consider sub-case \rom{1} as it is an interesting case. 
      The sub-case \rom{2} is similar to the corresponding 
      case of non-recursive process. 
      As in the previous case, we can further distinguish 
      cases in which $p = 0$ and $p > 0$. 
      We consider $p = 0$ and $\ell = \bactinp{n}{v}$.

      The final rule in the inference tree is as follows: 
      \begin{align*} 
        \AxiomC{$P_1' \subst{\tilde u'_1}{\tilde y_1} \by{\ell} 
        P_2' \subst{\tilde u'_2}{\tilde y_2} 
        \Par 
        R\subst{\tilde w_1}{\tilde z_1}\cdot 
         \subst{\tilde u'_R}{\tilde w_1}$} 
        \AxiomC{$\bn{\ell} \cap \fn{P_1''} = \emptyset$} 
        \LeftLabel{\scriptsize $\rulename{Par}{_L}$}
        \BinaryInfC{$P_1' \subst{\tilde u'_1}{\tilde y_1} \Par 
        R \subst{\tilde u''_1}{\tilde z_1}
        \by{\ell} P_2' \subst{\tilde u'_2}{\tilde y_2} \Par 
        R \subst{\tilde u''_1}{\tilde z_1} \Par
         R\subst{\tilde w_1}{\tilde z_1}\cdot 
         \subst{\tilde u'_R}{\tilde w_1}$} 	
        \DisplayProof 
        \end{align*}

      Let $\sigma_1 \in \indices{\fn{P_1}\cup \wtd u \cup \wtd x}$. 
      Further, let $\wbns y_1 = \fnb{P_1'}{\wbns x}$, 
      $\wbns z_1 = \fnb{R}{\wbns x}$, $\wbns{u} =\bname{\wtd u \sigma_1 : \wtd C}$ 
      where 
        $\wbns{x} =\bname{\wtd x \sigma_1 : \wtd C}$ with $\wtd u : \wtd C$, and 
        $\rhom=\subst{\bns u}{\bns x}$. 
        By the definition of $\relS$
        (\tabref{t:tablecd-rec}), there are following possibilities for $Q_1$:
        \begin{align*}
          Q^1_1 =& \news{\wtd \prop_k}(\apropout{k}{\wbns u} \Par
          \B{k}{\bns x}{P_1  \sigma_1}) \\
          Q^2_1 =& \news{\wtd \prop_k}\propout{k}{\wbns u'_2}
          \apropout{k+\degree}{\wbns u''_1}   \Par
          \B{k}{\bns y_1}{P'_1\sigma_1} \Par 
          \B{k+\degree}{\bns z_1}{R\sigma_1}  \\
          N^3_1 =& \{(R'_1 \Par R''_1) :
          \Cbrecpi{\bns u'_2}{\bns y_1}{\recp{X}P^*\sigma_1}^d_g,~ R''_1 \in 
          \Cbpi{\bns u''_1}{\bns z_1}{R \sigma_1}\}
        \end{align*}

        By \lemref{l:c-prop-closed} there exist
        \begin{align}
          Q'_1 &\in \Cbrecpi{\bns u'_2}{\bns y_1}{\recp{X}P^*\sigma_1}^d_g
        \\
          Q''_1 &\in \Cbpi{\bns u''_1}{\bns z_1}{R\sigma_1}
          \label{eq:fo-parl-rec-q''_1}
        \end{align}
        such that 
      \begin{align*}
        Q^1_1 \By{\tau} Q^2_1 \By{\tau} Q'_1 \Par Q''_1
      \end{align*}

    The interesting case is to consider  a process $Q^3_1$ defined as: 
    \begin{align*} 
      Q^3_1=& \news{\wtd \prop} 
         V_1 \Par 
            \apropoutrecsh{k+\degree+1}{\bns u''_{1}}
           \Par 
           V_2
      \end{align*}
      \noindent where 
      \begin{align*}
        V_1 & =  B_1 
        \Par
         \proproutk{r}{k+1}{\wbns u'_{2}}
        \recp{X}\proprinpk{r}{k}{\wbns y_1} (\proproutk{r}{k+1}{\wbns y_2}\rvar{X} \Par 
        \apropoutrecsh{k+\degree+1}{\wbns z_2}) \\
        V_2 & =  \Brec{k+1}{\bns y_2}{P_X}_{g_1} \Par 
        \Brec{k+\degree+1}{\bns w_2}{R\subst{\tilde w_2}{\tilde z_2}}_{\es}
      \end{align*}

      We have $Q^3_1 \fwb Q'_1 \Par Q''_1$
   ($\fwb$ is defined in Definition 18~\cite{KouzapasPY17}). We may notice that  
    % equivalent to $Q'_1 \Par Q''_1$ which 
    $Q^3_1$ can be a descendent of the recursive process 
    (following the similar  
    reasoning as in the previous case). 
    So, we consider how $Q^3_1$ evolves. As in the corresponding
    case of non-recursive processes, we do the case analysis on $\ell$. 
    % We consider case $\ell = \bactinp{n}{v}$.  
    If $v \in \wtd u$ then we take $\sigmav = \sigma_1$, otherwise $\sigmav =
    \initname{v}{j}$ for  $j > 0$.  
    Now, we could see that 

    $$Q^3_1 \By{\bactinp{n}{\tilde v}} Q_2$$ 

    \noindent where 
    \begin{align*}
      Q_2 =  \news{\wtd \prop} 
      V_1 \Par 
      \proproutk{r}{k+1}{\wbns u'_{2}}
      \recp{X}\proprinpk{r}{k}{\wbns y_1} (\proproutk{r}{k+1}{\wbns y_2}\rvar{X} \Par 
      \apropoutrecsh{k+\degree+1}{\wbns z_1})
        \Par 
        \apropoutrecsh{k+\degree+1}{\wbns u'_{R}}
        \Par 
        V_2
    \end{align*}

    We define $Q^1_2$ as follows
    \begin{align*}
      Q^1_2 &= \news{\wtd \prop} V_1 \Par    
      \proproutk{r}{k+1}{\wbns u'_{2}}
      \recp{X}\proprinpk{r}{k}{\wbns y_1} (\proproutk{r}{k+1}{\wbns y_2}\rvar{X} \Par 
      \apropoutrecsh{k+\degree+1}{\wbns z_1})
      \Par V_2 \Par \\
      & \quad \news{\wtd \prop_{k}} (\apropoutrecsh{k}{\wbns u''_1} 
      \Par \Brec{k}{\bns z_1}{R}_\es) 
     \Par \news{\wtd \prop_{k}} ( \apropoutrecsh{k}{\wbns u'_R} 
      \Par \Brec{k}{\bns w_1}{R\subst{\tilde w_1}{\tilde z_1}}_\es ) 
    \end{align*}

    By definition, we could see that 
    $Q^1_2 \in \Cbpi{\bns u_2}{\bns z_1}{P_2' \Par R \Par R\subst{\tilde w_1}{\tilde z_1}}$.
    Now, 
    by the definition of $\Brec{-}{-}{\cdot}_\es$ we have
    \begin{align*}
      &\apropoutrecsh{k+\degree+1}{\wbns u''_{1}}
      \Par 
      \apropoutrecsh{k+\degree+1}{\wbns u'_{R}}
      \Par 
      \Brec{k+\degree+1}{\bns z_1}{R}_{\es} 
      \fwb \\
      &\news{\wtd \prop_{k}} (\apropoutrecsh{k}{\wbns u''_1} 
      \Par \Brec{k}{\bns z_1}{R}_\es) 
     \Par \news{\wtd \prop_{k}} ( \apropoutrecsh{k}{\wbns u'_R} 
      \Par \Brec{k}{\bns w_1}{R\subst{\tilde w_1}{\tilde z_1}}_\es
    \end{align*}
    % \noindent (where $\fwb$ is defined in Definition 18~\cite{KouzapasPY17}). 
    As each trio in  
    $\Brec{k+\degree+1}{\bns z_1}{R}_{\es}$ makes a replica of itself 
    when triggered along a propagator.  
    % and by assumption we have $\wtd z_1 = \wtd z_2$, 
    % that is $\bns z_1 = \bns z_2$. 
    So, finally we have 
    $$Q_2 \fwb Q^1_2$$

    This concludes the proof. 

 \end{enumerate}

\end{proof}

\begin{restatable}[]{lemm}{lemmsdir}
  \label{l:lemmsdir}
  Assume $P_1 \subst{\tilde u}{\tilde x}$ is a well-formed 
  process and $P_1\subst{\tilde u}{\tilde x} \relS Q_1$.
  \begin{enumerate}
    \item 
				Whenever 
        ${Q_1}{\by{\news{\widetilde{m_2}}\bactout{\iname n}{\wtd v: \Gt{C_1}}}}{Q_2}$
				then there exist
				$P_2$ and $\sigmav$ such that 
        ${P_1\subst{\tilde u}{\tilde x}}{\by{\news{\widetilde{m_1}} \bactout{n}{v:C_1}}}{P_2}$
        where $v\sigmav \valuesrelate \wtd v$
        % where $V_1 \vrelate V_2$
        % and ${P_2}{\ \relS \ }{Q_2}$, 
        and, for a fresh $t$,
        \[
           {\newsp{\wtd{m_1}}{P_2 \parallel \ftrigger{t}{v}{C_1}}}
            \ \relS \ 
          {\newsp{\widetilde{m_2}}{Q_2 \parallel \ftriggerm{t}{v\sigmav}{C_1}}}
        \]

    \item	
      Whenever 
      ${Q_1}{\by{\abinp{\iname n}{\tilde v}}}{Q_2}$
      then there exist $P_2$ and $\sigmav$ such that 
      ${P_1\subst{\tilde u}{\tilde x}}
      {\by{\abinp{n}{v}}}{P_2}$ 
		where $v \sigmav \vrelate \wtd v$
      and
      ${P_2}{\ \relS \ }{Q_2}$, 

      \item	
       Whenever 
       ${Q_1}{\by{\tau}}{Q_2}$
       either \rom{1} ${P_1\subst{\tilde u}{\tilde x}}{\ \relS \ }{Q_2}$ 
       or 
       \rom{2}
        there exists $P_2$ such that 
       ${P_1}{\by{\tau}}{P_2}$ 
				and
        ${P_2}{\ \relS \ }{Q_2}$. 
  \end{enumerate} 
\end{restatable}

% \lemmsdir* 

\begin{proof}[Sketch]
  \label{app:lemmsdir}
  % By transition induction. 
Following Parrow,  we refer to prefixes 
corresponding to prefixes of the original process 
as \emph{essential prefixes}. 
We remark that a prefix in 
$\D{P}$ is non-essential if and only if is a prefix on a propagator name. 
First, we discuss case when transition is inferred without any 
actions from essential prefixes. In this case 
we know that an action can only involve propagator prefixes and  
by inspection of definition of  $\Cbpi{\tilde u}{\tilde x}{P_1}$ that 
$\ell = \tau$. 
 This concerns the sub-case \rom{1} of Part 3
and it directly follows by  \lemref{l:c-prop-closed}. 

  % First, we analyze case of $\tau$ transitions 
  % on propagator prefixes.  This concerns the sub-case \rom{1} of Part 3. 
  % This follows directly by the \lemref{l:c-prop-closed}. 
  Now, assume $Q_1 \by{\ell} Q_2$ when $\ell$ involves essential prefixes. 
  This concerns Part 1, Part 2, and 
  sub-case \rom{2} of Part 3. This case is mainly the inverse of the proof 
  of \lemref{l:lemms}. As Parrow, here we note that 
   an essential prefix is unguarded in $Q_1$ if and only if it is 
   unguarded in $P_1$. That is, by inspection of the definition, 
   function $\Cbpi{\tilde u}{\tilde x}{P_1}$ 
  does not unguard essential prefixes of $P_1$ that its members mimic
  (the propagators serve as guards). 
  % noting that only additional prefixes that 
  % $\Cbpi{\tilde u}{\tilde x}{P_1}$ introduce are propagator prefixes. 
  
\end{proof} 

% \begin{restatable}[]{thm}{mainbsthm}
%   Let $P$ be a \sessp process such that 
%   $\Gamma_1;\Delta_1 \proves P_1$. We have 
%   $$\horelm{\Gamma;\Delta}{P}{\ \mstb \ }
%   {\Gt{\Gamma};\Gt{\Delta}}{\Do{P}}$$ 
% \end{restatable}
\mainbsthm* 

\begin{proof}
  \label{app:mainbsthm}
%   To prove that $\Do{P}$ is MST-bisimilar to $P$ we construct a relation
% $\relS$ that is an MST-bisimulation and  that contains $(P,\Do{P})$; see \defref{d:relation-s}.

% To prove that $\Do{P}$ is MST-bisimilar to $P$
% we construct relation $\mathcal{S}$ (\defref{d:relation-s}) using auxiliary functions
%  $\Cbpi{-}{-}{\cdot}$
% and $\Dbpi{-}{-}{\cdot}$ (\tabref{t:tablecd} and \tabref{t:tablecd-rec}). 
% Then, we prove that $\mathcal{S}$ is a MST bisimulation 
By \lemref{l:lemms} and \lemref{l:lemmsdir} we know $\mathcal{S}$ is a MST bisimulation. 
So, we need to show  $(P,\Do{P}) \in \relS$.
Let $P_1$ be such that $P_1\subst{\tilde r}{\tilde x}=P$
where $\wtd r = \rfn{P}$. Further, let $\sigma = \bigcup_{v \in \tilde r} \subst{v_1}{v}$, 
so we have $\sigma \in \indices{\wtd r}$. Then, let $\wbns r = \bname{\wtd r : \wtd S}$
and $\wbns x = \bname{\wtd x : \wtd S}$ where $\wtd r : \wtd S$. 
Therefore, by \defref{def:decomp}  and \tabref{t:tablecd}  
we have $\Do{P} \in \Cbpi{\bns r}{\bns x}{P_1}$. 
Finally, by \defref{d:relation-s} we have  $(P,\Do{P}) \in \relS$. 

  % The relation $\mathcal{S}$ is a MST bisimulation (\lemref{l:lemms} 
  % and \lemref{l:lemmsdir}) 
  % and $(P, \D{P}) \in \mathcal{S}$.
\end{proof}
